# Supplementary material for: GPU-friendly and Linearly Convergent First-order Methods for Certifying Optimal $k$-sparse GLMs
Source: arXiv:2603.01306 source file (2026-03-01)
Supplement: Supplementary file 1 [file 07_Appendix.tex]

\makeatletter
\clearpage
\appendix
\setcounter{section}{0}%
\setcounter{subsection}{0}%
\setcounter{subsubsection}{0}%
\setcounter{equation}{0}%
\setcounter{figure}{0}%
\setcounter{table}{0}%
\setcounter{theorem}{0}%
\@ifundefined{c@lemma}{}{}%
\@ifundefined{c@corollary}{}{}%
\@ifundefined{c@proposition}{}{}%
\@ifundefined{c@definition}{}{}%
\@ifundefined{c@assumption}{}{}%
\@addtoreset{equation}{section}%
\@addtoreset{figure}{section}%
\@addtoreset{table}{section}%
\@ifundefined{c@lemma}{}{\@addtoreset{lemma}{section}}%
\@ifundefined{c@corollary}{}{\@addtoreset{corollary}{section}}%
\@ifundefined{c@proposition}{}{\@addtoreset{proposition}{section}}%
\@ifundefined{c@definition}{}{\@addtoreset{definition}{section}}%
\@ifundefined{c@assumption}{}{\@addtoreset{assumption}{section}}%

\@ifundefined{c@theorem}{}{}
\@ifundefined{c@lemma}{}{}
\@ifundefined{c@corollary}{}{}
\@ifundefined{c@proposition}{}{}
\@ifundefined{c@definition}{}{}
\@ifundefined{c@assumption}{}{}
\@ifundefined{c@algorithm}{}{}
\@ifundefined{c@algocf}{}{}
\makeatother

\phantomsection
\section*{Appendix}
\addcontentsline{toc}{section}{Appendix}

\addtocontents{toc}{\protect\setcounter{tocdepth}{2}}

\tableofcontents
\clearpage

\section{Additional Algorithm}
\label{ec:additional_algorithm}

A key component of the PAVA algorithm is the ability to merge adjacent blocks and update the solution rapidly.
For the sake of completeness, Algorithm~\ref{alg:up_and_down_block_algorithm_for_merging_in_PAVA} presents the efficient up and down block algorithm used to perform this merging operation in the Algorithm~\ref{alg:prox_of_g_conjugate_root_node}.

\begin{algorithm}[!htb]
    \DontPrintSemicolon
    \caption{Efficient Up and Down Block Algorithm for Lines 5-10 in Algorithm~\ref{alg:prox_of_g_conjugate_root_node}}
    \label{alg:up_and_down_block_algorithm_for_merging_in_PAVA}
    \KwData{vector $\bmu \in \mathbb{R}^p$, nonnegative weights $\brho \in \mathbb{R}_{+}^p$, vector $\hat{\balpha}$ with $\hat{\alpha}_j = \text{prox}_{\rho_j H_M}(\vert{\mu_j})$ for $j \in [p]$, cardinality $k \in \mathbb{N}$, and box constraint $M > 0$.}
    \KwResult{vector $\hat{\balpha}$.}
    
    % \tcp{Initialization for the first block}
    Initialize $b=1$, $P_1 = \rho_1$, $S_1 = \vert{\mu_1}$, $N_b=1$, $\alpha_1$, $r_1 = 1$\;
    $\alpha_{\text{prev}} = \hat{\alpha}_1$, $j=2$\;
    \While{$j \leq p$}{
        $b = b + 1$\;
        $P_b = \rho_j$, $S_b = \vert{\mu_j}$, $N_b=1$, $\alpha = \hat{\alpha}_j$\;
        % \tcp{If the value for the current singleton block is greater that of the previous block (isotonic violation), merge the current block with the previous block}
        \If{$\alpha > \alpha_{\text{prev}}$}{
            $b = b - 1$\;
            $P_b = P_b + \rho_j$, \, $S_b = S_b + \vert{\mu_j}$, \, $N_b = N_b + 1$, \, $\alpha = \text{prox}_{\frac{P_b}{N_b} H_{M}}(\frac{S_b}{N_b})$\;
            % \tcp{Look forward: keep merging the current block with the next block if the isotonic violation persists}
            \While{$j < n$ \textbf{and} $\alpha \leq \hat{\alpha}_j$}{
                $j = j + 1$\;
                $P_b = P_b + \rho_j$, \, $S_b = S_b + \vert{\mu_j}$, \, $N_b = N_b + 1$, \, $\alpha = \text{prox}_{\frac{P_b}{N_b} H_{M}}(\frac{S_b}{N_b})$\;
            }
            % \tcp{Look backward: keep merging the current block with the previous block if the isotonic violation persists}
            \While{$b > 1$ \textbf{and} $\alpha_{b-1} < \alpha$}{
                $b = b - 1$\;
                $P_b = P_b + P_{b+1}$, \, $S_b = S_b + S_{b+1}$, \, $N_b = N_b + N_{b+1}$, \, $\alpha = \text{prox}_{\frac{P_b}{N_b} H_{M}}(\frac{S_b}{N_b})$\;
            }
        }
        % \tcp{Save the current block's value and the index of the last element in the block}
        $\alpha_b = \alpha$, $r_b = j$\;
        % \tcp{Start fresh on the next element}
        $\alpha_{\text{prev}} = \alpha$, $j = j + 1$\;
    }
    % \tcp{Modify the output vector to have the same new value for all elements in each block}
    \For{$l = 1, ..., b$}{
        $\hat{\alpha}_{[r_{l-1}+1:r_l]} = \alpha_l$\;
    }
    \KwRet{$\hat{\bnu}$}\;
\end{algorithm}

\section{Proofs}
\label{ec:proofs}

This section provides complete proofs of the main theoretical results presented in the paper.
For convenience, we restate each result before presenting its proof.

% ==============================================================================
% Part I: Proofs for Section 3 (Methodology)
% ==============================================================================

\subsection{Error Bound for Subgradient Maps of Fenchel Conjugates (Lemma~\ref{lemma:error_bound_for_fenchel_conjugate_of_firmly_convex_function})}
\label{ec_proof:error_bound_for_fenchel_conjugate_of_firmly_convex_function}

\begin{repeatlemma}[Lemma~\ref{lemma:error_bound_for_fenchel_conjugate_of_firmly_convex_function}]
\label{ec_lemma:error_bound_for_fenchel_conjugate_of_firmly_convex_function}
    Let $h$ be a proper, closed, convex function such that there are no lines along which $h$ is finite and affine.
    If $h$ is firmly convex relative to some $\bnu \in \inter(\dom (h^*))$, then for any compact set $\mathcal U \subset \inter(\dom (h^*))$ with $\bnu \in \mathcal U$, there exists a constant $\alpha_{\mathcal U} > 0$ such that
    \begin{align*}
        \dist \left( \partial h^*\left( \bmu \right), \partial h^*\left( \bnu \right)   \right) \leq \frac{2}{\alpha_{\mathcal{U}}} \|\bmu - \bnu \|_2, \quad ~\forall \bmu \in \mathcal{U}.
    \end{align*}
\end{repeatlemma}

% derive the error bound for the Fenchel conjugate of a firmly convex function

\begin{proof}{Proof}
    Since there are no lines along which $h$ is finite and affine, the domain of $h^*$ has nonempty interior \citep[Corollary~13.4.2]{rockafellar1970convex}. 
    Define the tilted function of $h$ relative to $\bnu$ as $h_{\bnu} \left( \bgamma \right) := h\left( \bgamma \right) - \bnu^\top \bgamma$.
    Since $h$ is proper, closed, and convex, its conjugate $h^*$ is also proper, closed, and convex \citep[Theorem~12.2]{rockafellar1970convex}. Moreover, as $\mathcal{U} \subset \inter(\dom(h^*))$, \citep[Theorem~24.7]{rockafellar1970convex} implies that $\partial h^*(\mathcal{U})$ is nonempty and compact.
    Since $h$ is firmly convex relative to $\bnu$, it follows that for the compact set $\partial h^*(\mathcal{U})$ there exists a constant $\alpha_{\mathcal{U}} > 0$ such that, for any $\bgamma \in \partial h^*(\mathcal{U})$, the function $h_{\bnu}$ satisfies the quadratic growth condition
    \[
        h_{\bnu} \left( \bgamma \right) \geq \inf \left( h_{\bnu} \right) + \frac{\alpha_{\mathcal{U}}}{2} \dist^2 \big( \bgamma, ( \partial h_{\bnu} )^{-1} ( \bm{0} ) \big).
    \]
    By \citep[Theorem 3.3]{drusvyatskiy2018error}, the above quadratic growth condition implies the subdifferential error bound inequality
    \begin{align*}
        \dist \big( \bgamma, ( \partial h_{\bnu} )^{-1} \left( \bm{0} \right) \big) \leq \frac{2}{\alpha_{\mathcal{U}}} \dist \left( \bm{0}, \partial h_{\bnu} \left( \bgamma\right) \right).
    \end{align*}
    To simplify the inequality, first observe that the subdifferential of the tilted function satisfies $\partial h_{\bnu} ( \bgamma ) = \partial h ( \bgamma ) - \bnu$, which implies $\dist ( \bm{0}, \partial h_{\bnu} ( \bgamma ) ) = \dist ( \bnu, \partial h ( \bgamma ) )$.
    Second, by~\citep[Corollary 23.5.1]{rockafellar1970convex}, the identity $( \partial h_{\bnu} )^{-1} = \partial h_{\bnu}^*$ holds. Furthermore, since the conjugate of the tilted function satisfies $h_{\bnu}^*(\cdot) = h^*(\cdot+\bnu)$,we have $\left( \partial h_{\bnu} \right)^{-1}(\bm 0) = \partial h_{\bnu}^*(\bm 0) = \partial h^*(\bnu)$. Substituting these two relations into the error bound yields
    \begin{align}
        \label{eq:main:clean}
        \dist \left( \bgamma, \partial h^* \left( \bnu \right) \right) \leq \frac{2}{\alpha_{\mathcal{U}}} \dist \left( \bnu, \partial h \left( \bgamma\right) \right), \quad \forall \bgamma \in \partial h^*(\mathcal{U}).
    \end{align}
    Given some $\bmu \in \mathcal U$, let us pick some $\bbeta \in \partial h^* \left( \bmu \right)$. Then, we have
    \begin{align*}
        \dist \left( \partial h^* \left( \bmu \right), \partial h^* \left( \bnu \right) \right) 
        &\leq \dist \left( \bbeta, \partial h^* \left( \bnu \right) \right) 
        \leq \frac{2}{\alpha_{\mathcal{U}}} \dist ( \bnu, \partial h ( \bbeta ) )
        \leq \frac{2}{\alpha_{\mathcal{U}}} \dist(\bnu, \bmu),
    \end{align*}
    where the first inequality follows from $\bbeta \in \partial h^* \left( \bmu \right)$, the second inequality follows from $\bbeta \in \partial h^*(\mathcal{U})$ and inequality~\ref{eq:main:clean}, and the last inequality holds because $\bbeta \in \partial h^* \left( \bmu \right)$ gives us $\bmu \in \partial h \left( \bbeta \right)$~\citep[Corollary 23.5.1]{rockafellar1970convex}.
    The proof concludes using $\dist \left( \bnu, \bmu \right) = \|\bnu - \bmu \|_2$.
    \hfill \Halmos
\end{proof}

\subsection{Local Quadratic Upper Bound for Fenchel Conjugates (Lemma~\ref{lemma:quadratic_upper_bound_for_fenchel_conjugate_of_firmly_convex_function})}
\label{ec_proof:quadratic_upper_bound_for_fenchel_conjugate_of_firmly_convex_function}

\begin{repeatlemma}[Lemma~\ref{lemma:quadratic_upper_bound_for_fenchel_conjugate_of_firmly_convex_function}]
\label{ec_lemma:quadratic_upper_bound_for_fenchel_conjugate_of_firmly_convex_function}
    Let $h$ be a proper, closed, convex function such that there are no lines along which $h$ is finite and affine.
    If $h$ is firmly convex relative to some $\bnu \in \inter(\dom (h^*))$, then for any compact set $\mathcal U \subset \inter(\dom (h^*))$ with $\bnu \in \mathcal U$, there exists a constant $\alpha_{\mathcal U} > 0$ and a vector $\bs \in \partial h^*(\bnu)$ such that
    \begin{align*}
        h^*(\bmu) \leq h^*(\bnu) + \bs^\top \left( \bmu - \bnu\right) + \frac{\alpha_{\mathcal{U}}}{2} \|\bmu - \bnu\|^2, \quad ~\forall \bmu \in \mathcal{U}.
    \end{align*}
\end{repeatlemma}

% derive the quadratic upper bound for the Fenchel conjugate of a firmly convex function
\begin{proof}{Proof}
    Recall from the proof of Lemma~\ref{lemma:error_bound_for_fenchel_conjugate_of_firmly_convex_function} that $h^*$ is proper, closed, and convex, and that $\dom(h^*)$ is convex with nonempty interior. 
    Since the interior of a convex set is itself convex~\citep[Theorem~6.2]{rockafellar1970convex}, $\inter(\dom(h^*))$ is convex.
    Let $\mathcal K$ denote the convex hull of $\mathcal U$.
    Since $\mathcal U$ is compact and contained in the convex set $\inter(\dom(h^*))$, it follows that $\mathcal K$ is compact \citep[Theorem~17.2]{rockafellar1970convex} and satisfies $\mathcal K \subset \inter(\dom(h^*))$.
    
    Since $\bnu \in \mathcal U$, for any fixed $\bmu \in \mathcal U$, the entire line segment connecting $\bnu$ to $\bmu$ belongs to $\mathcal K$. 
    By the integral form of the mean-value theorem for convex functions~\citep[Theorem 2.3.4]{hiriart2004fundamentals}, we have
    \begin{align*}
        h^*\left( \bmu \right) - h^*\left( \bnu \right) = \int_0^1 \bs_t^\top \left( \bmu - \bnu \right) \mathrm{d}t
    \end{align*}
    for any selection of subgradients $\bs_t \in \partial h^* \left( \bnu + t \left( \bmu - \bnu \right) \right)$. 
    Note that since $h^*$ is proper and convex, it is differentiable almost everywhere in the interior of its domain \citep[Theorem~25.5]{rockafellar1970convex}. Thus, $\bs_t$ is unique for almost all $t \in [0,1]$, ensuring the path is measurable and the integral is well-defined.

    We now construct a companion path $\br_t$ to bound this integral. For each $t \in [0,1]$, let $\br_t := \proj_{\partial h^*(\bnu)}(\bs_t)$ be the projection of $\bs_t$ onto the compact convex set $\partial h^*(\bnu)$. 
    Since the subgradient mapping is bounded on the compact set $\mathcal K$~\citep[Theorem~24.7]{rockafellar1970convex}, $\bs_t$ is bounded.
    Furthermore, because the projection map is continuous and $\bs_t$ is measurable, $\br_t$ is both bounded and measurable. Consequently, the integral $\bs_0 := \int_0^1 \br_{t} \mathrm{d}t$ is well-defined.
    
    Using the mean-value theorem equality, we write:
    \begin{align}
        \label{ineq:mean_value_theorem_integral_form_two_parts}
        h^*\left( \bmu \right) - h^*\left( \bnu \right) 
        =& \int_0^1 \left(\bs_t - \br_{t} + \br_{t} \right)^\top \left(\bmu - \bnu \right) \mathrm{d}t \nonumber \\
        \leq& \left( \int_0^1 \|\bs_t - \br_{t} \|_2 \cdot \| \bmu - \bnu \|_2 \, \mathrm{d}t \right) + \left(\bmu - \bnu \right)^\top \bs_0,
    \end{align}
    where the inequality follows from the Cauchy-Schwarz inequality.
    
    By the definition of the projection, $\|\bs_t - \br_{t}\|_2 = \dist(\bs_t, \partial h^*(\bnu))$. Since $\mathcal K$ is convex and compact, and $\bs_t \in \partial h^*(\bnu + t(\bmu - \bnu))$ with $\bnu + t(\bmu - \bnu) \in \mathcal K$, Lemma~\ref{lemma:error_bound_for_fenchel_conjugate_of_firmly_convex_function} implies that there exists a constant $\alpha_{\mathcal K} > 0$ such that
    \begin{align*}
        \|\bs_t - \br_{t}\|_2 
        = \dist \left( \bs_t, \partial h^* \left( \bnu \right) \right)
        \leq \frac{2}{\alpha_{\mathcal{K}}} \|\bnu + t \left( \bmu - \bnu \right) - \bnu\|_2
        = \frac{2}{\alpha_{\mathcal{K}}} t \|\bmu - \bnu\|_2
    \end{align*}
    for every $t \in [0,1]$.
    Therefore, we can bound the first integral term as follows
    \[
        \int_0^1 \|\bs_t - \br_{t}\|_2 \cdot \| \bmu - \bnu \|_2 \, \mathrm{d}t \leq \int_0^1 \frac{2t}{\alpha_{\mathcal{K}}} \|\bmu - \bnu\|_2^2 \, \mathrm{d}t = \frac{1}{\alpha_{\mathcal{K}}} \|\bmu - \bnu\|_2^2.
    \]

    It remains to show that $\bs_0 \in \partial h^*(\bnu)$.
    For the sake of contradiction, suppose $\bs_0 \notin \partial h^*(\bnu)$.
    Since $\partial h^*(\bnu)$ is non-empty, compact and convex, by the Separating Hyperplane Theorem~\citep[Theorem 11.4]{rockafellar1970convex}, there exists a vector $\ba$ that strictly separates $\bs_0$ from $\partial h^*(\bnu)$, that is,
    \begin{align*}
        \ba^\top \bs_0 > \sup_{\bs \in \partial h^*(\bnu)} \ba^\top \bs.
    \end{align*}
    However, because $\br_{t} \in \partial h^*(\bnu)$ for all $t \in [0, 1]$, we also have $\ba^\top \br_{t} \le \sup_{\bs \in \partial h^*(\bnu)} \ba^\top \bs$.
    Integrating this inequality over $t \in [0, 1]$ yields 
    \[
        \ba^\top \bs_0 = \int_0^1 \ba^\top \br_{t} \mathrm{d}t \le \sup_{\bs \in \partial h^*(\bnu)} \ba^\top \bs,
    \]
    which leads to a contradiction.
    Thus, it must follow that $\bs_0 \in \partial h^*(\bnu)$.
    Plugging these results for the two integral terms back into~\eqref{ineq:mean_value_theorem_integral_form_two_parts}, we have
    \begin{align*}
        h^*\left( \bmu \right) - h^*\left( \bnu \right) &\leq \frac{1}{\alpha_{\mathcal{K}}} \|\bmu - \bnu\|_2^2 + \bs_0^\top \left(\bmu - \bnu \right).
    \end{align*}
    We complete the proof by defining $\alpha_{\mathcal{U}} := \frac{2}{\alpha_{\mathcal{K}}}$ and $\bs := \bs_0$.
    \hfill \Halmos
\end{proof}

\subsection{Primal Quadratic Growth and Dual Quadratic Decay Conditions (Theorem~\ref{theorem:quadratic:conditions})}
\label{ec_proof:quadratic_conditions}

\begin{repeattheorem}[Theorem~\ref{theorem:quadratic:conditions}]
\label{ec_theorem:quadratic_conditions}
    Under Assumptions~\ref{assumption:F:G}--\ref{assumption:quadratic}, let $\bzeta^\star$ denote the unique dual optimal solution.
	    For any compact sets $\mathcal{B} \subset \mathbb{R}^p$ and $\mathcal{Z} \subset \mathbb{R}^n$ satisfying $\bzeta^\star \in \mathcal{Z}$, $-\mathcal{Z} \subset \inter(\dom(F^*))$ and $\bX^\top \mathcal{Z} \subset \inter(\dom(G^*))$, there exist constants $\alpha_{\mathcal{B}}, \kappa_{\mathcal{Z}} > 0$ such that
	    \begin{align*}
		        \Phi(\bbeta) \geq \Phi^\star + \frac{\alpha_{\mathcal{B}}}{2} \dist^2 (\bbeta, \mathcal{B}^\star), \, \forall \bbeta \in \mathcal{B}, \quad \text{and} \quad
		        -\Psi(\bzeta) \leq -\Psi^\star + \frac{\kappa_{\mathcal{Z}}}{2} \|\bzeta - \bzeta^\star\|^2, \, \forall \bzeta \in \mathcal{Z}.
	    \end{align*}
	\end{repeattheorem}

% show that dual objective satisfies quadratic decay condition

\begin{proof}{Proof of Theorem~\ref{theorem:quadratic:conditions}}
    Under Assumptions~\ref{assumption:F:G} and \ref{assumption:standard_fenchel_duality_assumption}, Lemma~\ref{lemma:basic} guarantees the existence and uniqueness of the dual solution $\bzeta^\star$. We divide the proof into two parts.
    
    The first inequality is a direct consequence of the error bound result in \citep{drusvyatskiy2018error}. 
    In particular, the structural requirements of \citep[Corollary~4.3]{drusvyatskiy2018error} are satisfied by Assumption~\ref{assumption:quadratic}\,(ii) and Assumption~\ref{assumption:quadratic}\,(iii).
    Furthermore, Assumption~\ref{assumption:quadratic}\,(i) guarantees that the optimal solution set $\mathcal{B}^\star$ is compact. This compactness ensures that the growth constant $\alpha_{\mathcal{B}}$ is strictly positive and uniform over the compact set $\mathcal{B}$. This concludes the proof of the first claim.

    We next derive the second inequality by applying Lemma~\ref{lemma:quadratic_upper_bound_for_fenchel_conjugate_of_firmly_convex_function} to the dual objective components. 
    First, consider $F^*$. Set $h = F$ and $\bnu = -\bzeta^\star$. Assumption~\ref{assumption:quadratic}\,(iv) ensures $-\bzeta^\star \in \inter(\dom(F^*))$, which satisfies the conditions of Lemma~\ref{lemma:quadratic_upper_bound_for_fenchel_conjugate_of_firmly_convex_function}. Additionally, Assumption~\ref{assumption:quadratic}\,(ii) provides the firm convexity. Thus, there exist $\bs_1 \in \partial F^*(-\bzeta^\star)$ and $\alpha_1 > 0$ such that for all $\bzeta \in \mathcal{Z}$:
    \begin{align}
        \label{eq:F_upper_bound}
        F^*(-\bzeta) \leq F^*(-\bzeta^\star) + \bs_1^\top \left( -\bzeta + \bzeta^\star \right) + \frac{\alpha_1}{2} \| \bzeta - \bzeta^\star \|_2^2.
    \end{align}
    Next, consider $G^*$. Set $h = G$ and $\bnu = \bX^\top \bzeta^\star$. By Assumption~\ref{assumption:quadratic}\,(iv), we have $\bX^\top \bzeta^\star \in \inter(\dom(G^*))$. Applying Lemma~\ref{lemma:quadratic_upper_bound_for_fenchel_conjugate_of_firmly_convex_function} again, there exist $\bs_2 \in \partial G^*(\bX^\top \bzeta^\star)$ and $\alpha_2 > 0$ such that for all $\bzeta \in \mathcal{Z}$:
    \begin{align}
        \label{eq:G_upper_bound}
        G^*(\bX^\top \bzeta) 
        &\leq G^*(\bX^\top \bzeta^\star) + \bs_2^\top \left( \bX^\top \bzeta - \bX^\top \bzeta^\star \right) + \frac{\alpha_2}{2} \| \bX^\top \bzeta - \bX^\top \bzeta^\star \|_2^2 \nonumber \\
        &\leq G^*(\bX^\top \bzeta^\star) + (\bX \bs_2)^\top \left( \bzeta - \bzeta^\star \right) + \frac{\alpha_2 \|\bX\|_2^2}{2} \| \bzeta - \bzeta^\star \|_2^2.
    \end{align}
    Combining \eqref{eq:F_upper_bound} and \eqref{eq:G_upper_bound} with the definition $-\Psi(\bzeta) = F^*(-\bzeta) + G^*(\bX^\top \bzeta)$, we obtain
    \begin{align*}
        -\Psi(\bzeta) \leq -\Psi^\star + \left( -\bs_1 + \bX \bs_2 \right)^\top (\bzeta - \bzeta^\star) + \frac{\alpha_1 + \alpha_2 \|\bX\|_2^2}{2} \|\bzeta - \bzeta^\star\|_2^2.
    \end{align*}
    
    We claim that $-\bs_1 + \bX \bs_2 = \bm{0}$. 
    Let $\bd := -\bs_1 + \bX \bs_2$. Since Assumption~\ref{assumption:standard_fenchel_duality_assumption} guarantees that $\inter(\dom(\Psi))$ is nonempty and $\bzeta^\star$ is an optimal solution, for a sufficiently small step size $t > 0$, the point $\bzeta_t := \bzeta^\star - t \bd$ remains feasible.
    Substituting $\bzeta_t$ into the inequality yields
    \[
        -\Psi(\bzeta_t) \leq -\Psi^\star - t \|\bd\|_2^2 + \mathcal{O}(t^2).
    \]
    If $\bd \neq \bm{0}$, for small enough $t$, we would have $-\Psi(\bzeta_t) < -\Psi^\star$. However, $\Psi^\star$ is the optimal value, so $\Psi \left(\bzeta_t\right) \leq \Psi^\star$, which is a contradiction. Thus, we must have $-\bs_1 + \bX \bs_2 = \bm{0}$.
    Consequently, by setting $\kappa_{\mathcal{Z}} := \alpha_1 + \alpha_2 \|\bX\|_2^2$, we conclude the second claim.
    \hfill \Halmos
\end{proof}

\subsection{Primal-Dual Relations (Theorem~\ref{theorem:primal_dual_relation_dual_sequence_and_function_value})}
\label{ec_proof:primal_dual_relation_dual_sequence_and_function_value}

\begin{repeattheorem}[Theorem~\ref{theorem:primal_dual_relation_dual_sequence_and_function_value}]
\label{ec_theorem:primal_dual_relation_dual_sequence_and_function_value}
    Under Assumptions~\ref{assumption:F:G}--\ref{assumption:loss_function_is_essentially_strictly_convex}, let $\mathcal{B}^\star$ denote the set of primal optimal solutions and
    $\bzeta^\star$ denote the unique dual optimal solution.
    Let $\mathcal{B} \subseteq \dom (G)$ be a compact set such that $\mathcal{B}^\star \subseteq \mathcal{B}$.
    Define the corresponding dual image set $\mathcal{Z} := \{ - \nabla F(\bX \bbeta) \mid \bbeta \in \mathcal{B} \}$, and assume that the interior conditions $-\mathcal{Z} \subset \inter(\dom (F^*))$ and $\bX^\top \mathcal{Z} \subset \inter(\dom (G^*))$ hold.
    Then, there exist constants $\sigma_{\mathcal{B}}, \kappa_{\mathcal{B}} > 0$ such that for any primal vector $\bbeta \in \mathcal{B}$ and its induced dual vector $\bzeta := - \nabla F(\bX \bbeta)$, we have
    \begin{align*}
        \frac{\sigma_{\mathcal{B}}}{2 } \|\bzeta - \bzeta^\star\|_2^2 &\leq \Phi(\bbeta) - \Phi^\star  \quad
        \text{and} \quad
        \Psi(\bzeta^\star) - \Psi(\bzeta) \leq \frac{\kappa_{\mathcal{B}}}{\sigma_{\mathcal{B}}} \big( \Phi(\bbeta) - \Phi^\star \big).
    \end{align*}
\end{repeattheorem}

% show the primal-dual relation between dual variable sequence and function value gap

\begin{proof}{Proof of Theorem~\ref{theorem:primal_dual_relation_dual_sequence_and_function_value}}
    We first establish the first inequality relating the dual distance to the primal gap.
    By definition, $\bzeta = -\nabla F(\bX \bbeta)$. 
    By Assumption~\ref{assumption:loss_function_is_essentially_strictly_convex}, the function $F^*$ is essentially smooth \citep[Theorem~26.3]{rockafellar1970convex}.
    Thus, using the assumption $-\mathcal{Z} \subset \inter(\dom (F^*))$, the function $F^*$ is differentiable at $-\bzeta$. Applying the Fenchel identity \citep[Theorem 23.5]{rockafellar1970convex}, we have
    \[ -\bzeta = \nabla F(\bX \bbeta) \quad \iff \quad \nabla F^*(-\bzeta) = \bX \bbeta. \]
    Since $F$ is locally smooth (Assumption~\ref{assumption:F:G}), its conjugate $F^*$ is locally strongly convex \citep[Theorem 4.1]{goebel2008local}. Specifically, applying the definition of strong convexity on the compact set $-\mathcal{Z}$ to the points $-\bzeta^\star$ and $-\bzeta$, there exists a constant $\sigma_{\mathcal{B}} > 0$ such that
    \[
        F^*(-\bzeta^\star) \geq F^*(-\bzeta) + \nabla F^*(-\bzeta)^\top \left( \bzeta - \bzeta^\star \right) + \frac{\sigma_{\mathcal{B}}}{2} \|\bzeta - \bzeta^\star\|_2^2.
    \]
    Substituting $\nabla F^*(-\bzeta) = \bX \bbeta$ and rearranging terms, we obtain
    \begin{equation}
        \label{eq:strong_convexity_bound}
        \frac{\sigma_{\mathcal{B}}}{2} \|\bzeta - \bzeta^\star\|_2^2 \leq F^*(-\bzeta^\star) - F^*(-\bzeta) - (\bzeta^\star - \bzeta)^\top \bX \bbeta.
    \end{equation}
    Now, consider the primal optimality gap $\Phi(\bbeta) - \Phi^\star$. Using the identities $\Phi(\bbeta) = F(\bX \bbeta) + G(\bbeta)$ and $\Phi^\star = -F^*(-\bzeta^\star) - G^*(\bX^\top \bzeta^\star)$, we have
    \begin{align*}
        \Phi(\bbeta) - \Phi^\star 
        &= F(\bX \bbeta) + F^*(-\bzeta^\star) + G(\bbeta) + G^*(\bX^\top \bzeta^\star) \\
        &= \left[ F^*(-\bzeta^\star) - F^*(-\bzeta) - \bzeta^\top \bX \bbeta \right] + G(\bbeta) + G^*(\bX^\top \bzeta^\star), 
    \end{align*}
    where the equality holds as $\bzeta = -\nabla F(\bX \bbeta)$, so the Fenchel inequality is tight, and we have $F(\bX \bbeta) = -F^*(-\bzeta) - \bzeta^\top \bX \bbeta$. 
    Adding and subtracting $(\bzeta^\star)^\top \bX \bbeta$ to match the form in \eqref{eq:strong_convexity_bound} yields
    \begin{align*}
        \Phi(\bbeta) - \Phi^\star 
        &= \left[ F^*(-\bzeta^\star) - F^*(-\bzeta) - (\bzeta^\star - \bzeta)^\top \bX \bbeta \right] + \left[ G(\bbeta) + G^*(\bX^\top \bzeta^\star) - (\bzeta^\star)^\top \bX \bbeta \right] \\
        &\geq \frac{\sigma_{\mathcal{B}}}{2} \|\bzeta - \bzeta^\star\|_2^2,
    \end{align*}
    where the inequality holds due to \eqref{eq:strong_convexity_bound} and the Fenchel's inequality applied to $G$ and the pair $(\bbeta, \bX^\top \bzeta^\star)$. This proves the first claim.

    For the second inequality, we apply Theorem~\ref{theorem:quadratic:conditions}. Since $\bzeta \in \mathcal{Z}$ and the assumptions of Theorem~\ref{theorem:quadratic:conditions} are satisfied, there exists a constant $\kappa_{\mathcal{B}} > 0$ such that
    \[
        \Psi(\bzeta^\star) - \Psi(\bzeta) \leq \frac{\kappa_{\mathcal{B}}}{2} \|\bzeta - \bzeta^\star\|_2^2.
    \]
    Combining this with the first inequality yields the desired result.
    \hfill \Halmos
\end{proof}

The structural relationship established in Theorem~\ref{theorem:primal_dual_relation_dual_sequence_and_function_value} suggests that the duality gap $\Phi(\bbeta^t) - \Psi(\bzeta^t)$ serves as a robust proxy for the distance to optimality.
We now leverage this property to design a generic restart scheme to achieve linear convergence.

\subsection{Geometric Decay of Duality Gap (Proposition~\ref{prop:duality_gap_sublinear_bound})}
\label{ec_proof:duality_gap_sublinear_bound}

\begin{repeatproposition}[Proposition~\ref{prop:duality_gap_sublinear_bound}]
\label{ec_proposition:duality_gap_sublinear_bound}
    Under Assumptions~\ref{assumption:F:G}--\ref{assumption:sublinear_algorithm}, let $\alpha_{\mathcal{B}}, \sigma_{\mathcal{B}}, \kappa_{\mathcal{B}} > 0$ be the geometric constants derived in Theorem~\ref{theorem:primal_dual_relation_dual_sequence_and_function_value}.
    Then, the primal--dual iterates $\{(\bbeta^t, \bzeta^t)\}_{t \ge 1}$ satisfy the duality gap
    \begin{align*}
        \Phi(\bbeta^t) - \Psi(\bzeta^t) \leq \left( \frac{2 r(t) (1 + \kappa_{\mathcal{B}} / \sigma_{\mathcal{B}})}{\alpha_{\mathcal{B}}} \right) \big( \Phi(\bbeta^0) - \Psi(\bzeta^0) \big).
    \end{align*}
\end{repeatproposition}

% proof of Proposition~\ref{prop:duality_gap_sublinear_bound}

\begin{proof}{Proof of Proposition~\ref{prop:duality_gap_sublinear_bound}}
    From Theorem~\ref{theorem:primal_dual_relation_dual_sequence_and_function_value}, we have the inequality $\Psi(\bzeta^\star) - \Psi(\bzeta^t) \leq \frac{\kappa_{\mathcal{B}}}{\sigma_{\mathcal{B}}} (\Phi(\bbeta^t) - \Phi^\star)$.
    Adding $\Phi(\bbeta^t) - \Phi^\star$ to both sides, since strong duality holds, we bound the total duality gap
    \[
        \Phi(\bbeta^t) - \Psi(\bzeta^t) \leq \left( 1 + \frac{\kappa_{\mathcal{B}}}{\sigma_{\mathcal{B}}} \right) \left( \Phi(\bbeta^t) - \Phi^\star \right).
    \]
    Substituting the algorithmic rate assumption from \eqref{eq:algorithm_rate_assumption} into this inequality yields
    \[
        \Phi(\bbeta^t) - \Psi(\bzeta^t) \leq r(t) \left( 1 + \frac{\kappa_{\mathcal{B}}}{\sigma_{\mathcal{B}}} \right) \dist^2(\bbeta^0, \mathcal{B}^\star)
        \leq \left( \frac{2 r(t) (1 + \kappa_{\mathcal{B}} / \sigma_{\mathcal{B}})}{\alpha_{\mathcal{B}}} \right) (\Phi(\bbeta^0) - \Phi^\star),
    \]
    where the second inequality follows from Theorem~\ref{theorem:quadratic:conditions}. The proof concludes by noting that, by weak duality, we have $\Phi(\bbeta^0) - \Phi^\star \le \Phi(\bbeta^0) - \Psi(\bzeta^0)$.
    \hfill \Halmos
\end{proof}

\subsection{Linear Convergence Under Gap-Based Restart (Theorem~\ref{theorem:restart_linear_convergence})}
\label{ec_proof:restart_linear_convergence}

\begin{repeattheorem}[Theorem~\ref{theorem:restart_linear_convergence}]
\label{ec_theorem:restart_linear_convergence}
    Suppose the conditions of Proposition~\ref{prop:duality_gap_sublinear_bound} hold and $r\left( t \right)$ is monotonically decreasing.
    Let $(\bbeta^{\init}, \bzeta^{\init})$ be the initial primal--dual pair.
    For any target contraction factor $\eta > 1$, define the restart interval $t_{\max}$ as
    \begin{equation*}
        t_{\max} := \left\lceil r^{-1} \left( \frac{ \alpha_{\mathcal{B}} }{ 2 \eta ( 1 + \kappa_{\mathcal{B}} / \sigma_{\mathcal{B}} ) } \right) \right\rceil,
    \end{equation*}
    where $r^{-1}$ is the inverse of the rate function.
    If the algorithm is restarted every $t_{\max}$ iterations (resetting $t=0$ and setting $\bbeta^0$ to the current iterate), the sequence of duality gaps at the restart points converges linearly with
    \begin{align*}
        \Phi(\bbeta^{s \cdot t_{\max}}) - \Psi(\bzeta^{s \cdot t_{\max}}) \leq \eta^{-s} \left( \Phi(\bbeta^{\init}) - \Psi(\bzeta^{\init}) \right).
    \end{align*}
\end{repeattheorem}

% geometric decay of primal-dual gap

\begin{proof}{Proof of Theorem~\ref{theorem:restart_linear_convergence}}
    Consider the first restart epoch, starting at $t=0$ and ending at $t=t_{\max}$. 
    By invoking Proposition~\ref{prop:duality_gap_sublinear_bound}, the duality gap at iteration $t_{\max}$ satisfies
    \begin{align*}
        \Phi(\bbeta^{t_{\max}}) - \Psi(\bzeta^{t_{\max}}) 
        \leq \left[ \frac{2 r(t_{\max}) (1 + \kappa_{\mathcal{B}} / \sigma_{\mathcal{B}})}{\alpha_{\mathcal{B}}} \right] \left( \Phi(\bbeta^{\init}) - \Psi(\bzeta^{\init}) \right).
    \end{align*}
    We now analyze the contraction factor. By the definition of the restart interval $t_{\max}$, we have
    \[
        t_{\max} \geq r^{-1} \left( \frac{ \alpha_{\mathcal{B}} }{ 2 \eta ( 1 + \kappa_{\mathcal{B}} / \sigma_{\mathcal{B}} ) } \right).
    \]
    Since $r(\cdot)$ is a monotonically decreasing function, applying $r$ to both sides reverses the inequality:
    \[
        r(t_{\max}) \leq \frac{ \alpha_{\mathcal{B}} }{ 2 \eta ( 1 + \kappa_{\mathcal{B}} / \sigma_{\mathcal{B}} ) }.
    \]
    Substituting this upper bound for $r(t_{\max})$ back into the duality gap inequality, the geometric constants cancel out and we obtain
    \begin{align*}
        \Phi(\bbeta^{t_{\max}}) - \Psi(\bzeta^{t_{\max}}) 
        &\leq \left[ \frac{2 (1 + \kappa_{\mathcal{B}} / \sigma_{\mathcal{B}})}{\alpha_{\mathcal{B}}} \cdot \frac{ \alpha_{\mathcal{B}} }{ 2 \eta ( 1 + \kappa_{\mathcal{B}} / \sigma_{\mathcal{B}} ) } \right] \left( \Phi(\bbeta^{\init}) - \Psi(\bzeta^{\init}) \right) \\
        &= \eta^{-1} \left( \Phi(\bbeta^{\init}) - \Psi(\bzeta^{\init}) \right).
    \end{align*}
    
    This establishes that the duality gap contracts by a factor of at least $\eta^{-1}$ after one full restart epoch. 
    Since the algorithm is re-initialized at the end of each epoch (setting the new $\bbeta^0$ to the current iterate), this contraction applies recursively. 
    Therefore, after $s$ restarts (spanning $s \cdot t_{\max}$ total iterations), we obtain the bound in the theorem statement. This completes the proof.
    \hfill \Halmos
\end{proof}

\subsection{(Theoretical) Optimal Choice of Restart Parameter (Theorem~\ref{theorem:optimal_restart_eta_choice})}
\label{ec_proof:optimal_restart_eta_choice}

\begin{repeattheorem}[Theorem~\ref{theorem:optimal_restart_eta_choice}]
\label{ec_theorem:optimal_restart_eta_choice}
    Suppose the convergence rate behaves like $r(t) \approx C / t^q$ for some $q > 0$ and $C > 0$.
    Then, the constant-optimal choice of the restart parameter is $\eta = e^q$.
\end{repeattheorem}

\begin{proof}{Proof}
	    Given the tolerance level $\epsilon > 0$ for the primal-dual gap and some restart decrease factor $\eta > 1$, if we ignore the ceiling operation, the number of iterations is approximately
    \[
        T_{\max} \approx \log_\eta \left( \frac{\Phi(\bbeta^{\text{init}}) - \Psi(\bzeta^{\text{init}})}{\epsilon}\right) \cdot r^{-1} \left( \frac{ \alpha_{\mathcal{B}} }{ 2 \eta ( 1 + \kappa_{\mathcal{B}} / \sigma_{\mathcal{B}} ) } \right) 
    \]
    Under the assumption that $r(t) \approx C / t^q$, we have
    \[
        T_{\max} \approx \log_\eta \left( \frac{\Phi(\bbeta^{\text{init}}) - \Psi(\bzeta^{\text{init}})}{\epsilon}\right) \cdot \left( \frac{ 2 C \eta ( 1 + \kappa_{\mathcal{B}} / \sigma_{\mathcal{B}} )  }{ \alpha_{\mathcal{B}} } \right)^{1/q}.
    \]
    Ignoring the terms that do not depend on $\eta$, the iteration complexity is
    \[
        T_{\max} \propto \log_{\eta}\left( \frac{1}{\epsilon} \right)\eta^{1/q} = \log \left( \frac{1}{\epsilon} \right) \frac{\eta^{1/q}}{\log \eta}.
    \]
    Taking the derivative of $\eta^{1/q} / \log \eta$ with respect to $\eta$ and setting it to zero, we have
    \[
        \frac{d}{d\eta} \left( \frac{\eta^{1/q}}{\log \eta} \right)
        = \frac{\eta^{1/q - 1} \left( \frac{1}{q} \log \eta - 1 \right)}{(\log \eta)^2}
        = 0
        \quad \Longleftrightarrow \quad
        \log \eta = q
        \quad \Longleftrightarrow \quad
        \eta = e^q.
    \]
    The second derivative of $\eta^{1/q} / \log \eta$ is
    \[
        \frac{d^2}{d\eta^2} \left( \frac{\eta^{1/q}}{\log \eta} \right)
        = \frac{\eta^{1/q - 2}}{(\log \eta)^3}\left( \frac{1-q}{q^2}(\log \eta)^2 + \frac{q-2}{q}\log \eta + 2 \right), \qquad (\eta>1,\ q>0).
    \]
    Evaluating at $\eta = e^q$ (so that $\log \eta = q$), we obtain
    \[
        \left.\frac{d^2}{d\eta^2} \left( \frac{\eta^{1/q}}{\log \eta} \right)\right|_{\eta=e^q}
        = \frac{(e^q)^{1/q - 2}}{q^3}\left( \frac{1-q}{q^2}q^2 + \frac{q-2}{q}q + 2 \right)
        = \frac{e^{1-2q}}{q^3} > 0.
    \]
    Therefore, $\eta=e^q$ yields a local minimum of $\eta^{1/q}/\log\eta$ and is the only one, so it is the global minimum for $\eta>1$ and the optimal choice for the restart decrease factor.
    \hfill \Halmos
\end{proof}

% ==============================================================================
% Part II: Proofs for Section 4 (Efficient Implementation for Sparse GLMs)
% ==============================================================================

\subsection{Convex Analysis Properties at a BnB Node (Lemma~\ref{lemma:g_is_proper_closed_and_convex})}
\label{ec_proof:g_is_proper_closed_and_convex}

\begin{repeatlemma}[Lemma~\ref{lemma:g_is_proper_closed_and_convex}]
\label{ec_lemma:g_is_proper_closed_and_convex}
    The implicit function $g_{\mathcal{N}}$ in~\eqref{eq:function_g_definition} is proper, closed and convex, with a compact domain.
\end{repeatlemma}

% g is proper, closed and convex
\begin{proof}{Proof}
    Define the function $H: \mathbb{R}^p \times \mathbb{R}^p \to \overline{\mathbb{R}}$ as 
    \[
        H(\bbeta, \bz) = \frac{1}{2} \sum_{j \in [p]} \beta_j^2/z_j + \delta_{\mathcal{D}} ( \bbeta, \bz ).
    \]
    First, observe that each term $\beta_j^2 / z_j$ is the perspective of a convex quadratic function and is therefore proper, closed, and convex~\citep[Lemma~1 \& 2]{shafiee2024constrained}.
    Second, since the domain $\mathcal{D}$ is a nonempty bounded polyhedron, the indicator function $\delta_{\mathcal{D}}$ is also proper, closed, and convex.
    Consequently, as $H$ is the sum of proper, closed, and convex functions, it retains these properties~\citep[Theorem 9.3]{rockafellar1970convex}.

    The function $g_{\mathcal{N}}$ is defined as the partial minimization of $H$ with respect to $\bz$.
    Since the domain $\mathcal{D}$ is bounded, the domain of the recession function of $H$ consists solely of the zero vector. 
    Thus, the recession condition of~\citet[Theorem 9.2]{rockafellar1970convex} is satisfied, implying that $g_{\mathcal{N}}$ is proper, closed, and convex.
    Finally, the domain of $g_{\mathcal{N}}$ corresponds to the projection of the compact set $\mathcal{D}$ onto the $\bbeta$-coordinates. Since the projection is a linear map and $\mathcal{D}$ is compact polyhedron, $\dom(g_{\mathcal{N}})$ is a compact polyhedron~\citep[Theorem 19.3]{rockafellar1970convex}.
    \hfill \Halmos
\end{proof}

\subsection{Fenchel-Conjugate Representation at a BnB Node (Lemma~\ref{lemma:function_g_conjugate_in_BnB})}
\label{ec_proof:function_g_conjugate_in_BnB}

\begin{repeatlemma}[Lemma~\ref{lemma:function_g_conjugate_in_BnB}]
\label{ec_lemma:function_g_conjugate_in_BnB}
    The Fenchel conjugate of $g_{\mathcal{N}}$ is given by
    \begin{align*}
        g_{\mathcal{N}}^* \left( \balpha \right) =
            \sum_{j \in \mathcal{J}_1} H_M(\alpha_j) \, + \textstyle
            \TopSum_{k - | \mathcal J_1|} \big( \bm{H}_M \big( \balpha_{\calJ_f} \big) \big).
    \end{align*}
\end{repeatlemma}

% derive the conjugate function of $g_{\mathcal{N}}$

\begin{proof}{Proof of Lemma~\ref{lemma:function_g_conjugate_in_BnB}}
    Recall that the Huber loss function admits the variational form 
    \[ H_M(\alpha) = \sup_{\beta \in \mathbb R} \left\{ \alpha \beta - \beta^2 / 2 \ : \ |\beta| \leq M \right\}. \]
    By the definition of the Fenchel conjugate, we have
    \begin{align*}
        g_{\mathcal{N}}^* \left( \balpha \right) = \sup_{\left( \bbeta, \bz \right) \in \mathcal{D}} ~ \balpha^\top \bbeta - \frac{1}{2} \sum_{j \in [p]} \frac{\beta_j^2}{z_j} .
    \end{align*}
    Using the definition of the domain $\mathcal D$, we can decompose the supremum over the partition $\mathcal{J}_0, \mathcal{J}_1, \mathcal{J}_f$.
    \begin{align*}
        g_{\mathcal{N}}^* \left( \balpha \right) 
        =& \sup \left\{ \sum_{j \in \mathcal J_0}  \alpha_j \beta_j - \frac{\beta_j^2}{2z_j}  \ : \ z_j = \beta_j = 0, \ \forall j \in \mathcal J_0 \right\} \\
        &+ \sup \left\{ \sum_{j \in \mathcal J_1}  \alpha_j \beta_j - \frac{\beta_j^2}{2z_j} \ : \ z_j = 1, |\beta_j| \leq M, \ \forall j \in \mathcal J_1 \right\} \\
        &+ \sup \left\{ \sum_{j \in \mathcal J_f}  \alpha_j \beta_j - \frac{\beta_j^2}{2z_j} \ : \ \sum_{j \in \mathcal J_f} z_j \leq k - |\mathcal J_1|, \ z_j \in [0,1], \ |\beta_j| \leq M z_j, \ \forall j \in \mathcal J_f \right\}.
    \end{align*}
    The first term trivially amounts to zero. 
    By the variational form of the Huber loss, the second term sums to $\sum_{j \in \mathcal J_1} H_M(\alpha_j)$. 
    For the third term, optimizing over $\beta_j$ for a fixed $z_j$ yields
    \begin{align*}
        \sup_{|\beta_j| \leq M z_j} \left\{ \alpha_j \beta_j - \frac{\beta_j^2}{2z_j} \right\} 
        = z_j \sup_{|\beta_j/z_j| \leq M} \left\{ \alpha_j \frac{\beta_j}{z_j} - \frac{1}{2} \left(\frac{\beta_j}{z_j}\right)^2 \right\} 
        = z_j H_M(\alpha_j).
    \end{align*}
    Substituting this back, the third supremum becomes the following linear program over $\bz_{\mathcal{J}_f}$
    \begin{align}
        \label{eq:LP:rep}
        &\sup \left\{  \sum_{j \in \mathcal{J}_f} z_j H_M(\alpha_j)  :  \sum_{j \in \mathcal{J}_f} z_j \leq k - \lvert \mathcal{J}_1 \rvert, \ z_j \in [0, 1], \forall j \in \mathcal{J}_f \right\} 
        = \textstyle \TopSum_{k - \lvert \mathcal{J}_1 \rvert} \big( \bm{H}_M \big( \balpha_{\mathcal{J}_f} \big) \big),
    \end{align}
    where the last equality follows from the fact that the optimal strategy is to assign $z_j=1$ to the indices corresponding to the largest values of the non-negative weights $H_M(\alpha_j)$.
    Summing the three parts completes the proof.
    \hfill \Halmos
\end{proof}

\subsection{PLQ and Firm-Convex Structure at a BnB Node (Lemma~\ref{lemma:g_and_g_Fenchel_are_PLQ_and_firmly_convex})}
\label{ec_proof:g_and_g_Fenchel_are_PLQ_and_firmly_convex}

\begin{repeatlemma}[Lemma~\ref{lemma:g_and_g_Fenchel_are_PLQ_and_firmly_convex}]
\label{ec_lemma:g_and_g_Fenchel_are_PLQ_and_firmly_convex}
    The functions $g_{\mathcal{N}}$ and $g_{\mathcal{N}}^*$ are both PLQ and firmly convex.
\end{repeatlemma}

% show that g and g^* are PLQ and firmly convex

\begin{proof}{Proof}
    We first show that $g_{\mathcal{N}}^*$ is PLQ.
    Recall that $g_{\mathcal{N}}^* ( \balpha ) = h_1 ( \balpha ) + h_2 ( \balpha )$, with $h_1 ( \balpha ) := \sum_{j \in \mathcal{J}_1} H_M(\alpha_j)$ and $h_2 ( \balpha ) := \TopSum_{\bar{k}} \big( \bm{H}_M ( \balpha_{\mathcal{J}_f} ) \big)$.
    The Huber function $H_M$ is PLQ by definition. Since the class of convex PLQ functions is closed under addition~\citep[Exercise~10.22]{rockafellar2009variational}, $h_1$ is PLQ.
    For the second term, let $\bar p = |\mathcal J_f|$ and $\bar k = k - |\mathcal{J}_1|$. We partition the subspace $\mathbb{R}^{\bar{p}}$ associated with $\balpha_{\mathcal{J}_f}$ into $\binom{\bar{p}}{\bar{k}}$ sorting regions indexed by $l$
    \begin{align*}
        \mathcal{D}_l := \left\{ \balpha \in \mathbb{R}^p \mid \lvert \alpha_i \rvert \geq \lvert \alpha_j \rvert, \ \forall i \in \mathcal{I}_l, \, \forall j \in \mathcal{J}_f \setminus \mathcal{I}_l \right\}.
    \end{align*}
    Within each region $\mathcal{D}_l$, the $\TopSum$ operator fixes its selection to the set $\mathcal{I}_l$.
    We further subdivide each $\mathcal{D}_l$ based on the thresholds of the Huber function. Define the intervals:
    \[
        I_1 := (M, +\infty), \quad I_2 := [0, M], \quad I_3 := [-M, 0), \quad I_4 := (-\infty, -M].
    \]
    We partition $\mathcal{D}_l$ into $4^{\bar{p}}$ polyhedral cells $\mathcal{D}_{l,\bm m}$, indexed by a vector $\bm m \in \{1, 2, 3, 4\}^{\bar{p}}$, such that for each $j \in \mathcal{J}_f$, $\alpha_j \in I_{m_j}$.
    The union of these sets satisfies $\bigcup_{l} \bigcup_{\bm m} \mathcal{D}_{l,\bm m} = \mathbb{R}^p = \dom(g^*_{\mathcal N}) $.
    
    On any specific cell $\mathcal{D}_{l,\bm m}$, the function $h_2$ reduces to a fixed sum of Huber terms over the set~$\mathcal{I}_l$. Specifically, depending on whether the interval index $m_j$ corresponds to the quadratic region ($| \alpha_j | \le M$) or the linear region ($| \alpha_j | > M$), the function takes the form:
    \begin{align*}
        h_2(\balpha) = \sum_{j \in \mathcal{I}_l \cap \mathcal{Q}_{\bm m}} \frac{1}{2} \alpha_j^2 + \sum_{j \in \mathcal{I}_l \cap \mathcal{L}_{\bm m}} \left( M |\alpha_j| - \frac{1}{2}M^2 \right),
    \end{align*}
    where $\mathcal{Q}_{\bm m}$ and $\mathcal{L}_{\bm m}$ are the sets of indices mapped to quadratic and linear intervals, respectively. 
    Since this expression consists purely of linear and quadratic terms, $h_2$ is PLQ. As the sum of PLQ functions is PLQ \citep[Exercise~10.22]{rockafellar2009variational}, $g_{\mathcal{N}}^*$ is PLQ.

    We next prove that $g_{\mathcal{N}}$ is PLQ. By Lemma~\ref{lemma:g_is_proper_closed_and_convex}, $g_{\mathcal{N}}$ is proper, closed, and convex, and hence $g_{\mathcal{N}}^*$ is proper, closed, and convex with $g_{\mathcal{N}} = (g_{\mathcal{N}}^*)^*$ \citep[Theorem~12.2]{rockafellar1970convex}. Since the Fenchel conjugate of a proper, closed, and convex PLQ function is also PLQ \citep[Theorem 11.14(b)]{rockafellar2009variational}, it follows that $g_{\mathcal{N}}$ is PLQ.

    Finally, we establish the firm convexity of $g_{\mathcal{N}}$ and $g_{\mathcal{N}}^*$.
    Since both functions are convex PLQ, their tilted counterparts, defined as $h_{\bnu}(\cdot) := h(\cdot) - \bnu^\top (\cdot)$, remain trivially convex PLQ for any vector $\bnu \in \mathbb{R}^p$.
    It is well-established that proper, closed, and convex PLQ functions satisfy the quadratic growth condition on any compact set~\citep[Theorem~2.7]{li1995error}.
    Consequently, both $g_{\mathcal{N}}$ and $g_{\mathcal{N}}^*$ satisfy the definition of firm convexity relative to any vector $\bnu$. This completes the proof.
    \hfill \Halmos
\end{proof}

\subsection{Correctness of the Compute-g-Value Algorithm (Theorem~\ref{theorem:compute_g_value_algorithm_correctness})}
\label{ec_proof:compute_g_value_algorithm_correctness}

\begin{repeattheorem}[Theorem~\ref{theorem:compute_g_value_algorithm_correctness}]
\label{ec_theorem:compute_g_value_algorithm_correctness}
    For any $\bbeta \in \dom (g_{\mathcal{N}})$, let $\bar \bbeta := \bbeta_{\mathcal{J}_f}$, $\bar p := \lvert \mathcal{J}_f \rvert$, and $\bar k := k - \lvert \mathcal{J}_1 \rvert$.
    Then
    \begin{align*}
        g_{\mathcal{N}}(\bbeta)
        &= \frac{1}{2} \sum_{j \in \mathcal{J}_1}\beta_j^2 + \frac{1}{2}\min_{\bomega} \left\{ \sum_{j=1}^{\bar k} \omega_j^2 \ \middle|\ 
        \begin{array}{l}
            \bomega \ge \bm{0}, \quad M \ge \omega_1 \ge \cdots \ge \omega_{\bar k} \ge 0, \\
            \omega_{\bar k+1} = \cdots = \omega_{\bar p} = 0, \quad \bomega \succeq_m |\bar{\bbeta}|
        \end{array}
        \right\}.
    \end{align*}
    Here, $\bomega \succeq_m |\bar{\bbeta}|$ denotes that $\bomega$ majorizes $|\bar{\bbeta}|$, \textit{i.e.},
    \[
        \sum_{j=1}^{\ell} \omega_j \ge \sum_{j=1}^{\ell} |\bar\beta_{(j)}| \quad \forall \ell = 1,\ldots,\bar p-1,
        \qquad \text{and} \qquad
        \sum_{j=1}^{\bar p} \omega_j = \sum_{j=1}^{\bar p} |\bar\beta_{(j)}|.
    \]
    Algorithm~\ref{alg:compute_g_value_root_node_algorithm} computes a minimizer $\bomega$ of the above problem and thus evaluates $g_{\mathcal{N}}(\bbeta)$ exactly with a computational complexity of $\mathcal O(p + \bar p \log \bar k + \bar k)$.
\end{repeattheorem}

% show that our algorithm computes g value exactly

\begin{proof}{Proof of Theorem~\ref{theorem:compute_g_value_algorithm_correctness}}
    We first simplify the evaluation of $g_{\mathcal{N}}(\bbeta)$ by decomposing the problem based on the partition $\mathcal{J}_0, \mathcal{J}_1, \mathcal{J}_f$ defined by node $\mathcal{N}$.
    Using the definitions of the domain $\mathcal{D}$ and the function $g_{\mathcal{N}}$, the optimization problem in~\eqref{eq:function_g_definition} separates as follows
    \begin{align*}
        g_{\mathcal{N}}(\bbeta)
        &= \frac{1}{2} \sum_{j \in \mathcal{J}_0} \frac{\beta_j^2}{0}
        + \frac{1}{2} \sum_{j \in \mathcal{J}_1} \beta_j^2 %\\
        % &\quad 
        + \frac{1}{2} \min_{\bz_{\mathcal{J}_f} \in \mathbb R^{\bar p}} \left\{ \sum_{j \in \mathcal{J}_f} \frac{\beta_j^2}{z_j} \ : \
        \begin{array}{l}
            z_j \in [0, 1], \ \forall j \in \mathcal J_f, \\
            \lvert \beta_j \rvert \leq M z_j, \ \forall j \in \mathcal J_f, \\
            \sum_{j \in \mathcal{J}_f} z_j \leq \bar{k},
        \end{array}
        \right\},
    \end{align*}
    where $\bar{k} := k - |\mathcal{J}_1|$ and $\bar p := |\mathcal{J}_f|$.
    Note that the first term is finite if and only if $\beta_j=0$ for all $j\in\mathcal{J}_0$ (in which case it is zero).
    The second term is constant given $\bbeta$.
    Therefore, the core difficulty lies in the third term. For notational simplicity, we reformulate the third term (ignoring $\frac{1}{2}$) as
    \begin{align}
        \label{eq:reduced_problem}
        \min_{\bar \bz \in \mathbb R^{\bar p}} \left\{ \sum_{j \in [\bar p]} \frac{\bar \beta_j^2}{\bar z_j} \ : \
        \begin{array}{l}
            \bar \bz \in [0, 1]^{\bar p}, \quad \1^\top \bar \bz \leq \bar{k}, \\
            \lvert \bar\beta_j \rvert \leq M \bar z_j, \ \forall j \in [\bar p],
        \end{array}
        \right\},
    \end{align}
    where $\bar {\bbeta} := \bbeta_{\mathcal{J}_f}$ and $\bar {\bz} := \bz_{\mathcal{J}_f}$.
    Since the objective and constraints depend on $\bar{\bbeta}$ only through the magnitudes $|\bar\beta_j|$ and are permutation-invariant, we sort the magnitudes of the free variables such that
    $|\bar{\beta}_{(1)}| \geq |\bar{\beta}_{(2)}| \geq \dots \geq |\bar{\beta}_{(\bar{p})}|$.
    This expression is equivalent to the variational characterization of half the squared $\bar k$-support norm \citep{argyriou2012sparse, kim2022convexification}.

    We now avoid working directly with $\bar\bz$ and instead derive an evaluation procedure solely based on $\bar\bbeta$ through a majorization-based convex-hull representation.
    Consider the following three sets:
    \begin{itemize}
        \item $\mathcal{S}_1 := \left\{ \left( t, \bar{\bbeta} \right)  \,\middle|\,  \|\bar{\bbeta}\|_2^2 \leq t, \, \|\bar{\bbeta}\|_{\infty} \leq M, \, \|\bar{\bbeta}\|_0 \leq \bar{k} \right\},$
        \item $\mathcal{S}_2 := \left\{ \left( t, \bar{\bbeta} \right)  \,\middle|\, \exists \bar\bz \in [0, 1]^{\bar p} \ \st \ \sum_{j \in [\bar p]} \bar\beta_j^2 / \bar z_j \leq t, \ \1^\top \bar\bz \leq \bar{k}, \ \lvert \bar\beta_j \rvert \leq M \bar z_j \ \forall j \in [\bar p] \right\},$
        \item $\mathcal{S}_3 := \left\{ \left( t, \bar{\bbeta} \right)  \,\middle|\, \exists \bomega \in \mathbb{R}^{\bar p} \ \st \
        \begin{array}{l}
            \bomega \ge \bm{0}, \quad \sum_{j \in [\bar p]} \omega_j^2 \leq t, \quad M \ge \omega_1 \ge \cdots \ge \omega_{\bar k} \ge 0, \\
            \omega_{\bar k+1} = \cdots = \omega_{\bar p} = 0, \quad \bomega \succeq_m |\bar{\bbeta}|
        \end{array}
        \right\},$
    \end{itemize}
    where $|\bar{\bbeta}|$ denotes the elementwise absolute value, and $\bomega \succeq_m |\bar{\bbeta}|$ denotes that $\bomega$ majorizes $|\bar{\bbeta}|$, \textit{i.e.},
    \[
        \sum_{j=1}^{\ell} \omega_j \ge \sum_{j=1}^{\ell} |\bar\beta_{(j)}| \quad \forall \ell = 1,\ldots,\bar p-1,
        \qquad \text{and} \qquad
        \sum_{j=1}^{\bar p} \omega_j = \sum_{j=1}^{\bar p} |\bar\beta_{(j)}|.
    \]

    If $\mathcal{S}_2$ had binary constraints $\bar\bz \in \{0,1\}^{\bar p}$, then it would coincide with $\mathcal{S}_1$. Relaxing $\bar z_j \in \{0,1\}$ to $\bar z_j \in [0,1]$ yields the (closed) convex hull, so $\mathcal{S}_2$ is the closed convex hull of $\mathcal{S}_1$~\citep{shafiee2024constrained}.
    Moreover, since $\mathcal{S}_1$ is sign- and permutation-invariant, \citet[Theorem~4]{kim2022convexification} show that $\mathcal{S}_3$ is also the closed convex hull of $\mathcal{S}_1$.
    Therefore, $\mathcal{S}_2 = \mathcal{S}_3$, and the optimal value of~\eqref{eq:reduced_problem} can be written as
    \begin{align}
        \min \left\{ t \,\middle|\, \left( t, \bar{\bbeta} \right) \in \mathcal{S}_2 \right\}
        &= \min \left\{ t \,\middle|\, \left( t, \bar{\bbeta} \right) \in \mathcal{S}_3 \right\} \nonumber \\
        &= \min_{\bomega} \left\{ \sum_{j=1}^{\bar k} \omega_j^2 \ \middle|\ 
        \begin{array}{l}
            \bomega \ge \bm{0}, \quad M \ge \omega_1 \ge \cdots \ge \omega_{\bar k} \ge 0, \\
            \omega_{\bar k+1} = \cdots = \omega_{\bar p} = 0, \quad \bomega \succeq_m |\bar{\bbeta}|
        \end{array}
        \right\}
        \label{eq:reduced_problem_majorization_form}.
    \end{align}

    We next show that Algorithm~\ref{alg:compute_g_value_root_node_algorithm} constructs the minimizer in~\eqref{eq:reduced_problem_majorization_form}.
    Let $\theta := \sum_{j=1}^{\bar p} |\bar\beta_{(j)}|$ denote the total sum.
    Since $\bomega \succeq_m |\bar{\bbeta}|$, we must have $\omega_1 \ge |\bar\beta_{(1)}|$. In addition, the equality of total sums and the ordering $\omega_1 \ge \cdots \ge \omega_{\bar k}$ imply $\bar k\,\omega_1 \ge \sum_{j=1}^{\bar k} \omega_j = \theta$, hence $\omega_1 \ge \theta/\bar k$.
    Therefore, $\omega_1 \ge \max\left(|\bar\beta_{(1)}|, \theta/\bar k \right)$.
    If $\theta/\bar k \ge |\bar\beta_{(1)}|$, the choice $\omega_1 = \cdots = \omega_{\bar k} = \theta/\bar k$ minimizes $\sum_{j=1}^{\bar k} \omega_j^2$ among all vectors with fixed sum $\theta$ (by convexity of $x \mapsto x^2$).
    Otherwise, the minimizer must satisfy $\omega_1 = |\bar\beta_{(1)}|$, and we repeat the same argument on the remaining coordinates with updated remaining sum $\theta \gets \theta - |\bar\beta_{(1)}|$.
    This yields the iterative ``peeling'' rule implemented in Algorithm~\ref{alg:compute_g_value_root_node_algorithm}:
    in iteration $j$, compute the candidate average $\overline{\theta} := \theta / (\bar k - j + 1)$; if $\overline{\theta} \ge |\bar\beta_{(j)}|$ then set $\omega_j = \cdots = \omega_{\bar k} = \overline{\theta}$ and stop; otherwise set $\omega_j = |\bar\beta_{(j)}|$ and update $\theta \gets \theta - |\bar\beta_{(j)}|$.
    The returned objective value equals the optimal value of~\eqref{eq:reduced_problem_majorization_form}, and hence of~\eqref{eq:reduced_problem}.

    Finally, the construction above also yields the familiar closed-form expression as in~\citet[Proposition~6]{kim2022convexification}.
    Let $\kappa \in \{0,\ldots,\bar k-1\}$ denote the number of ``peeled'' coordinates, i.e., the number of indices for which the algorithm sets $\omega_j = |\bar\beta_{(j)}|$.
    Then $\omega_1 = |\bar\beta_{(1)}|,\ldots,\omega_{\kappa} = |\bar\beta_{(\kappa)}|$ and $\omega_{\kappa+1} = \cdots = \omega_{\bar k} = \frac{1}{\bar k - \kappa} \sum_{j=\kappa+1}^{\bar p} |\bar\beta_{(j)}|$.
    Substituting into~\eqref{eq:reduced_problem_majorization_form} gives
    \begin{equation*}
        \sum_{j=1}^{\kappa} \bar{\beta}_{(j)}^2 + \frac{1}{\bar{k}-\kappa} \left( \sum_{j=\kappa+1}^{\bar{p}} |\bar{\beta}_{(j)}| \right)^2,
    \end{equation*}
    where $\kappa$ is the unique integer satisfying
    \[
        |\bar{\beta}_{(\kappa)}| > \frac{1}{\bar{k}-\kappa} \sum_{j=\kappa+1}^{\bar{p}} |\bar{\beta}_{(j)}| \geq |\bar{\beta}_{(\kappa+1)}|.
    \]
    In the original $\bar\bz$-formulation~\eqref{eq:reduced_problem}, the same splitting index $\kappa$ corresponds to the number of coordinates for which the constraint $\bar z_j \le 1$ is active ($\bar z_{(j)}^\star = 1$), while for $j>\kappa$ the remaining budget is distributed proportionally as $\bar z_{(j)}^\star \propto |\bar\beta_{(j)}|$.

    The computational cost of the algorithm is dominated by operations on the free variables $\mathcal{J}_f$. Extracting $\bar{\bbeta}$ takes $\mathcal{O}(\bar{p})$ time. The sorting step typically requires $\mathcal{O}(\bar{p} \log \bar{p})$; however, since the optimal solution effectively depends only on the top $\bar{k}$ components and the residual sum, this can be optimized to $\mathcal{O}(\bar{p} \log \bar{k})$ using a partial sort. The subsequent linear scan to determine $\kappa$ and the final summation perform at most $\mathcal{O}(\bar{k})$ operations. Including the $\mathcal{O}(p)$ time to handle the fixed indices, the total complexity is $\mathcal{O}(p + \bar{p} \log \bar{k} + \bar{k})$. This completes the proof.
    \hfill \Halmos
\end{proof}

\subsection{Correctness of the Evaluate-Prox Algorithm (Theorem~\ref{theorem:evaluate_prox_g_algorithm_correctness})}
\label{ec_proof:evaluate_prox_g_algorithm_correctness}

\begin{repeattheorem}[Theorem~\ref{theorem:evaluate_prox_g_algorithm_correctness}]
\label{ec_theorem:evaluate_prox_g_algorithm_correctness}
    For any $\bbeta \in \mathbb{R}^p$ and $\rho > 0$, Algorithm~\ref{alg:prox_of_g_conjugate_root_node} computes $\prox_{\rho g^*_{\mathcal{N}}} ( \bbeta ) $ exactly with a computational complexity of $\mathcal{O}(p + \bar p \log \bar p)$, where $\bar p = \lvert \mathcal{J}_f \rvert$ and $\bar k = k - \lvert \mathcal{J}_1 \rvert$. Moreover, Algorithm~\ref{alg:prox_of_g_conjugate_root_node} can be used as a subroutine to compute $\prox_{\rho g_{\mathcal{N}}}(\bbeta)$ exactly via the extended Moreau decomposition
    \begin{align*}
        \prox_{\rho g_{\mathcal{N}}} ( \bbeta) = \bbeta - \rho \prox_{\rho^{-1} g_{\mathcal{N}}^*} \big( \rho^{-1} \bbeta \big).
    \end{align*}
\end{repeattheorem}

% show that our algorithm evaluates prox_{g_N} correctly.

\begin{proof}{Proof of Theorem~\ref{theorem:evaluate_prox_g_algorithm_correctness}}
    The primal update~\eqref{eq:prox:gN} follows directly from the Extended Moreau Decomposition~\citep[Theorem 6.45]{beck2017first}. We thus focus on evaluating $\prox_{\rho g_{\mathcal{N}}^*}$.
    
    Recall from Lemma~\ref{lemma:function_g_conjugate_in_BnB} that $g_{\mathcal{N}}^*$ decomposes separably over the index sets $\mathcal{J}_0, \mathcal{J}_1,$ and $\mathcal{J}_f$.
    Consequently, the proximal optimization problem decomposes across these index sets.
    Let
    \begin{align*}
        \balpha^\star := \prox_{\rho g_{\mathcal{N}}^*}(\bbeta) 
        = \argmin_{\balpha \in \mathbb R^p} \ \frac{1}{2} \| \balpha - \bbeta \|_2^2 + \rho g_{\mathcal{N}}^*(\balpha).
    \end{align*}
    Using the separable form of $g_{\mathcal{N}}^*$, the objective can be written as
    \begin{align*}
        \frac{1}{2} \| \balpha - \bbeta \|_2^2 + \rho g_{\mathcal{N}}^*(\balpha)
        =& \frac{1}{2} \|\balpha_{\mathcal{J}_0} - \bbeta_{\mathcal{J}_0}\|_2^2 
        \quad + \quad \frac{1}{2} \|\balpha_{\mathcal{J}_1} - \bbeta_{\mathcal{J}_1}\|_2^2 + \rho \sum_{j \in \mathcal{J}_1} H_M(\alpha_j) \\
        \quad &+ \frac{1}{2} \|\balpha_{\mathcal{J}_f} - \bbeta_{\mathcal{J}_f}\|_2^2 + \rho \textstyle \TopSum_{\bar k} \big(\bm{H}_M(\balpha_{\mathcal{J}_f})\big),
    \end{align*}
    where $\bar k = k - |\mathcal{J}_1|$.
    The first two subproblems are trivially solved by $\balpha^\star_{\mathcal{J}_0} = \bbeta_{\mathcal{J}_0}$ and $\balpha^\star_{\mathcal{J}_1} = [\prox_{\rho H_M}(\beta_j)]_{j \in \mathcal J_1}$, the standard proximal operator of the Huber loss for every $j \in \mathcal J_1$.
    
    The core difficulty lies in solving the last optimization problem. For notational simplicity, let $\bar \bbeta = \bbeta_{\mathcal{J}_f}$ and $\bar \balpha = \balpha_{\mathcal{J}_f}$. We aim to solve the reformulated problem
    \begin{equation*} 
        \min_{\bar \balpha \in \mathbb R^{\bar p}} ~ \frac{1}{2} \|\bar \balpha - \bar \bbeta\|_2^2 + \rho \textstyle \TopSum_{\bar k} \big( \bm{H}_M(\bar \balpha) \big).
    \end{equation*}
    We simplify the problem using two structural properties of the optimal solution $\bar \balpha^\star$.
    First, since the Huber loss is an even function, we have $\sgn(\bar \balpha^\star) = \sgn(\bar \bbeta)$.
    Second, if $|\bar \beta_i| \ge |\bar \beta_j|$, then $|\bar \alpha^\star_i| \ge |\bar \alpha^\star_j|$.
    For the sake of contradiction, suppose the opposite were true $|\bar \alpha^\star_i| < |\bar \alpha^\star_j|$.
    Then we could swap $\alpha^\star_i$ and $ \alpha^\star_j$ to further decrease the loss function, which contradict with the fact that the solution $\bar{\balpha}^\star$ is already optimal.
    
    Using these properties and the definition of $\TopSum_{\bar k}$ operator, we can reformulate the above minimization problem as a generalized isotonic regression problem on the magnitudes $|\bar \balpha|$ as follows
    \begin{equation}
    \label{eq:ison}
    \begin{aligned}
        \min_{\bnu \in \mathbb{R}^{\bar p}_+} \quad \sum_{j=1}^{\bar p} \frac{1}{2} (\nu_j - |\bar \beta_{\pi(j)}|)^2 + \rho_j H_M(\nu_j) \quad \text{s.t.} \quad  \nu_1 \ge \nu_2 \ge \dots \ge \nu_{\bar p} \ge 0,
    \end{aligned}
    \end{equation}
    where $\bar \beta_{\pi(j)}$ denotes the $j$-th largest element of $|\bar \bbeta|$ in magnitude, and the weights are defined as $\rho_j = \rho$ for $j \le \bar k$ and $\rho_j = 0$ for $j > \bar k$. 
    If $\bnu^\star$ solves~\eqref{eq:ison}, we can recover $\bar \balpha^\star$ via $\bar \balpha^\star = \sign(\bar \bbeta) \odot \bnu^\star$.
    
    The optimization problem~\eqref{eq:ison} minimizes a sum of convex functions under a total order constraint. After sorting, it can be solved exactly in linear time using the PAVA algorithm presented in~\citep{busing2022monotone}. 
    Algorithm~\ref{alg:prox_of_g_conjugate_root_node} implements this procedure. Lines 6--11 perform the PAVA steps, iteratively merging adjacent blocks that violate the monotonicity constraint $\nu_j \ge \nu_{j+1}$. 
    Since sorting takes $\mathcal{O}(\bar p \log \bar p)$ and the PAVA scan takes $\mathcal{O}(\bar p)$, the total complexity is dominated by the sort. This completes the proof.
    \hfill \Halmos
\end{proof}

\subsection{GLM Regularity Conditions for the Framework (Proposition~\ref{proposition:regularity})}
\label{ec_proof:regularity}

\begin{repeatproposition}[Proposition~\ref{proposition:regularity}]
\label{ec_proposition:regularity}
    Consider the primal objective $\Phi ( \bbeta ) = F ( \bX \bbeta ) + G ( \bbeta )$, where $F(\bz) := f (\bz, \by )$ with $f: \mathbb R^n \times \mathbb R^n \to \mathbb R$ being strictly convex, locally smooth, and firmly convex in $\bz$, and $G (\bbeta ) := 2 \lambda_2 \, g_{\mathcal{N}}\left(\bbeta\right)$ with $\lambda_2 > 0$ and $g_{\mathcal{N}}$ being defined in~\eqref{eq:function_g_definition}. Then, Assumptions~\ref{assumption:F:G}--\ref{assumption:loss_function_is_essentially_strictly_convex} hold.
\end{repeatproposition}

\begin{proof}{Proof of Proposition~\ref{proposition:regularity}}
    Since $f(\cdot,\by)$ is strictly convex in its first argument $\bz$, there are no lines along which $F$ is finite and affine.
    Additionally, since $f$ is real-valued, convex, and locally smooth, $F$ is trivially proper, closed and convex.  
    Moreover, Lemma~\ref{lemma:g_is_proper_closed_and_convex} establishes that $g_{\mathcal{N}}$, or equivalently $G$, is proper, closed, and convex with a compact domain.
    Since $\dom(G)$ is compact, there are no lines along which $G$ is finite and affine. Thus, Assumptions~\ref{assumption:F:G} and \ref{assumption:loss_function_is_essentially_strictly_convex} are satisfied.

    Since $F$ is locally smooth and real-valued, it is differentiable everywhere and $\inter(\dom(F)) = \mathbb R^n$. The domain of $G$ is defined by box and cardinality constraints, which form a nonempty polyhedron with nonempty relative interior. Thus, $\rint(\dom(\Phi))$ is nonempty, guaranteeing the existence of a Slater point $\bbeta_s$. 
    For the dual, since $\dom(G)$ is compact, its conjugate $G^*$ is real-valued and finite everywhere, implying $\inter(\dom(G^*)) = \mathbb{R}^p$.
    Since there are no lines along which $F$ is finite and affine, $\inter(\dom(F^*))$ is nonempty \citep[Corollary~13.4.2]{rockafellar1970convex}. Hence, the intersection of the interiors is nonempty, guaranteeing the existence of a Slater point $\bzeta_s$. 
    Thus, Assumption~\ref{assumption:standard_fenchel_duality_assumption} is satisfied.

    The optimal primal solution set $\mathcal{B}^\star$ is a closed subset of $\dom(G)$. Since $\dom(G)$ is compact thanks to Lemma~\ref{lemma:g_is_proper_closed_and_convex}, $\mathcal{B}^\star$ is compact. Since $\dom(F) = \mathbb{R}^n$, the inclusion $\bX \mathcal{B}^\star \subset \inter(\dom(F))$ holds trivially. This verifies Assumption~\ref{assumption:quadratic}\,(i).
    Additionally, $F$ is firmly convex by the assumption of the lemma. $G$ is also firmly convex thanks to Lemma~\ref{lemma:g_and_g_Fenchel_are_PLQ_and_firmly_convex}. This verifies Assumption~\ref{assumption:quadratic}\,(ii).
    
    Since $G^*$ is PLQ thanks to Lemma~\ref{lemma:g_and_g_Fenchel_are_PLQ_and_firmly_convex}, its subdifferential is a polyhedral set.
    By Assumption~\ref{assumption:loss_function_is_essentially_strictly_convex}, $F$ is strictly convex.
    Since $F$ is locally smooth and real-valued, it is differentiable everywhere and $\dom(\partial F) = \mathbb{R}^n$, so $F$ is essentially strictly convex. Therefore, $F^*$ is essentially smooth~\citep[Theorem~26.3]{rockafellar1970convex}.
    Since $F^*$ is essentially smooth, \citep[Theorem~26.1]{rockafellar1970convex} implies $\dom(\partial F^*) = \inter(\dom(F^*))$.
    The KKT condition $\bX \bbeta^\star \in \partial F^*(-\bzeta^\star)$ then yields $-\bzeta^\star \in \inter(\dom(F^*))$.
    Since $\dom(G^*) = \mathbb{R}^p$, $\bX^\top \bzeta^\star \in \inter(\dom(G^*))$ holds trivially. This verifies Assumption~\ref{assumption:quadratic}\,(iv).
    Moreover, $-\bzeta^\star \in \inter(\dom(F^*))$ implies $\partial F^*(-\bzeta^\star) = \{\nabla F^*(-\bzeta^\star)\}$ by \citep[Theorem~26.1]{rockafellar1970convex}, which is a polyhedral set. This verifies Assumption~\ref{assumption:quadratic}\,(iii) and concludes the proof.
    \hfill \Halmos
\end{proof}

% ==============================================================================
% Part III: GLM loss verification details referenced in Section 4.3
% ==============================================================================

\subsection{Verifications for Common GLM Loss Functions}
\label{ec:glm_loss_verifications}
% \noindent
% In particular, because $\dom(G)$ is compact in the perspective relaxation (Lemma~\ref{lemma:g_is_proper_closed_and_convex}), its image $\bX(\dom(G))$ is also compact.
% Consequently, the local smoothness and firm convexity constants above apply uniformly over $\bz \in \bX(\dom(G))$, verifying the assumptions of Proposition~\ref{proposition:regularity} for these loss functions.
This appendix verifies that several standard GLM loss functions satisfy the regularity conditions assumed in Proposition~\ref{proposition:regularity}, namely that $F$ is strictly convex, locally smooth, and firmly convex.
Throughout, we use $\bz = \bX \bbeta \in \bbR^n$ to denote the prediction vector and write the loss as $F(\bz) := f(\bz,\by)$.
For multinomial logistic regression, we treat $\bz$ as the stacked vector of class scores after fixing a reference class, as detailed in Lemma~\ref{lemma:glm_loss_multinomial_logistic_regularities}.

\begin{lemma}[Linear regression (least squares)]
\label{lemma:glm_loss_least_squares_regularities}
Let $\by \in \bbR^n$ and define the least squares loss
\[
    F(\bz) := \frac{1}{2}\|\bz - \by\|_2^2, \qquad \bz \in \bbR^n.
\]
Then, $F$ is strictly convex,~\emph{globally} smooth, and firmly convex.
\end{lemma}
\begin{proof}{Proof}
The function $F$ is twice continuously differentiable with
\[
    \nabla F(\bz) = \bz - \by,
    \qquad
    \nabla^2 F(\bz) = \bI \quad \text{for all } \bz \in \bbR^n.
\]
Hence $F$ is $1$-strongly convex and $1$-smooth on $\bbR^n$, which implies strict convexity and local smoothness.
Moreover, for any $\bnu \in \bbR^n$, the tilted function $F_{\bnu}(\bz) := F(\bz) - \bnu^\top \bz$ has the same Hessian $\nabla^2 F_{\bnu} \equiv \bI$, and is therefore $1$-strongly convex.
Strong convexity implies the quadratic growth condition, so $F$ is firmly convex in the sense of Section~\ref{sec:methodology}.
\hfill \Halmos
\end{proof}

\begin{lemma}[Logistic regression]
\label{lemma:glm_loss_logistic_regularities}
Let $\by \in \{-1,1\}^n$ and define the logistic loss
\[
    F(\bz) := \sum_{i=1}^n \log\!\left(1 + \exp\!\left(-y_i z_i\right)\right),
    \qquad \bz \in \bbR^n.
\]
Then, $F$ is strictly convex, \emph{globally} smooth, and firmly convex.
\end{lemma}
\begin{proof}{Proof}
The function $F$ is twice continuously differentiable with gradient and Hessian given componentwise by
\[
    \big(\nabla F(\bz)\big)_i = -\frac{y_i}{1+\exp(y_i z_i)},
    \qquad
    \nabla^2 F(\bz) = \diag\!\left(\left\{ \frac{\exp(y_i z_i)}{(1+\exp(y_i z_i))^2} \right\}_{i=1}^n\right).
\]
For all finite $\bz$, we have $\nabla^2 F(\bz) \succ \bm{0}$, and hence $F$ is strictly convex on $\bbR^n$.

To show global smoothness, note that since $\|\nabla^2 F(\bz)\|_2$ equals the largest diagonal entry and
\[
    0 < \frac{\exp(y_i z_i)}{(1+\exp(y_i z_i))^2} \le \frac{1}{4} \quad \text{for all } \bz \in \bbR^n.
\]
Thus, we have $\sup_{\bz\in\bbR^n}\|\nabla^2 F(\bz)\|_2 \le 1/4$, which implies that $F$ is globally smooth.

For firm convexity, note that the Hessian is continuous and positive definite everywhere.
Hence, by compactness, the minimum eigenvalue over $\mathcal{B}$ satisfies
\[
    m_{\mathcal B} := \inf_{\bz\in\mathcal B}\lambda_{\min}\!\left(\nabla^2 F(\bz)\right) > 0.
\]
Therefore, $F$ is $m_{\mathcal B}$-strongly convex on $\mathcal{B}$.
For any $\bnu\in\bbR^n$, the tilted function $F_{\bnu}(\bz)=F(\bz)-\bnu^\top \bz$ has the same Hessian and is also $m_{\mathcal B}$-strongly convex on $\mathcal{B}$, which implies the quadratic growth condition on $\mathcal{B}$.
Thus, $F$ is firmly convex.
\hfill \Halmos
\end{proof}

\begin{lemma}[Poisson regression]
\label{lemma:glm_loss_poisson_regularities}
Let $\by \in \bbR^n$ with $y_i \in \{0,1,2,\ldots\}$ for all $i\in[n]$, and define the Poisson loss
\[
    F(\bz) := \sum_{i=1}^n \left(\exp(z_i) - y_i z_i\right),
    \qquad \bz \in \bbR^n.
\]
Then, $F$ is strictly convex, locally smooth, and firmly convex.
\end{lemma}
\begin{proof}{Proof}
The function $F$ is twice continuously differentiable with
\[
    \big(\nabla F(\bz)\big)_i = \exp(z_i) - y_i,
    \qquad
    \nabla^2 F(\bz) = \diag\!\left(\left\{ \exp(z_i) \right\}_{i=1}^n\right).
\]
Since $\exp(z_i) > 0$ for all $z_i\in\bbR$, we have $\nabla^2 F(\bz)\succ\bm{0}$ for all $\bz$, and $F$ is strictly convex on $\bbR^n$.

Let $\mathcal{B}\subset \bbR^n$ be compact and define
\[
    \underline z := \min_{\bz\in\mathcal B}\min_{i\in[n]} z_i,
    \qquad
    \overline z := \max_{\bz\in\mathcal B}\max_{i\in[n]} z_i,
\]
which are finite by compactness.
Then, for all $\bz\in\mathcal B$,
\[
    e^{\underline z}\,\bI \preceq \nabla^2 F(\bz) \preceq e^{\overline z}\,\bI.
\]
The upper bound implies that $\nabla F$ is Lipschitz on $\mathcal B$ (local smoothness), and the lower bound implies that $F$ is $e^{\underline z}$-strongly convex on $\mathcal B$.
As in Lemma~\ref{lemma:glm_loss_logistic_regularities}, strong convexity of the tilted functions on arbitrary compact sets yields the quadratic growth condition, and thus $F$ is firmly convex.
\hfill \Halmos
\end{proof}

\begin{lemma}[Gamma (exponential) regression]
\label{lemma:glm_loss_gamma_regularities}
Let $\by \in \bbR^n$ with $y_i>0$ for all $i\in[n]$, and define the Gamma (exponential) regression loss
\[
    F(\bz) := \sum_{i=1}^n \left(y_i \exp(-z_i) + z_i\right), \qquad \bz \in \bbR^n.
\]
Then, $F$ is strictly convex, locally smooth, and firmly convex.
\end{lemma}
\begin{proof}{Proof}
The function $F$ is twice continuously differentiable with
\[
    \big(\nabla F(\bz)\big)_i = -y_i \exp(-z_i) + 1,
    \qquad
    \nabla^2 F(\bz) = \diag\!\left(\left\{ y_i \exp(-z_i) \right\}_{i=1}^n\right).
\]
Since $y_i>0$ and $\exp(-z_i)>0$ for all $z_i\in\bbR$, we have $\nabla^2 F(\bz)\succ\bm{0}$ for all $\bz$, and thus $F$ is strictly convex on $\bbR^n$.

Let $\mathcal{B}\subset \bbR^n$ be compact and define
\[
    \underline z := \min_{\bz\in\mathcal B}\min_{i\in[n]} z_i,
    \qquad
    \overline z := \max_{\bz\in\mathcal B}\max_{i\in[n]} z_i,
\]
which are finite by compactness.
Then, for all $\bz\in\mathcal B$,
\[
    \diag\!\left(\left\{ y_i e^{-\overline z} \right\}_{i=1}^n\right) \preceq \nabla^2 F(\bz) \preceq \diag\!\left(\left\{ y_i e^{-\underline z} \right\}_{i=1}^n\right).
\]
The upper bound implies that $\nabla F$ is Lipschitz on $\mathcal B$ (local smoothness), and the lower bound implies that $F$ is strongly convex on $\mathcal B$.
As in Lemma~\ref{lemma:glm_loss_logistic_regularities}, strong convexity of the tilted functions on arbitrary compact sets yields the quadratic growth condition, and thus $F$ is firmly convex.
\hfill \Halmos
\end{proof}

\begin{lemma}[Multinomial logistic regression]
\label{lemma:glm_loss_multinomial_logistic_regularities}
Fix an integer $K\ge 2$, assume that the coefficient vector for class $K$ is zero.
For each $i\in[n]$, let $\by_i \in \{0,1\}^{K-1}$ satisfy $\bm{1}^\top \by_i \le 1$.
Define $\bz_i \in \bbR^{K-1}$ and consider the multinomial logistic regression loss
\[
    F(\bz) := \sum_{i=1}^n \left(\log\!\left(1 + \bm{1}^\top \exp(\bz_i)\right) - \by_i^\top \bz_i\right),
\]
where $\bz := (\bz_1,\ldots,\bz_n) \in \bbR^{n (K-1)}$ stacks the row vectors $\bz_i$.
Then $F$ is strictly convex, locally smooth, and firmly convex with respect to $\bz$.
\end{lemma}
\begin{proof}{Proof}
For each $i\in[n]$, define
\[
    \bp_i := \frac{\exp(\bz_i)}{1+\bm{1}^\top \exp(\bz_i)} \in \bbR^{K-1},
    \qquad
    p_{i0} := \frac{1}{1+\bm{1}^\top \exp(\bz_i)} \in (0,1),
\]
so that $p_{i0}+\bm{1}^\top \bp_i=1$ and all entries are strictly positive.
Then $F$ is twice continuously differentiable and its Hessian is block-diagonal, with the $i$-th block given by
\[
    \nabla^2_{\bz_i} F(\bz) = \diag\!\big(\bp_i\big) - \bp_i \bp_i^\top,
\]
For any nonzero $\bv\in\bbR^{K-1}$, we have
\[
    \bv^\top \nabla^2_{\bz_i} F(\bz)\, \bv
    = \sum_{l=1}^{K-1} p_{il} v_l^2 - \Big(\sum_{l=1}^{K-1} p_{il} v_l\Big)^2,
\]
which is the variance of a random variable taking the value $v_l$ with probability $p_{il}$ and $0$ with probability $p_{i0}>0$.
This variance is strictly positive whenever $\bv\neq \bm{0}$, so each block is positive definite and therefore $\nabla^2 F(\bz)\succ \bm{0}$ for all $\bz$.
Hence $F$ is strictly convex.

Let $\mathcal{B}$ be any compact subset of the $\bz$-space.
Since $\nabla^2 F$ is continuous, $\|\nabla^2 F(\bz)\|_2$ is bounded above on $\mathcal{B}$, implying that $\nabla F$ is Lipschitz on $\mathcal{B}$ (local smoothness).
Moreover, since $\nabla^2 F(\bz)\succ \bm{0}$ for all $\bz$ and $\mathcal B$ is compact, there exists $m_{\mathcal B}>0$ such that $\nabla^2 F(\bz)\succeq m_{\mathcal B}\bI$ for all $\bz\in\mathcal B$, so $F$ is strongly convex on $\mathcal B$.
As in Lemma~\ref{lemma:glm_loss_logistic_regularities}, strong convexity of the tilted functions on arbitrary compact sets yields the quadratic growth condition, and thus $F$ is firmly convex.
\hfill \Halmos
\end{proof}

\section{Experimental Setup Details}
\label{ec_expt:experimental_setup}

% \subsection{Setup for Evaluating Proximal Operators}
% \label{ec:setup_for_evaluating_proximal_operators}
% The synthetic data generation process is as follows.
% We sample the input vector $\bgamma \in \bbR^p$ from the standard multivariate Gaussian distribution, $\bgamma \sim \calN(\mathbf{0}, \bI_p)$, where $\bI_p$ denotes the identity matrix with dimension $p$.
% We vary the dimension $p \in \{2^0, 2^1, ..., 2^{10}\} \times 10^2$ and set the cardinality $k$ to be $10$, the box constraint $M$ to be $1.0$, and the weight parameter $\rho$  to be $1.0$.
% We report the running time for evaluating these proximal operators.
% To obtain the mean and standard deviation of the running time, we repeat each setting 5 times, each with a different random seed.

\subsection{Setup for Solving the Perspective Relaxation}
\label{ec_expt:setup_for_solving_the_perspective_relaxation}

We generate our synthetic datasets in the following procedure.
First, we sample each feature vector $\bx_i \in \bbR^p $ from a Gaussian distribution, $\bx_i \sim \calN(\mathbf{0}, \bSigma)$, where the covariance matrix has entries $\Sigma_{jl} = \sigma^{\vert{j-l}}$.
The variable $\sigma \in (0, 1)$ controls the features correlation: if we increase $\sigma$, feature columns in the design matrix $\bX$ become more correlated.
Throughout the experimental section, we set $\sigma=0.5$.
Next, we create the sparse coefficient vector $\bbeta^*$ with $k$ equally spaced nonzero entries, where $\beta^*_j = 1$ if $j \text{ mod } (p/k) = 0$ and $\beta^*_j = 0$ otherwise.
After these two steps, we build the prediction vector $\by$.
If our loss function is squared error loss (regression task), we set $y_i = \bx_i^T \bbeta^* + \epsilon_i$, where $\epsilon_i$ is a Gaussian random noise with $\epsilon_i \sim \calN(0, \frac{\Vert{\bX \bbeta^*}}{\text{SNR}})$, and $\text{SNR}$ stands for the signal-to-noise ratio.
In all our experiments, we choose $\text{SNR}=5$.
If our loss function is logistic loss (classification task), we set $y_i \sim Bern(\bx_i^T \bbeta^* + \epsilon_i)$, where $Bern(P)$ is a Bernoulli random variable with $\bbP(y_i = 1) = P$ and $\bbP(y_i = -1) = 1 - P$.

% For this experiment, we vary the feature dimension $p \in \{1000, 2000, 4000, 8000, 16000\}$.
% We control the sample size by using a parameter called $n$-to-$p$ ratio, or sample to feature ratio.
% For the results in the main paper, we set $n$-to-$p$ ratio to be $1.0$, the box constraint $M$ to be $2$, the number of nonzero coefficients k (also the cardinality constraint) to be $10$, and $\ell_2$ regularization coefficient $\lambda_2$ to be $1.0$.
% Again, we report and compare the running times, with means and standard deviations calculated based on 5 repeated simulations with different random seeds.

\subsection{Setup for Demonstrating Restart Scheme Generality on LASSO Problems}
\label{ec_expt:setup_for_restart_generality_lasso}
To demonstrate that our restart scheme is applicable beyond perspective relaxations, we consider two LASSO-type composite problems:
\begin{align*}
    \min_{\bbeta \in \bbR^p} \quad & f(\bX\bbeta, \by) + \lambda_1 \lVert \bbeta \rVert_1 \quad \text{($\ell_1$-regularized)},\\
    \min_{\bbeta \in \bbR^p} \quad & f(\bX\bbeta, \by) + \delta_{\lVert \bbeta \rVert_1 \le C}(\bbeta) \quad \text{($\ell_1$-ball constrained)},
\end{align*}
where $\delta_{\lVert \bbeta \rVert_1 \le C}(\bbeta)$ is the indicator function of the $\ell_1$-norm ball with radius $C$.
We use the same synthetic data generation procedure as in Appendix~\ref{ec_expt:setup_for_solving_the_perspective_relaxation} and fix $n=p=16000$, $k=10$, and $\sigma=0.5$, with coefficient magnitude $\beta_j^* \in \{0,1\}$ and random seed $0$.
In the $\ell_1$-regularized experiments we set $\lambda_1 = 1.0$, and in the $\ell_1$-ball constrained experiments we set $C = 10.0$.

\subsection{Setup for Certifying Optimality}
\label{ec_expt:setup_for_certifying_optimality_tmp}

\paragraph{Datasets and Preprocessing}
We run on both synthetic and real-world datasets.
For the synthetic datasets, we use the same data generation process as in the previous subsection for solving the perspective relaxation, with $n$-to-$p$ ratio equal to $1.0$, number of nonzero coefficients $k=10$, and the feature correlation parameter $\sigma=0.5$.
We vary the feature dimension $p \in \{1000, 2000, 4000, 8000, 16000\}$.
For the real-world datasets, we use the dataset Santander Customer Transaction Prediction dataset~\citep{santander} for linear regression and DOROTHEA~\cite{asuncion2007uci} for logistic regression.

The Santander dataset has 4459 samples and orginally has 4992 features.
After pruning redundant features, we have 4735 features.
The DOROTHEA dataset has 1950 samples and 100000 features.
After pruning redundant features, we have 91598 features.
For both the Santander and DOROTHEA dataset, we center each feature to have mean $0$ and norm equal to $1$.

\paragraph{Choice of Hyperparameters}
On the synthetic datasets, we set the box constraint $M=2$, the $\ell_2$ regularization coefficient $\lambda_2=1.0$, and the cardinality constraint $k=10$.
On the real-world datasets, we perform 5-fold cross-validation (without the box-constraint) to select the optimal hyperparameters for $\lambda_2$ and the range of $k$ values.
For both datasets, the best $\lambda_2$ from cross-validation is $1.0$.
The best $k$ from cross-validation is around $10$ for Santander and around $5$ for DOROTHEA.
When we run BnB with the box-constraint, we set the box constraint $M$ to be around twice the largest magnitude of $\bbeta$ obtained from the cross-validation.
Based on these cross-validation results, we set $M=10$.
For Santander, we test $k \in \{5, 6, 7, 8, 9, 10\}$, and for DOROTHEA, we test $k \in \{5, 10, 15, 20, 25\}$.

\paragraph{Branch and Bound}
For our method, we implement a customized branch-and-bound (BnB) framework based on the codebase in~\cite{liu2024okridge}.
We use the same heuristics for finding feasible solutions and branching as in~\cite{liu2024okridge}.
To obtain a high-quality feasible solution at each node, we run beamsearch with beam width $5$.
For branching, we use the best beamsearch solution at each node and, among its nonzero coefficients, branch on the variable that would induce the largest loss increase if set to $0$.
This prioritizes important variables early in BnB.
The key difference is that we use our proximal gradient method to compute safe lower bounds at each node for pruning.
For our proximal method, we use FISTA with line search and restart factor $\eta=e^3$, which gave the best empirical performance.

\subsection{Computing Platforms}
When investigating how much GPU can accelerate our computation, we ran the experiments with both CPU and GPU implementations on the Nvidia A100s.
For everything else, we ran the experiments with the CPU implementation on AMD Milan with CPU speed 2.45 Ghz and 8 cores.
% \ToDo{Comment out for original submission?}
% We conducted the experiments in the the Delta system at the National Center for Supercomputing Applications from the Advanced Cyberinfrastructure Coordination Ecosystem: Services \& Support (ACCESS) program~\cite{boerner2023access}.

\section{Additional Experimental Results}
\label{ec:additional_results}

\subsection{Solving the Perspective Relaxation}
\label{ec_expt:perturbation_study_on_solving_the_perspective_relaxation}

We provide perturbation studies on solving the perspective relaxation by varying the box constraint $M$, the $\ell_2$ regularization coefficient $\lambda_2$, and the sample-to-feature ($n$-to-$p$) ratio. Unless otherwise noted, settings match Figure~\ref{fig:solve_convex_relaxation_main_paper} ($M=2.0$, $\lambda_2=1.0$, $n$-to-$p$ ratio $=1$).

Figure~\ref{ec_fig:convex_relaxation_M_1.2} and Figure~\ref{ec_fig:convex_relaxation_M_5.0} tighten and loosen the box constraint to $M=1.2$ and $M=5.0$, respectively. Figure~\ref{ec_fig:convex_relaxation_lambda2_0.1} and Figure~\ref{ec_fig:convex_relaxation_lambda2_10} vary the $\ell_2$ penalty to $\lambda_2 = 0.1$ and $\lambda_2 = 10$. Figure~\ref{ec_fig:convex_relaxation_n_p_ratio_10.0} and Figure~\ref{ec_fig:convex_relaxation_n_p_ratio_0.1} adjust the $n$-to-$p$ ratio to $10.0$ and $0.1$ while keeping $M=2.0$ and $\lambda_2=1.0$.

\begin{figure}[!h]
    \vspace{0em}
    \centering
    \includegraphics[width=1.0\textwidth]{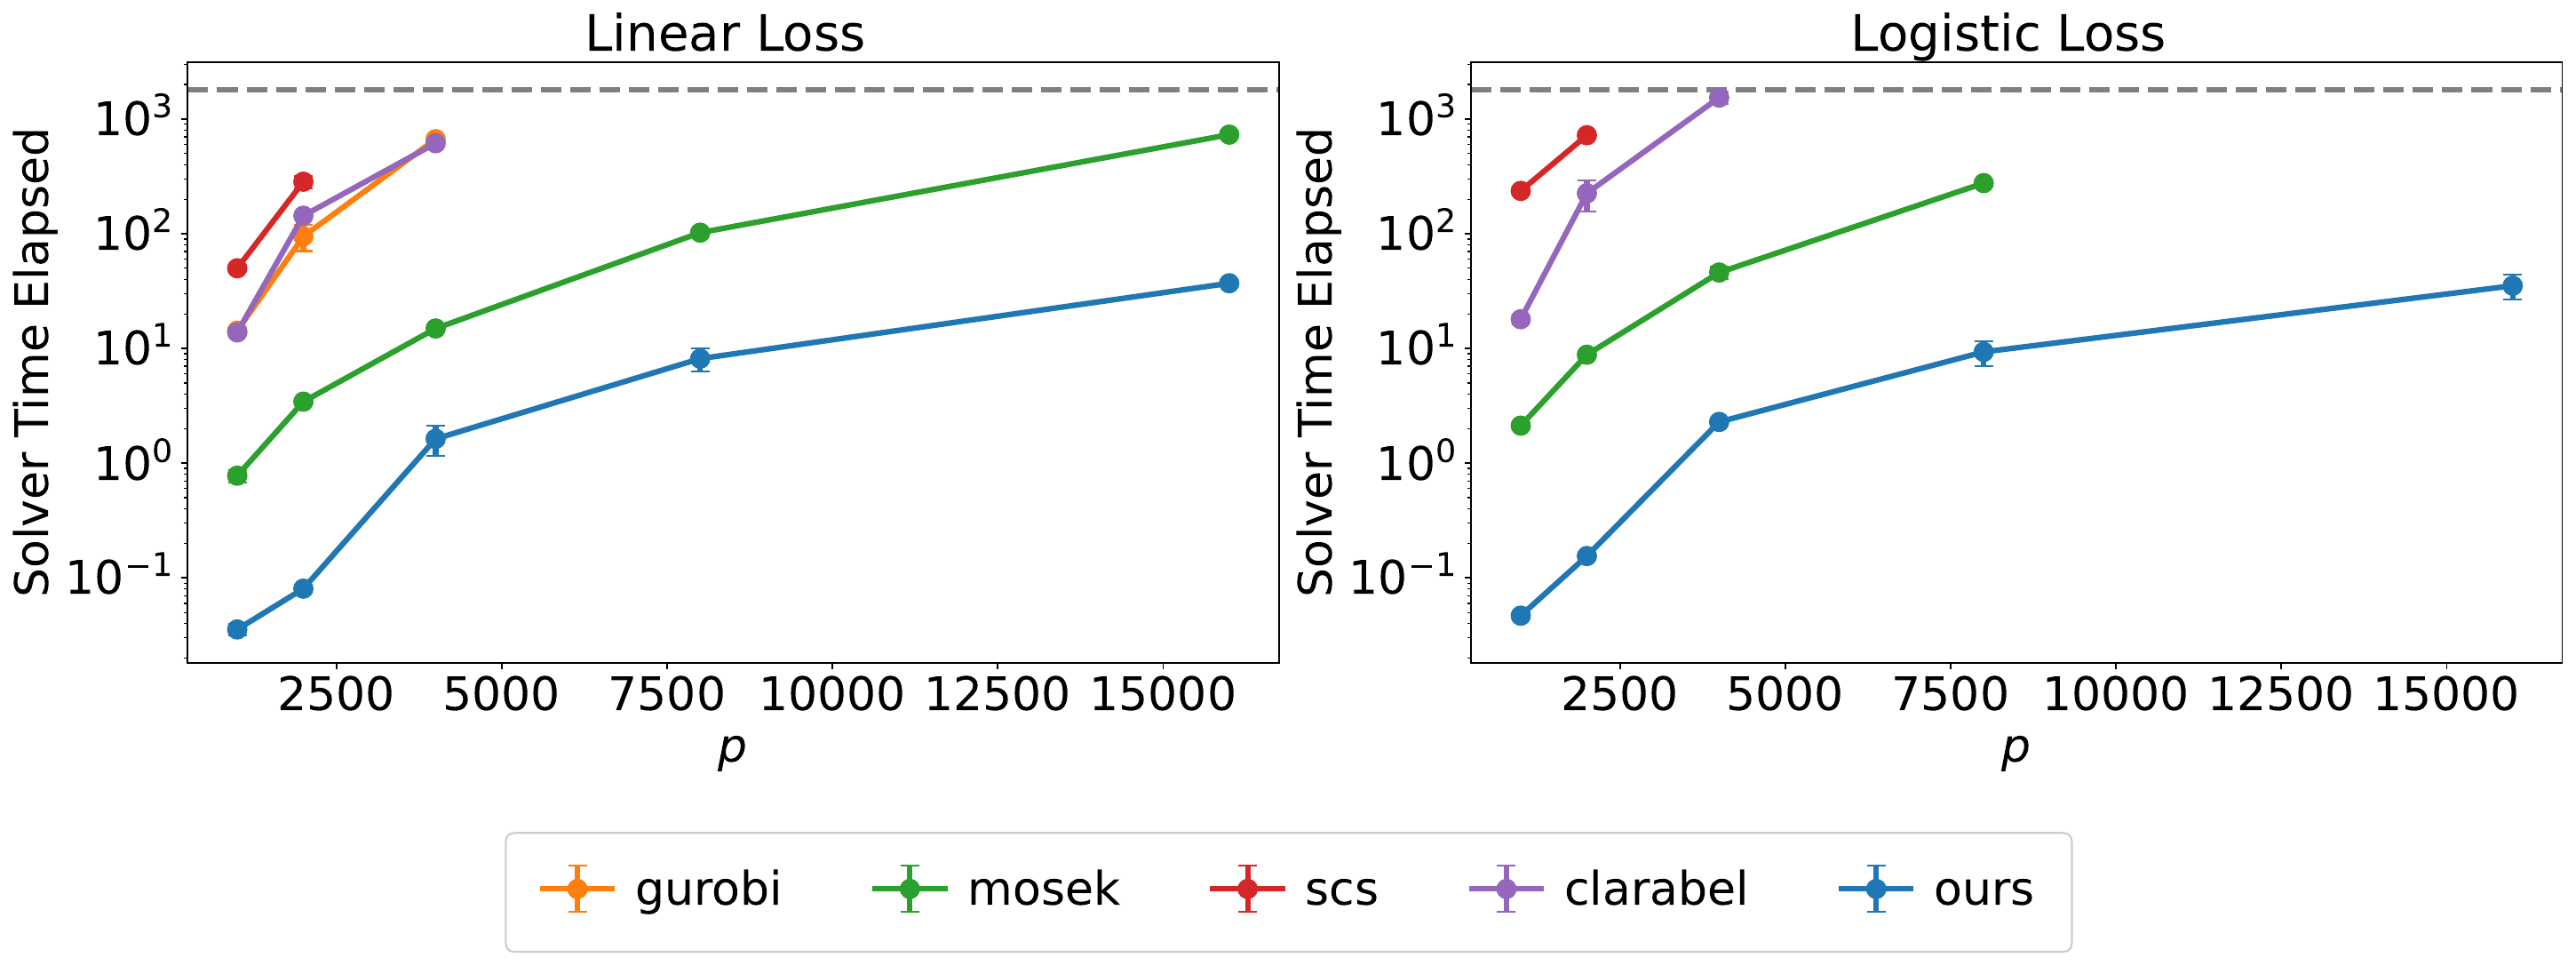}
    \caption{Running time comparison of solving Problem~\ref{obj:perspective_relaxation} when the box constraint is tightened to $M=1.2$.}
    \label{ec_fig:convex_relaxation_M_1.2}
    \vspace{0em}
\end{figure}

\begin{figure}[!h]
    \vspace{0em}
    \centering
    \includegraphics[width=1.0\textwidth]{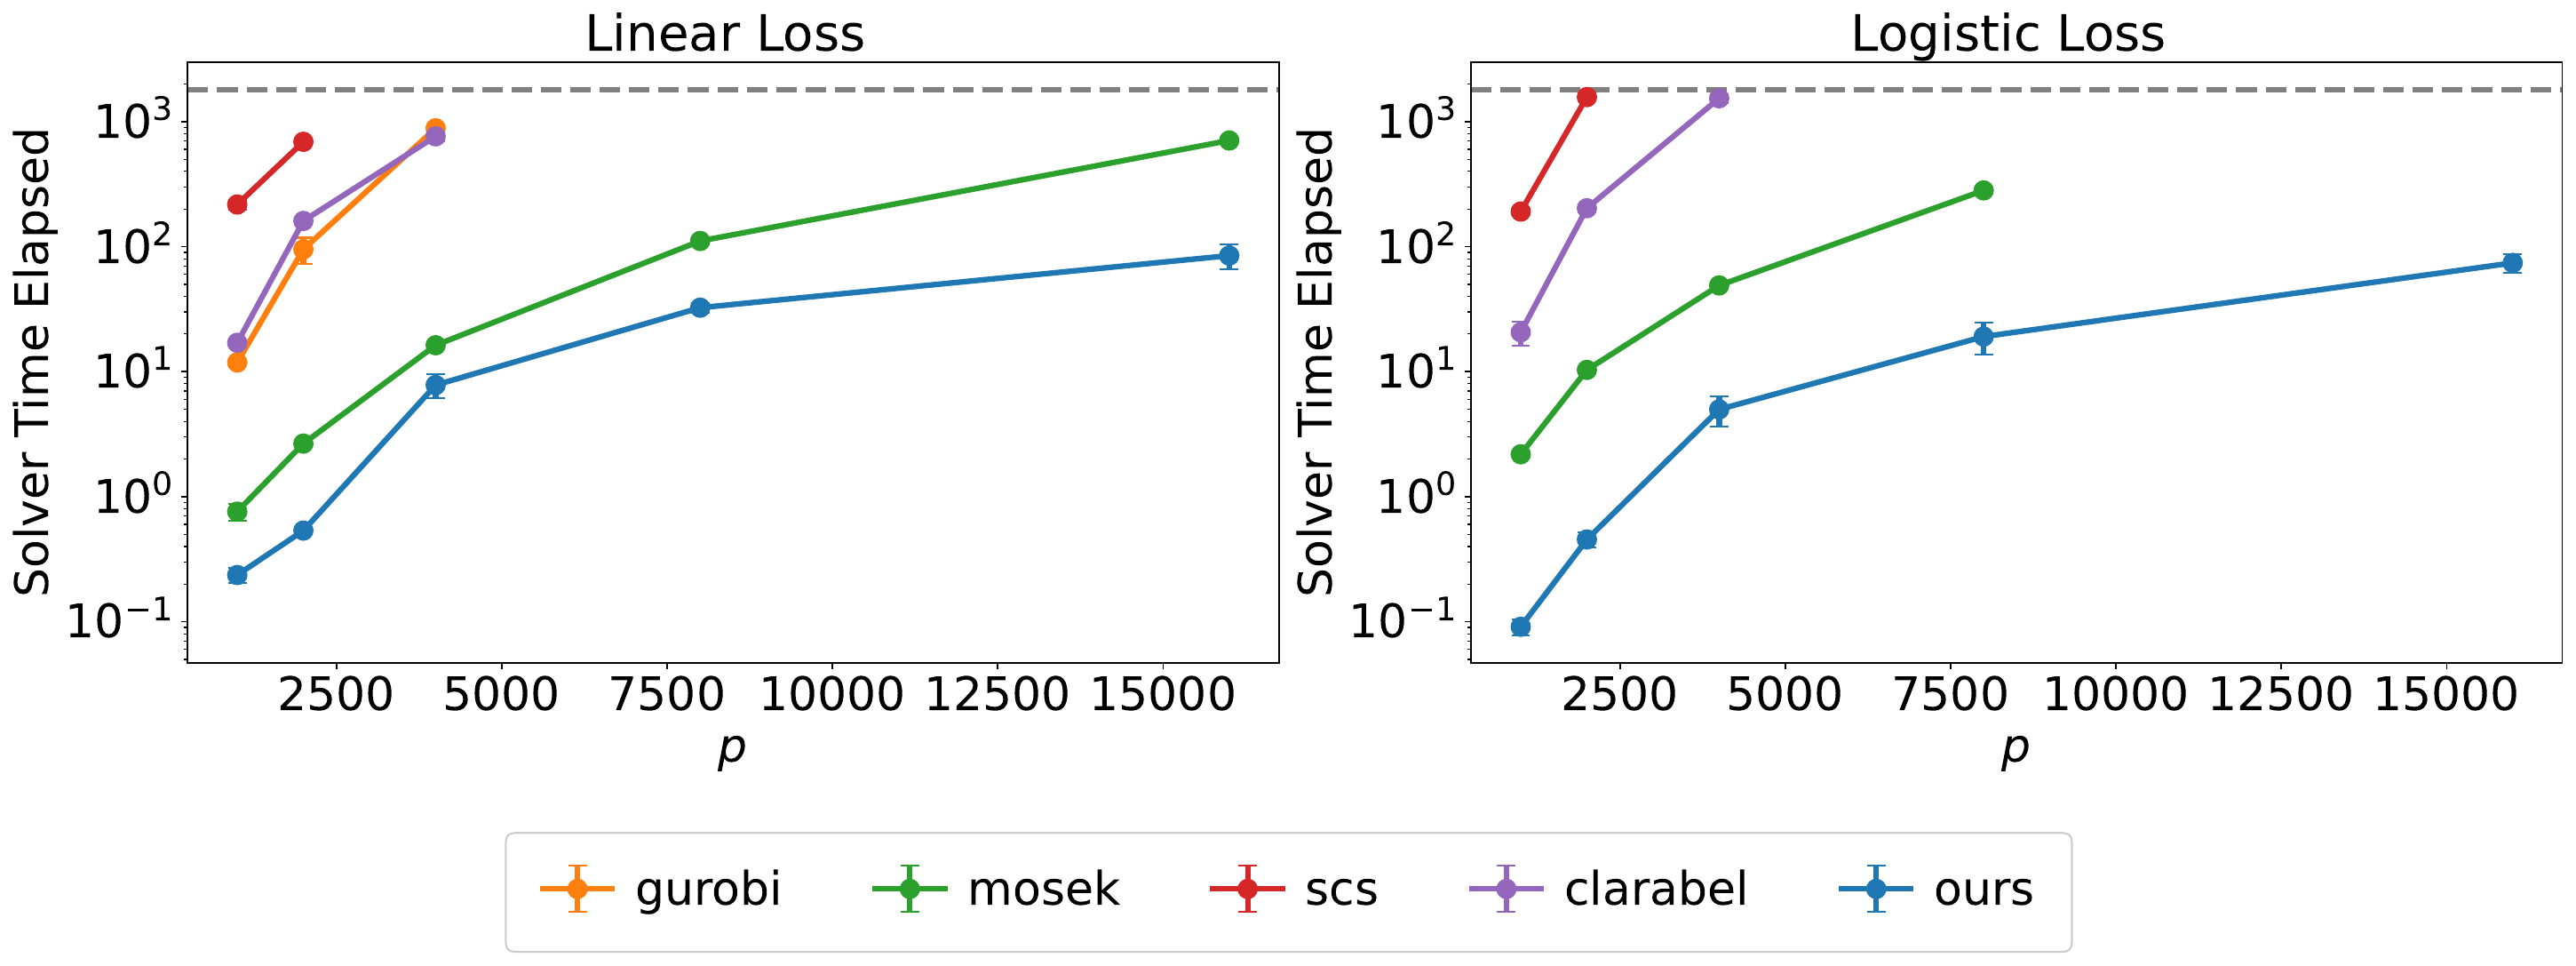}
    \caption{Running time comparison of solving Problem~\ref{obj:perspective_relaxation} when the box constraint is relaxed to $M=5.0$.}
    \label{ec_fig:convex_relaxation_M_5.0}
    \vspace{0em}
\end{figure}

\clearpage

\begin{figure}[!h]
    \centering
    \includegraphics[width=1.0\textwidth]{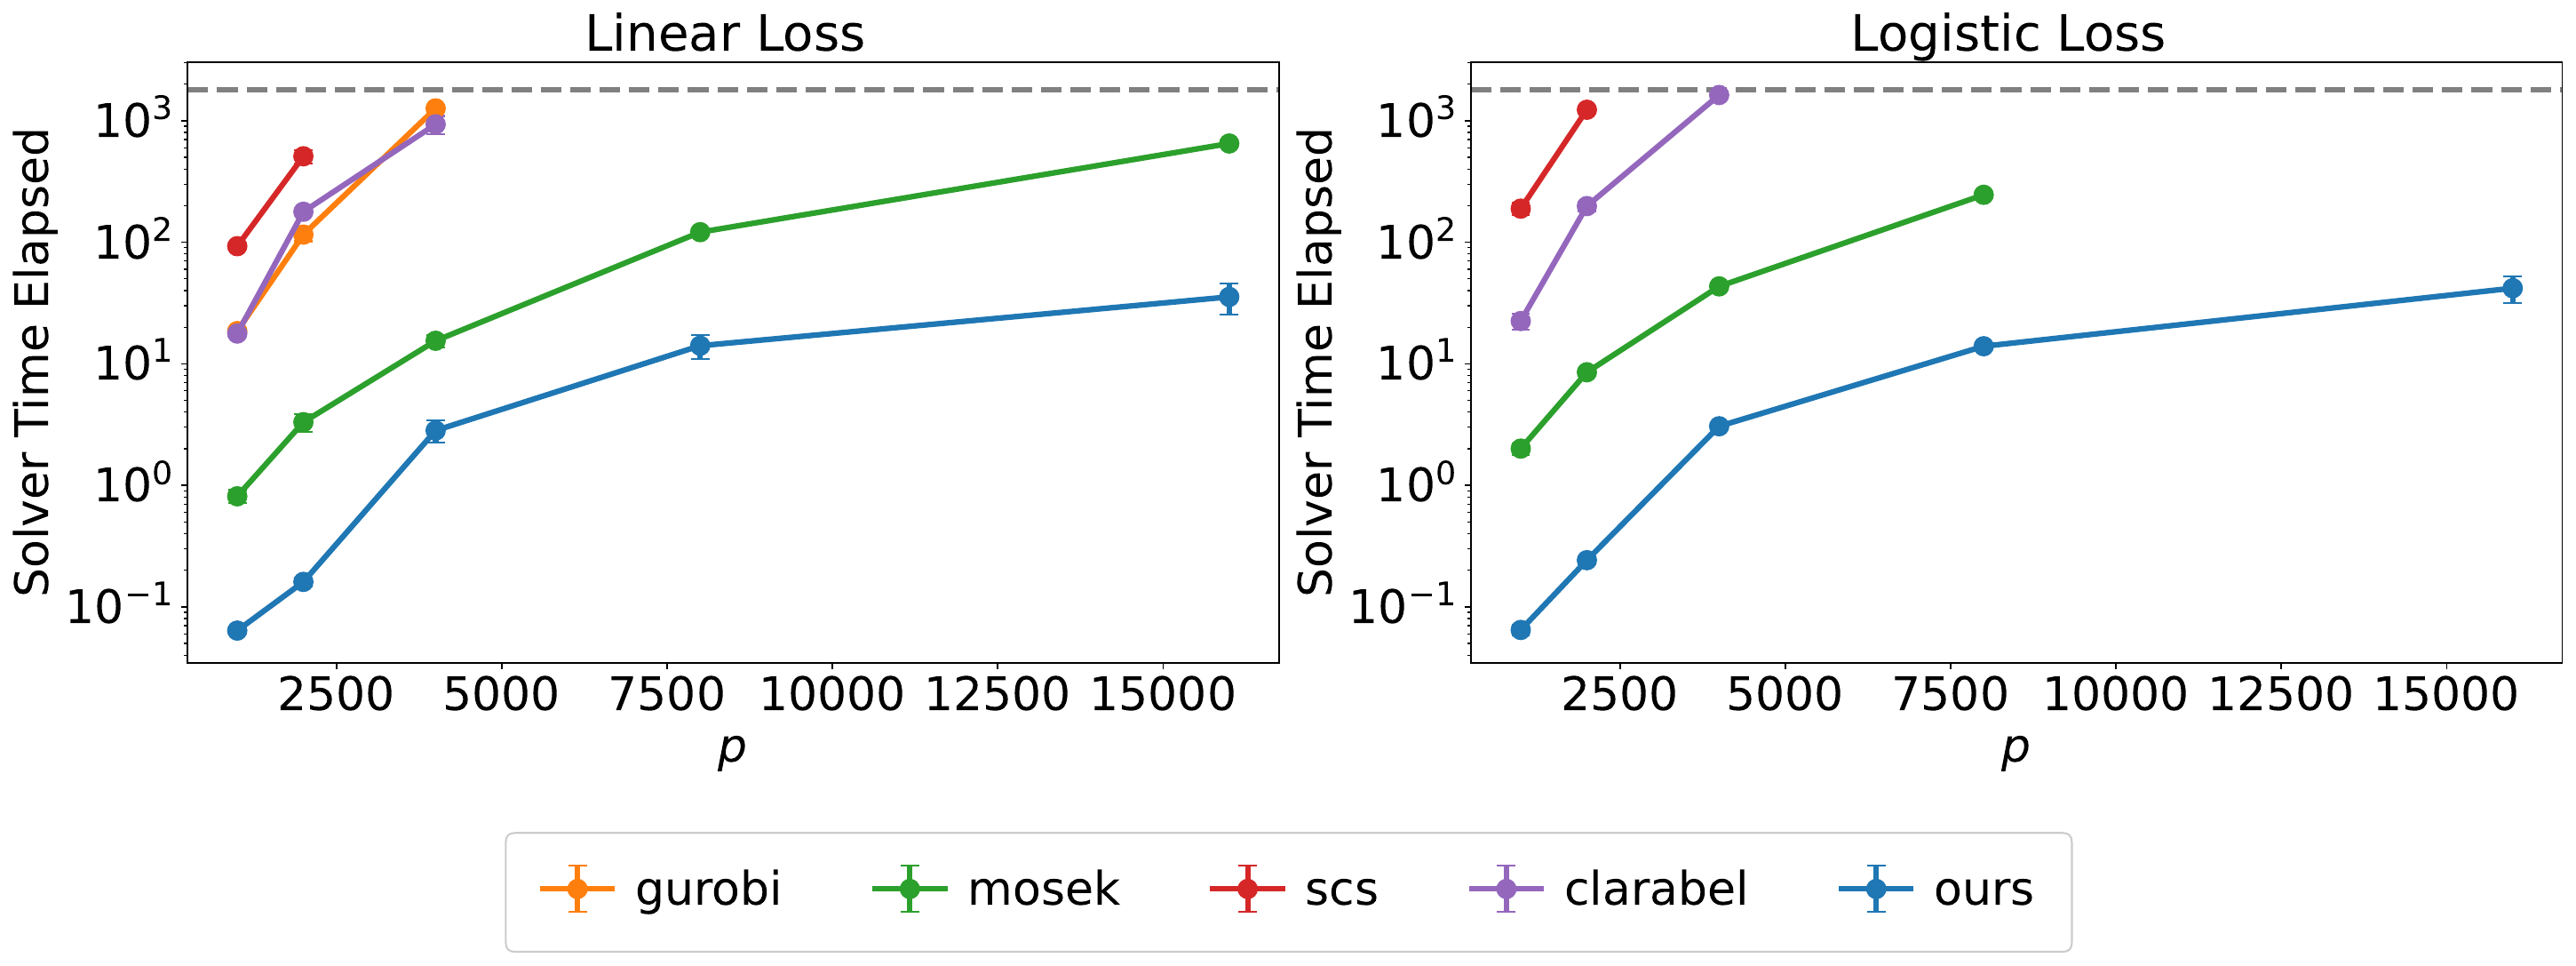}
    \caption{Running time comparison of solving Problem~\ref{obj:perspective_relaxation} with the $\ell_2$ regularization reduced to $\lambda_2 = 0.1$.}
    \label{ec_fig:convex_relaxation_lambda2_0.1}
    \vspace{0em}
\end{figure}

\begin{figure}[!h]
    \centering
    \includegraphics[width=1.0\textwidth]{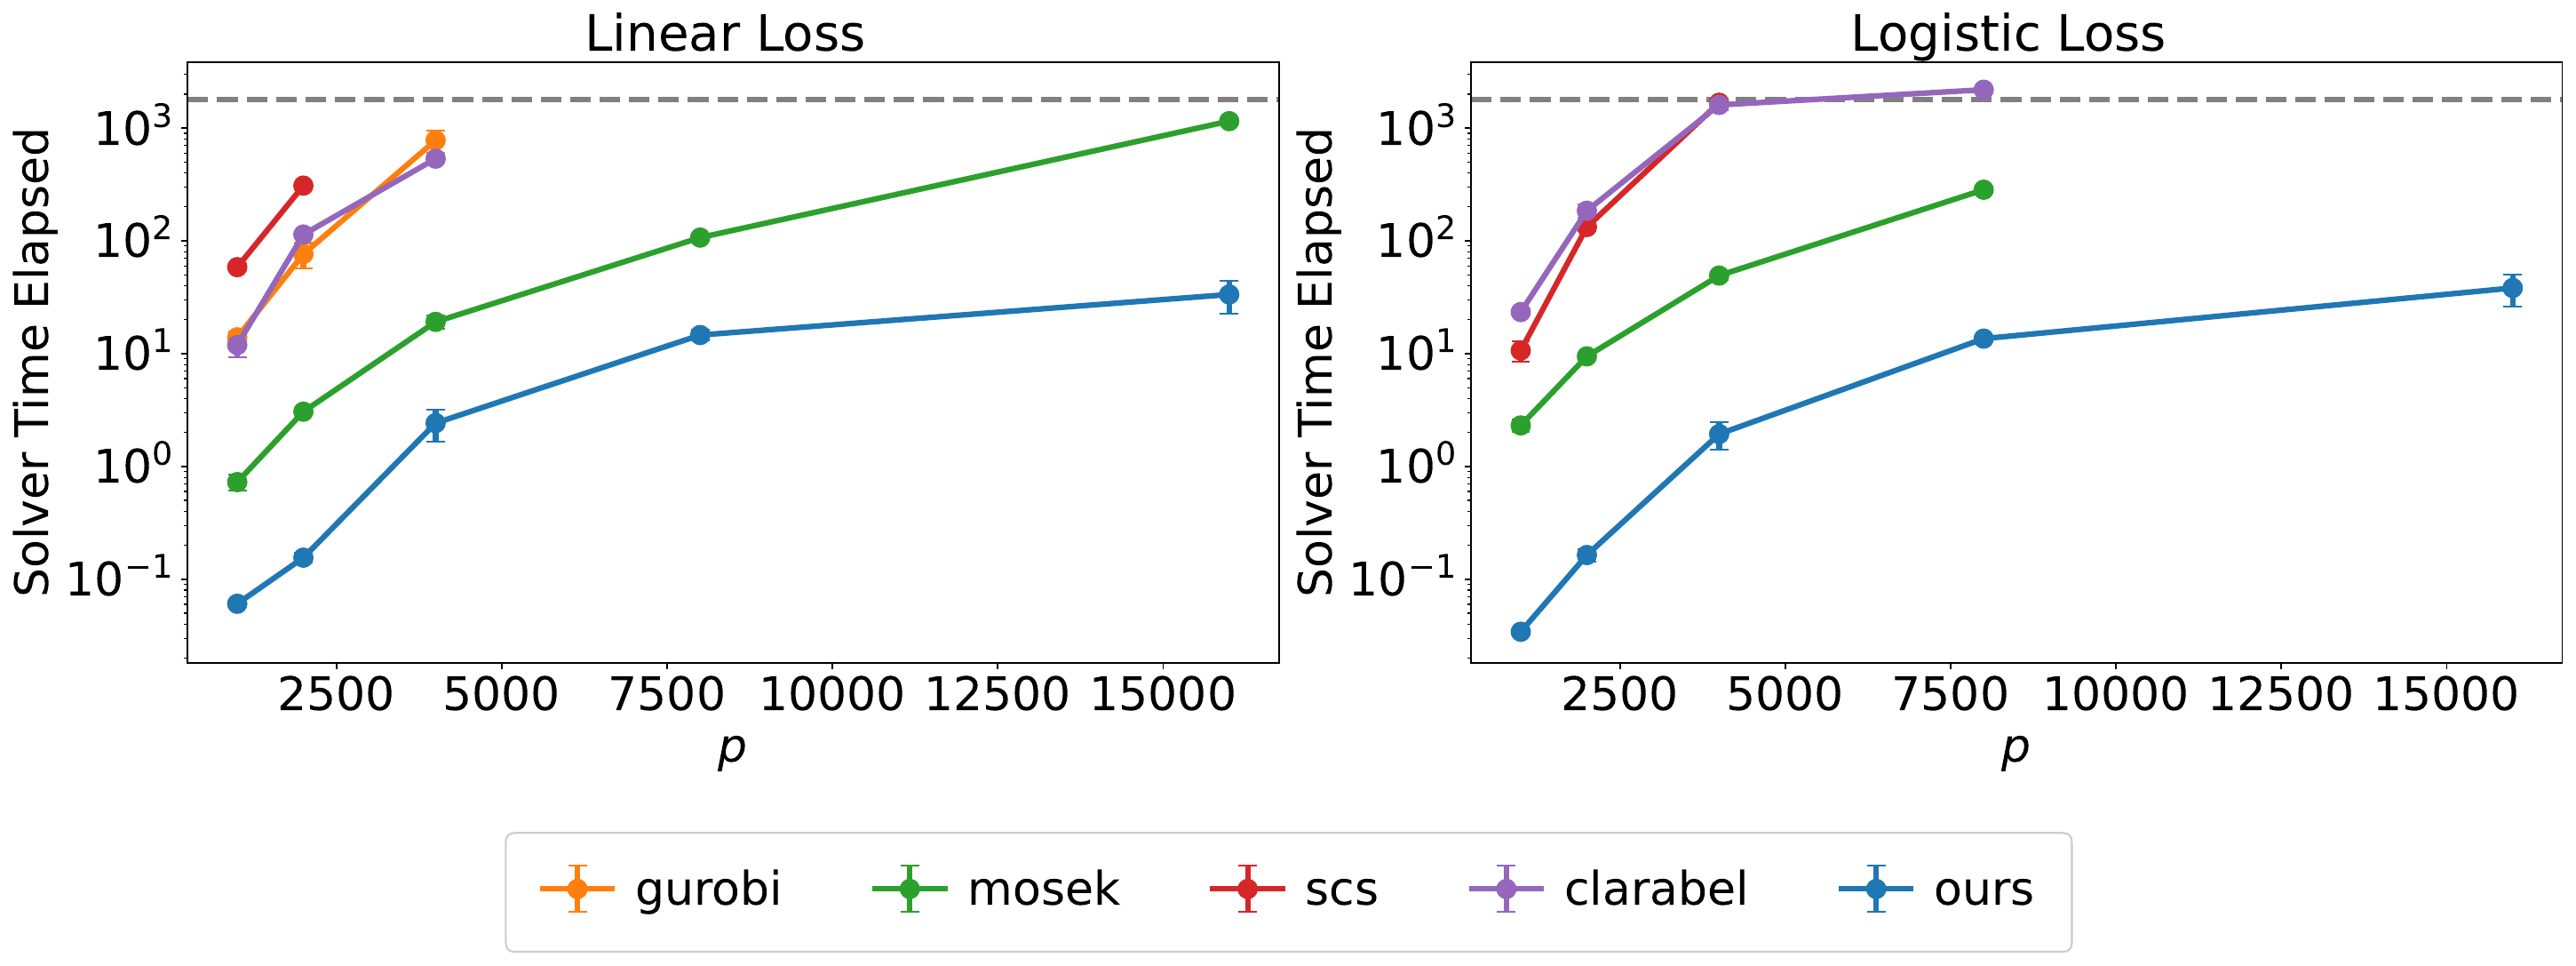}
    \caption{Running time comparison of solving Problem~\ref{obj:perspective_relaxation} with the $\ell_2$ regularization increased to $\lambda_2 = 10$.}
    \label{ec_fig:convex_relaxation_lambda2_10}
    \vspace{0em}
\end{figure}

\clearpage

\begin{figure}[!h]
    \centering
    \includegraphics[width=1.0\textwidth]{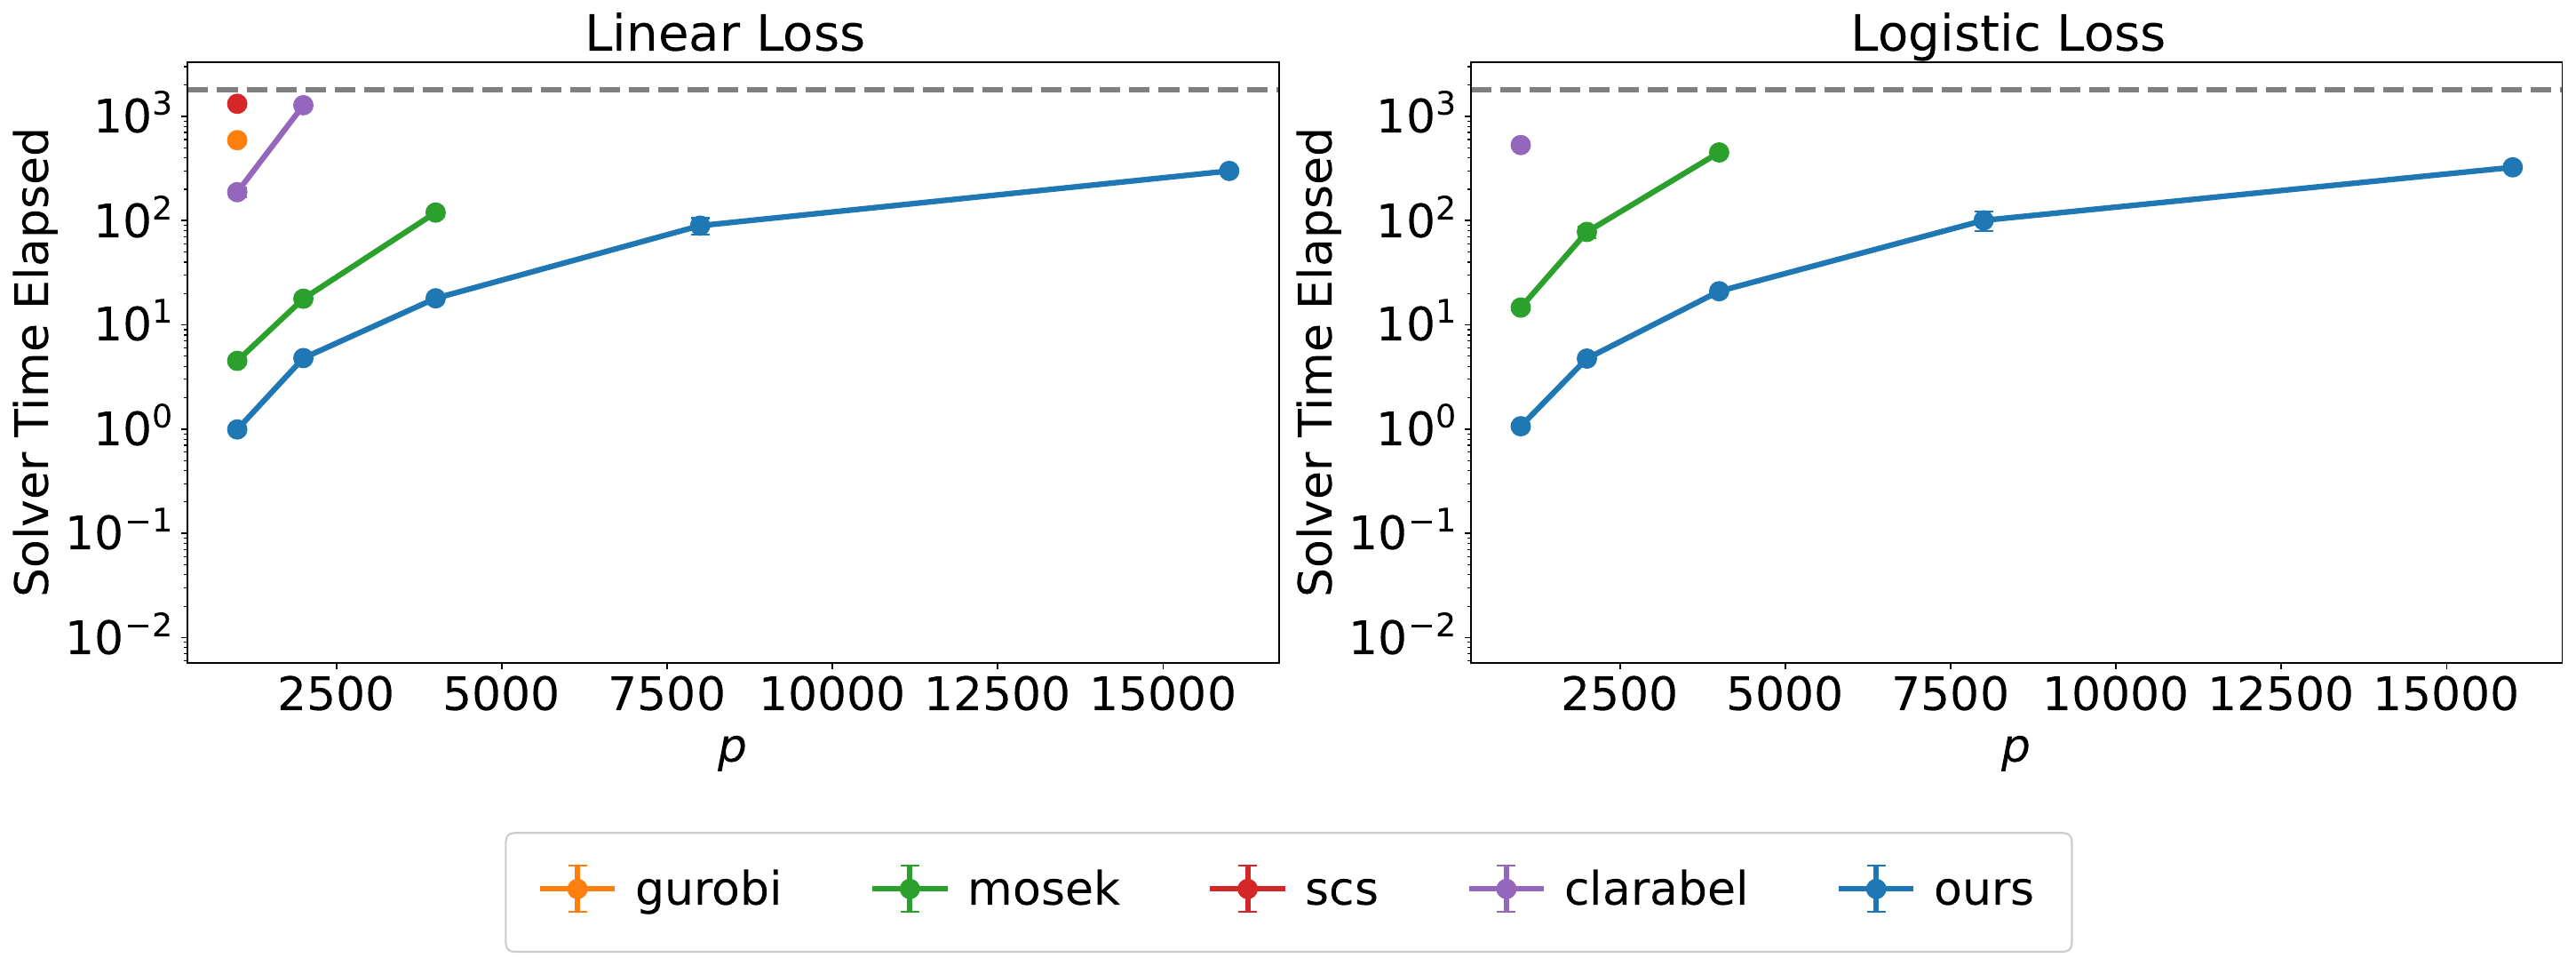}
    \caption{Running time comparison of solving Problem~\ref{obj:perspective_relaxation} when the $n$-to-$p$ ratio is increased to $10.0$.}
    \label{ec_fig:convex_relaxation_n_p_ratio_10.0}
    \vspace{0em}
\end{figure}

\begin{figure}[!h]
    \centering
    \includegraphics[width=1.0\textwidth]{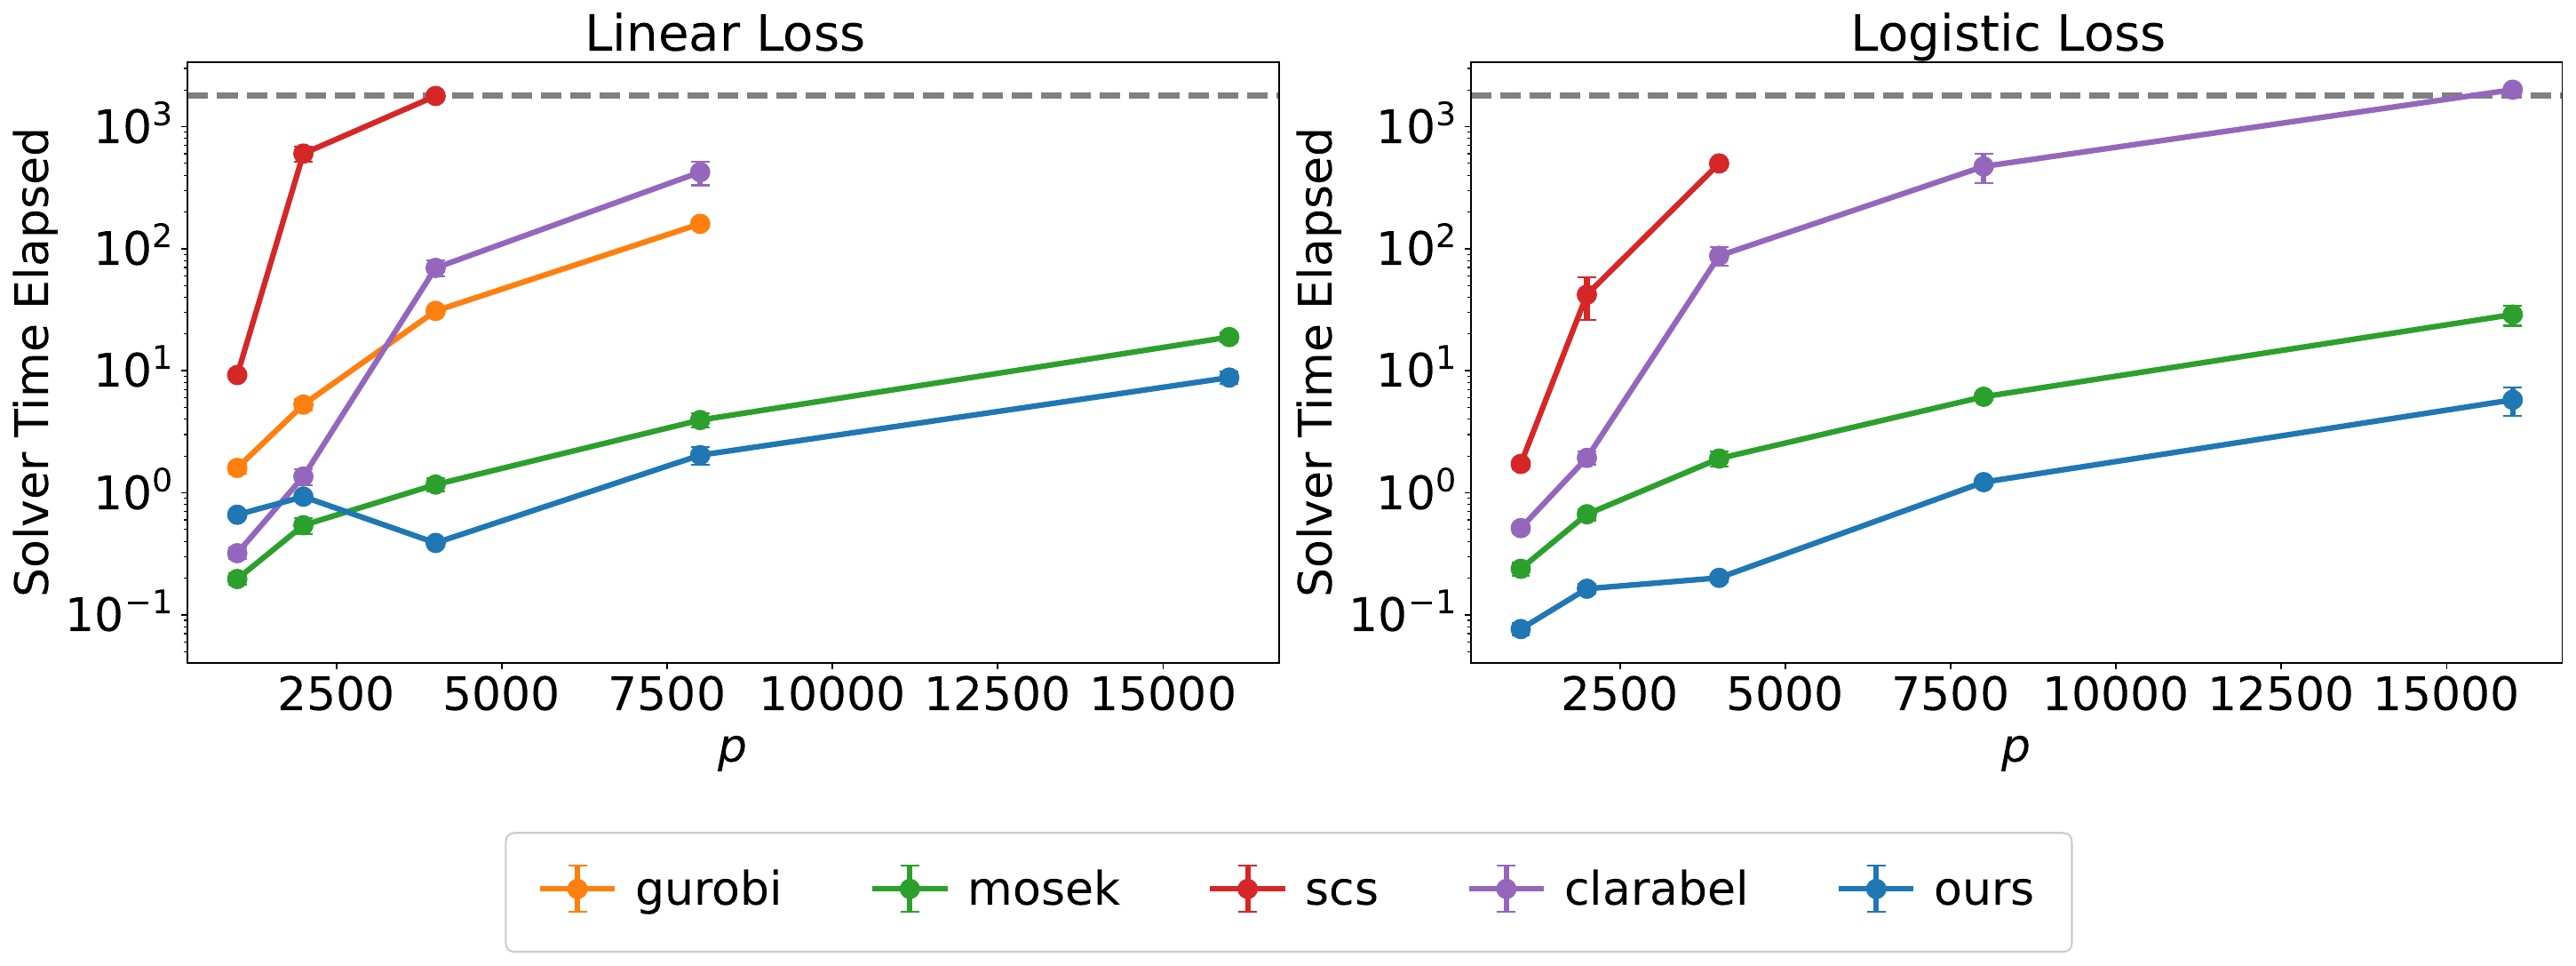}
    \caption{Running time comparison of solving Problem~\ref{obj:perspective_relaxation} when the $n$-to-$p$ ratio is decreased to $0.1$.}
    \label{ec_fig:convex_relaxation_n_p_ratio_0.1}
\end{figure}

\clearpage

\subsection{Shrink Factor in Duality-based Restart Scheme}
\label{ec_expt:shrink_factor_in_duality_based_restart_scheme}
In the main paper, we noted that the duality-based restart scheme can work with any decrease factor $\eta>1$, but the choice of $\eta$ affects practical running speed.
We compare $\eta \in \{e, e^2, e^3\}$ to illustrate this effect.
The results are shown in Figure~\ref{ec_fig:PDRestart_achieves_linear_convergence_rate_exponents_linear} and Figure~\ref{ec_fig:PDRestart_achieves_linear_convergence_rate_exponents_logistic}.
We are able to improve the practical speeds of all methods by changing $\eta$ from $e$ to $e^2$ and $e^3$, which matches the theoretical prediction in Theorem~\ref{theorem:optimal_restart_eta_choice} and discussion at the end of Section~\ref{subsec:restart_scheme}.

\begin{figure}[!h]
    \vspace{0em}
    \centering
    \includegraphics[width=1.0\textwidth]{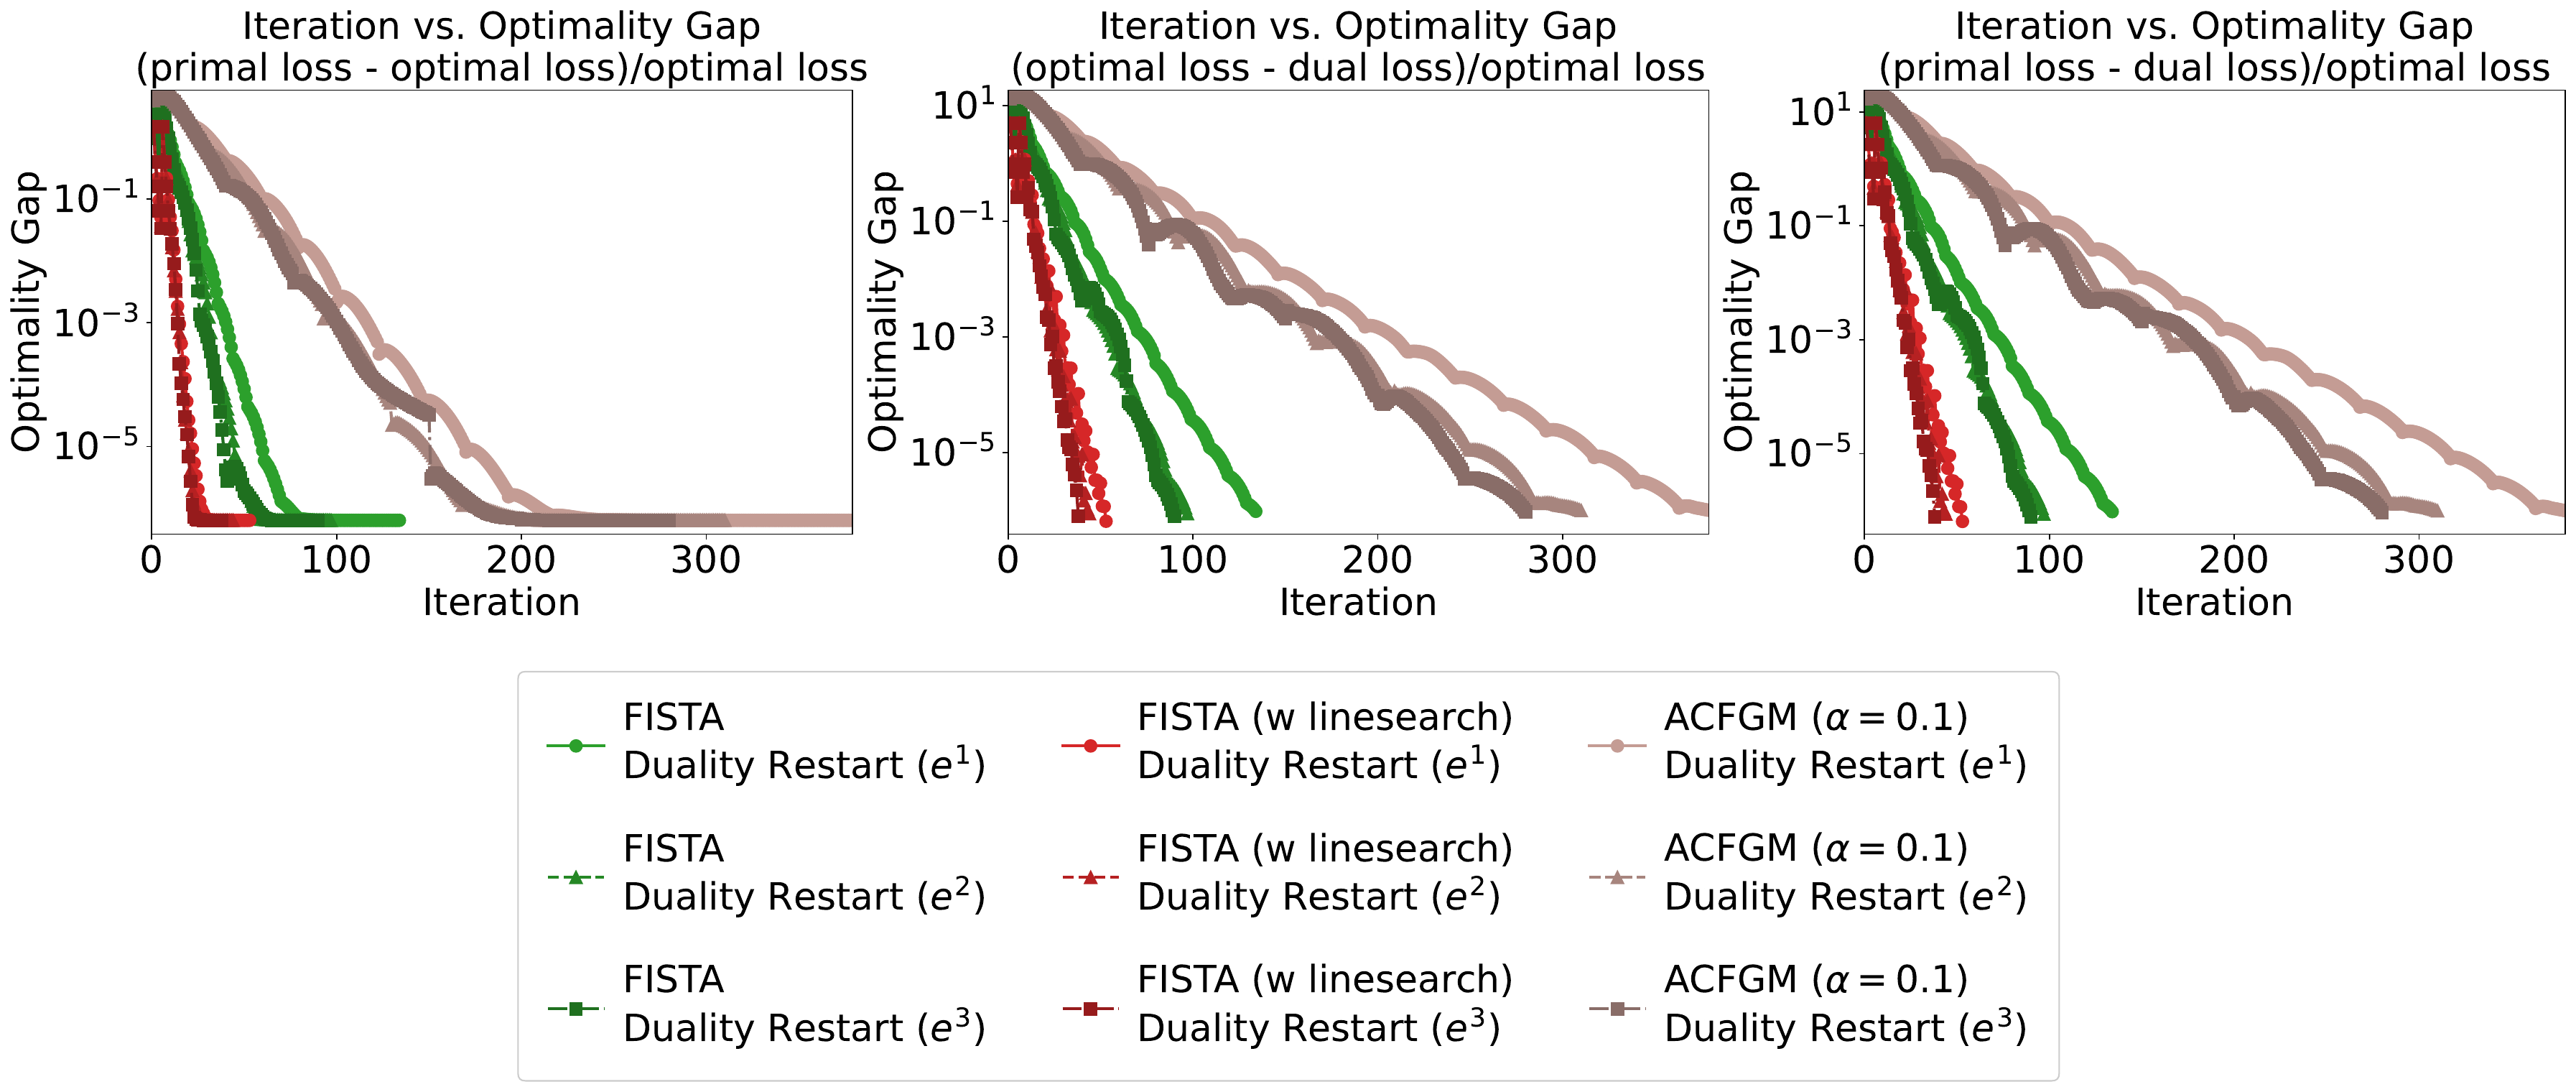}
    \caption{Convergence speed comparison of FISTA methods (with and without line search) and ACFGM (with duality-gap-based restarted ) for $\eta=e$, $\eta=e^2$, and $\eta=e^3$ on solving the perspective relaxation in Problem~\ref{obj:perspective_relaxation} with the linear regression loss, $n= 16000$, $p= 16000$, $k= 10$, $\rho= 0.5$, $\lambda_2 = 1.0$, and $M = 2.0$.}
    \label{ec_fig:PDRestart_achieves_linear_convergence_rate_exponents_linear}
    \vspace{0em}
\end{figure}

\begin{figure}[!h]
    \vspace{0em}
    \centering
    \includegraphics[width=1.0\textwidth]{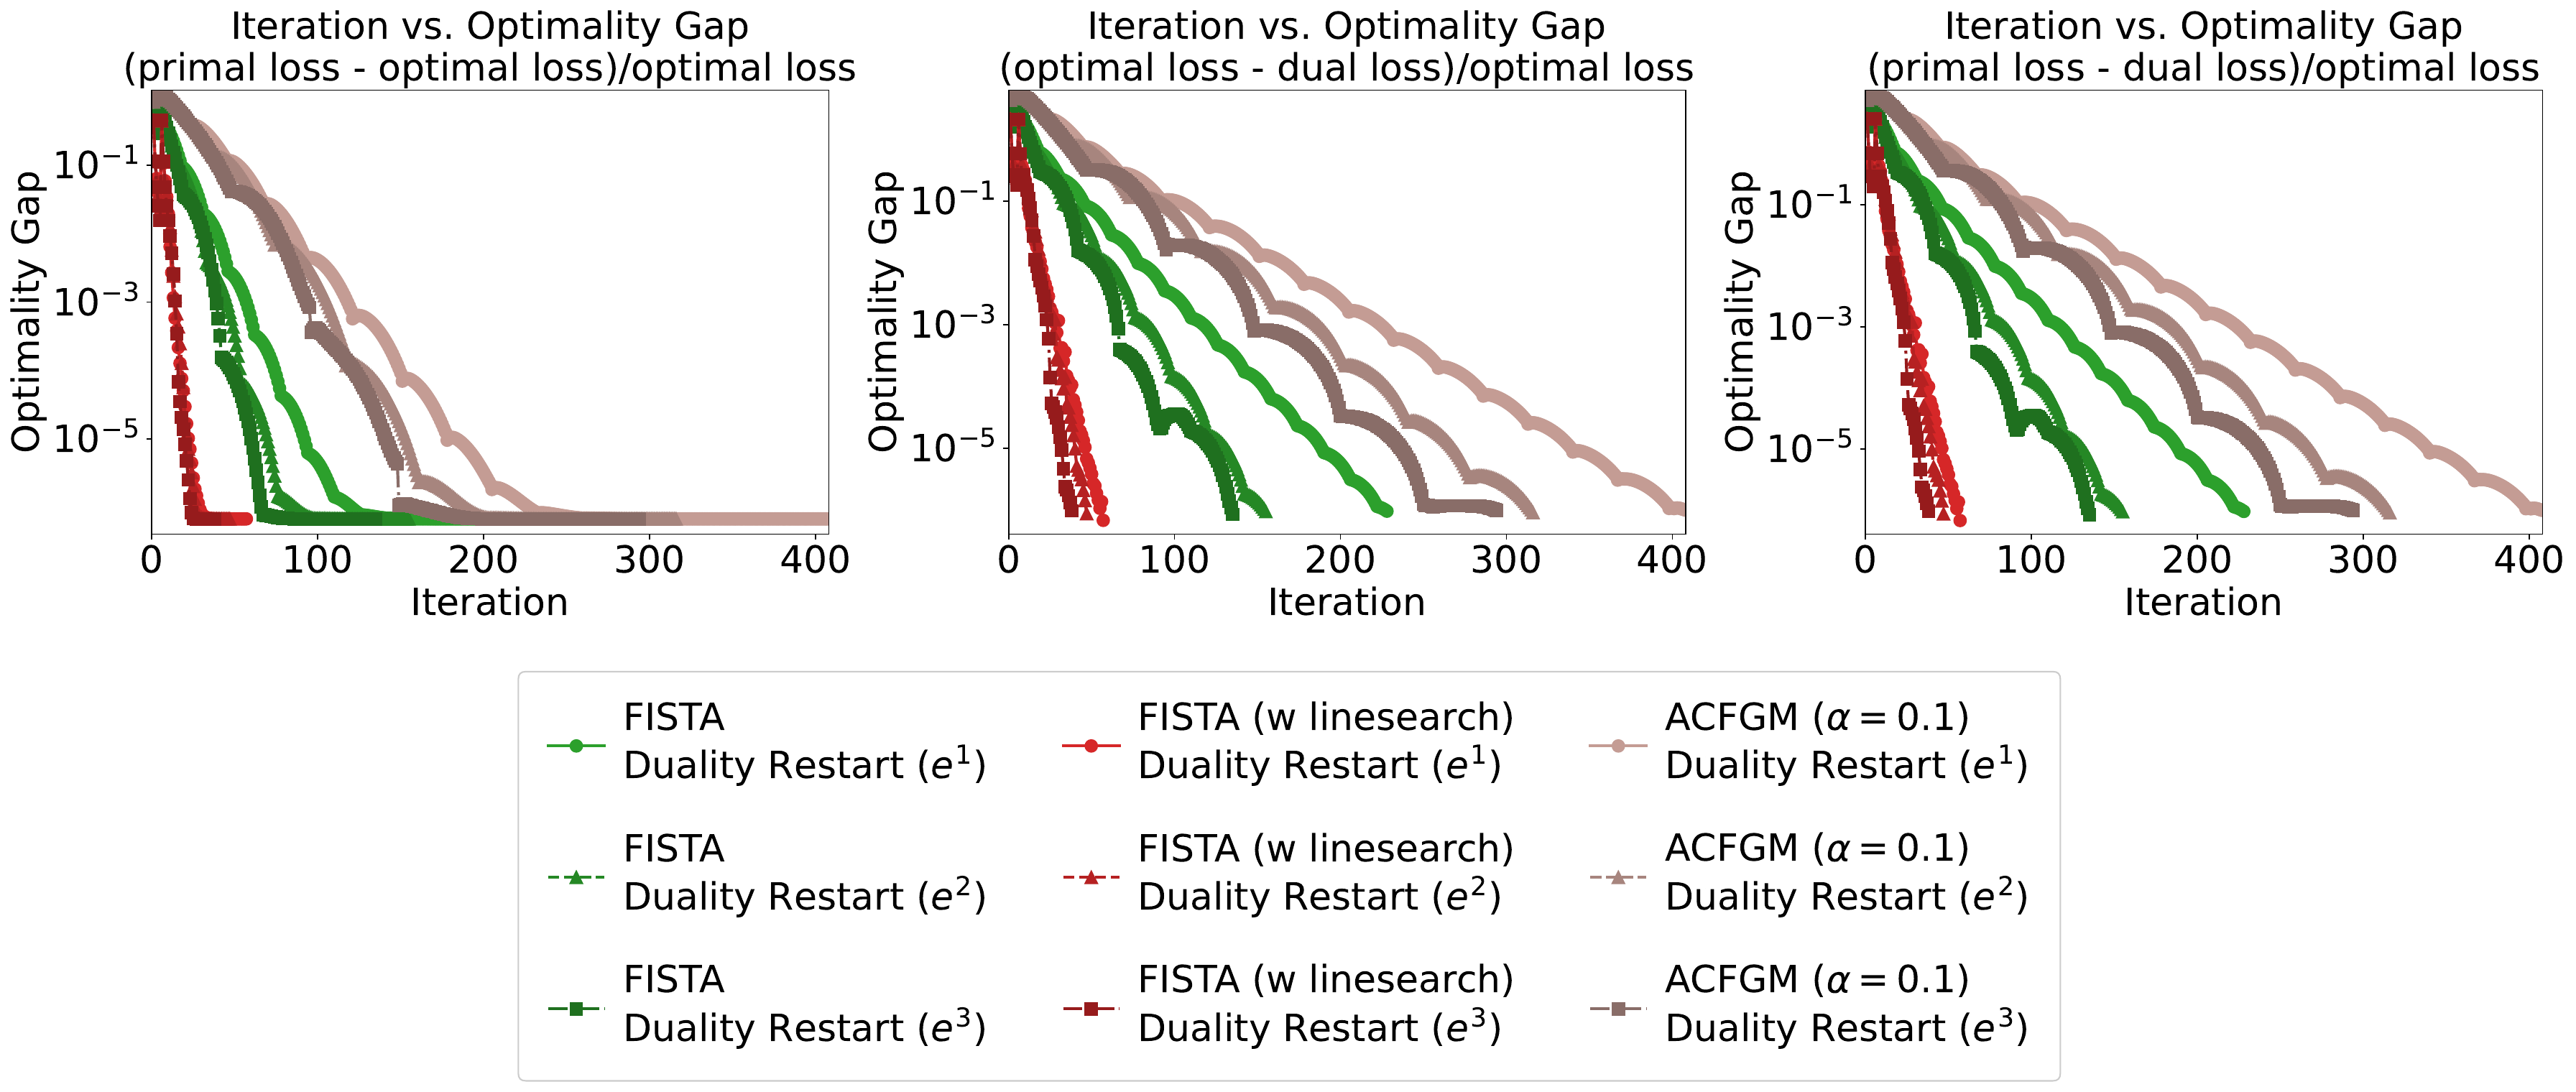}
    \caption{Convergence speed comparison of FISTA methods (with and without line search) and ACFGM (with duality-gap-based restarted ) for $\eta=e$, $\eta=e^2$, and $\eta=e^3$ on solving the perspective relaxation in Problem~\ref{obj:perspective_relaxation} with the logistic regression loss, $n= 16000$, $p= 16000$, $k= 10$, $\rho= 0.5$, $\lambda_2 = 1.0$, and $M = 2.0$.}
    \label{ec_fig:PDRestart_achieves_linear_convergence_rate_exponents_logistic}
\end{figure}

\clearpage
\subsection{Can Our Restart Scheme Benefit Other Problems Beyond Perspective Relaxations?}
\label{ec_expt:restart_beyond_perspective_relaxations}
To demonstrate the broader applicability of our duality-gap-based restart scheme beyond perspective relaxations, we apply it to accelerate proximal gradient methods for solving LASSO problems.
We report results for both an $\ell_1$-ball constrained formulation, where $G(\bbeta) := \delta_{\lVert \bbeta \rVert_1 \leq C}(\bbeta)$, and an $\ell_1$-regularized formulation, where $G(\bbeta) := \lambda_1 \lVert \bbeta \rVert_1$.
See Appendix~\ref{ec_expt:setup_for_restart_generality_lasso} for the experimental setup and parameter choices.
The results are shown in Figure~\ref{ec_fig:l1_constrained_linear_convergence}--Figure~\ref{ec_fig:l1_regularized_logistic_convergence}.
Like in the main paper for solving the perspective relaxation, we observe that our restart scheme accelerates both FISTA and ACFGM to achieve linear convergence rates.

\begin{figure}[!h]
    \centering
    \includegraphics[width=1.0\textwidth]{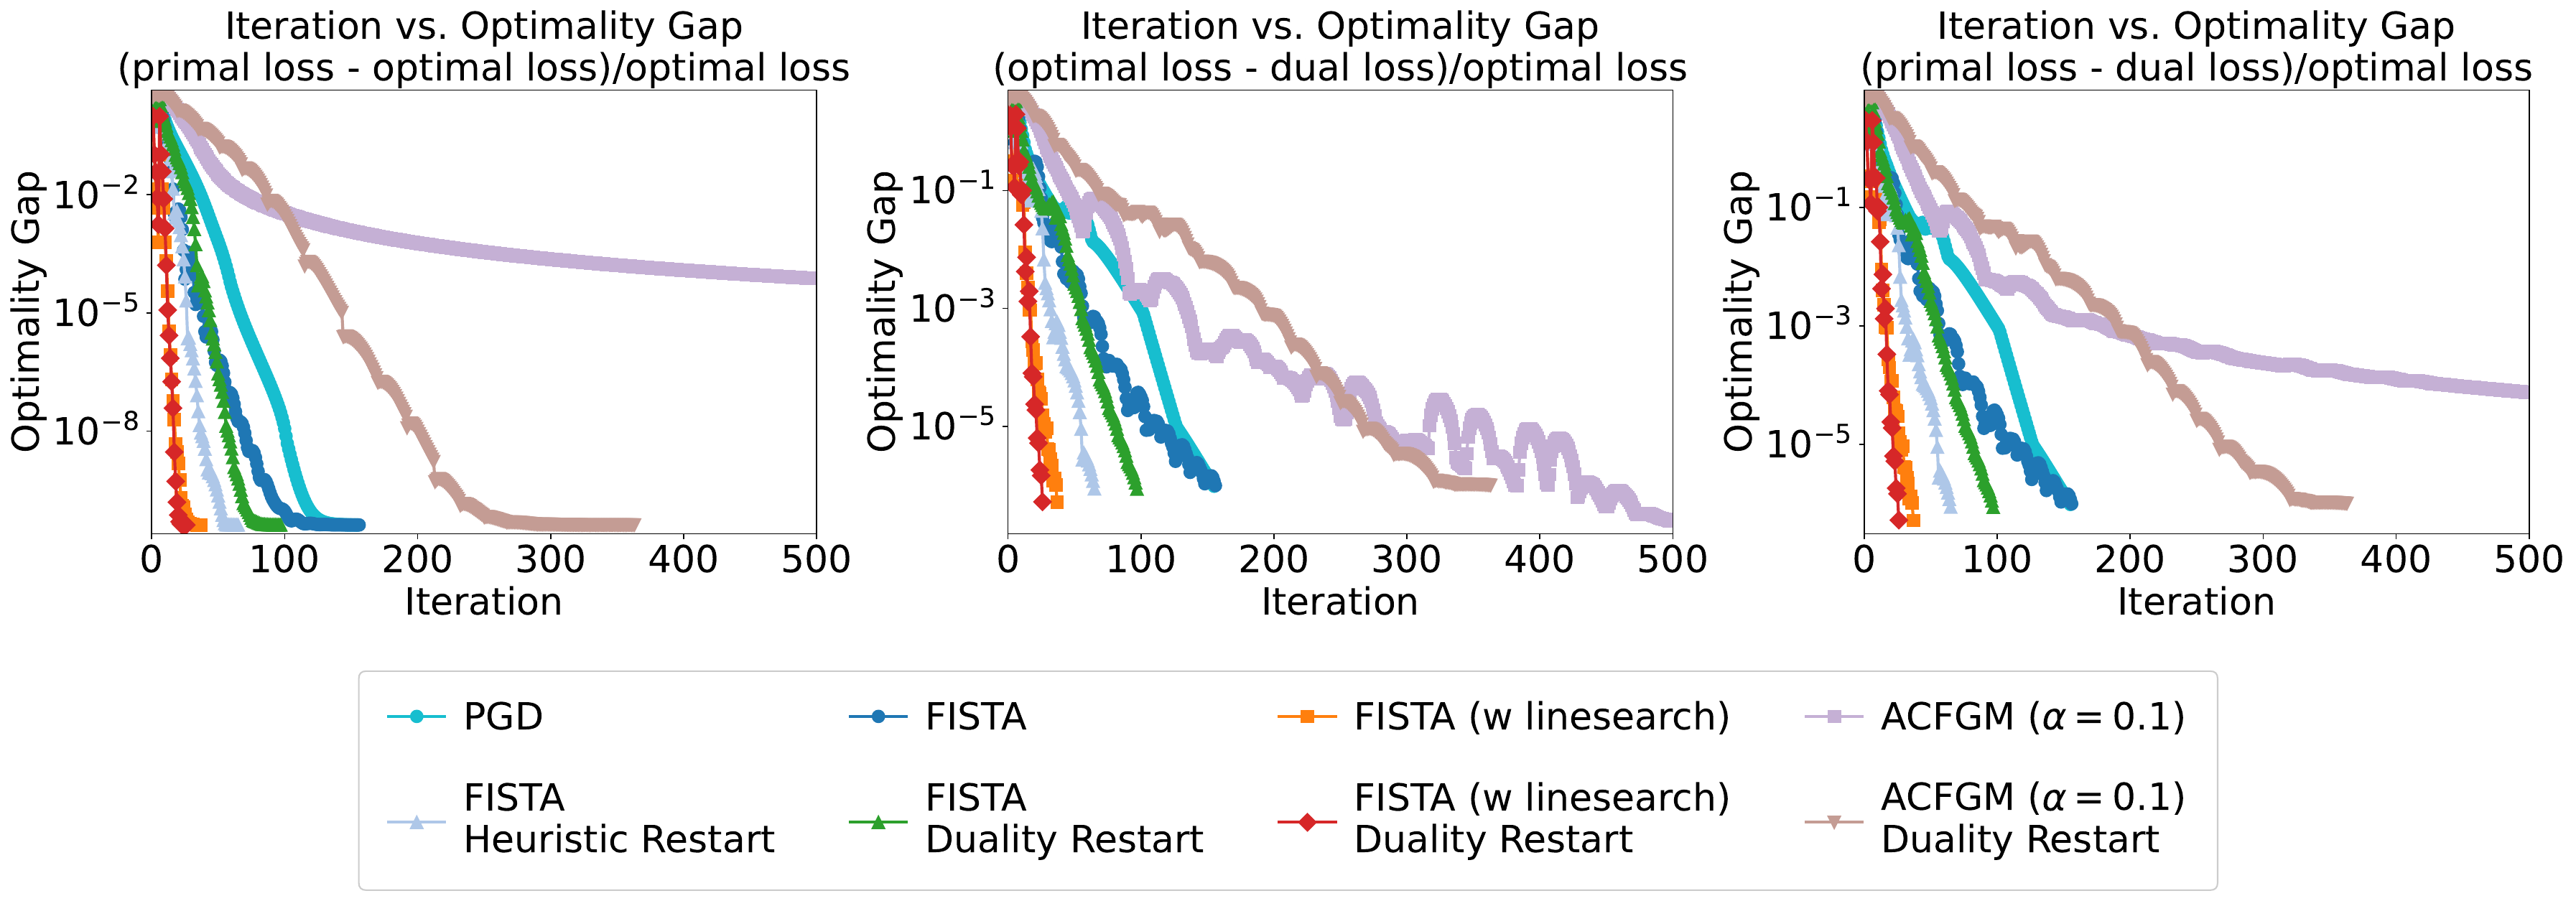}
    \caption{Convergence speed comparison between accelerated methods (with and without restart), on solving the $\ell_1$-ball constrained problem with the least squares loss.}
    \label{ec_fig:l1_constrained_linear_convergence}
    \vspace{0em}
\end{figure}

\begin{figure}[!h]
    \centering
    \includegraphics[width=1.0\textwidth]{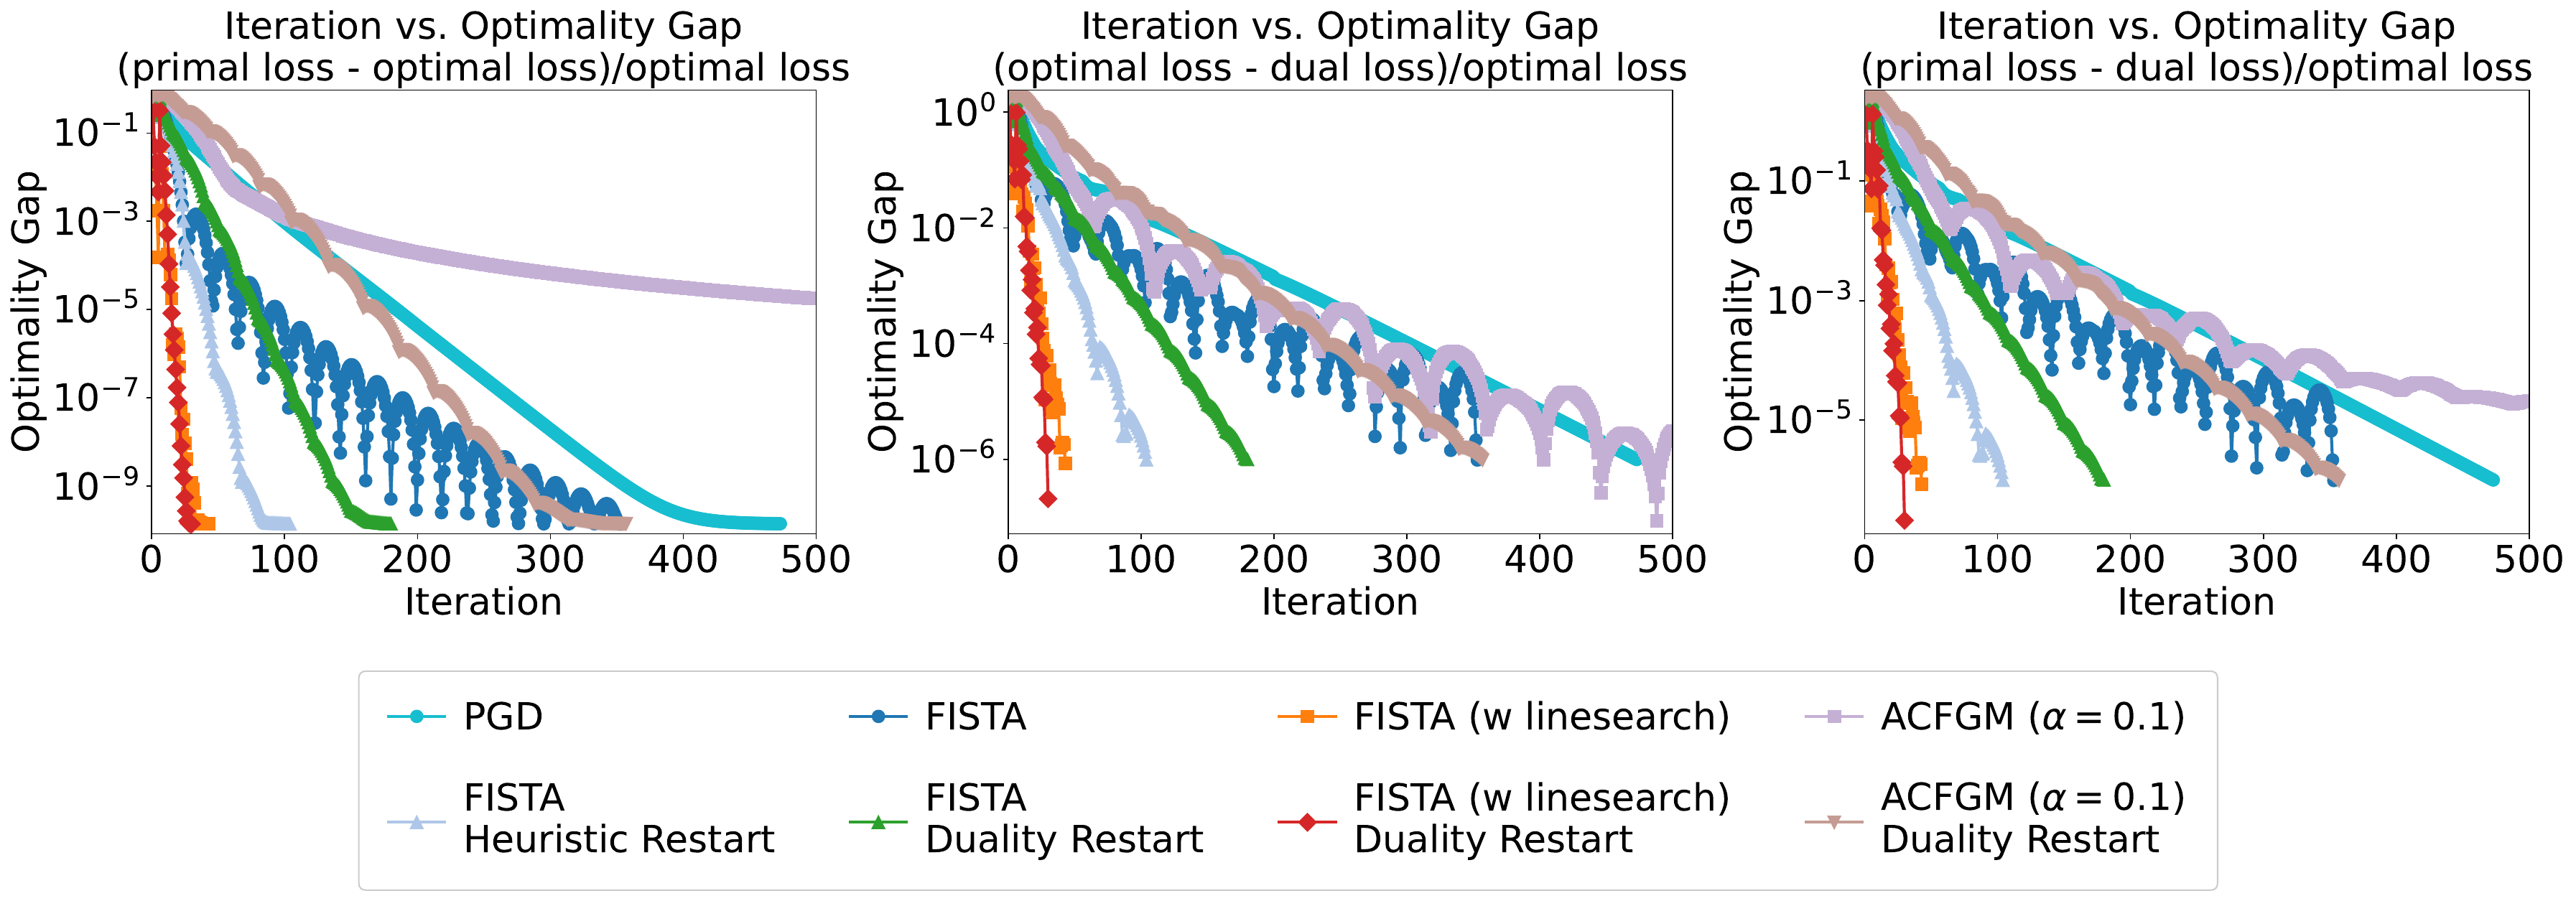}
    \caption{Convergence speed comparison between accelerated methods (with and without restart), on solving the $\ell_1$-ball constrained problem with the logistic regression loss.}
    \label{ec_fig:l1_constrained_logistic_convergence}
    \vspace{0em}
\end{figure}

\paragraph{Dual feasibility for $\ell_1$-regularized problems.}
For the $\ell_1$-regularized formulation, the Fenchel conjugate of the regularization term $G(\bbeta) = \lambda_1 \lVert \bbeta \rVert_1$ is $G^*(\bu) = \delta_{\lVert \bu \rVert_\infty \le \lambda_1}(\bu)$, and hence the dual objective is finite only when $\lVert \bX^\top \bzeta \rVert_\infty \le \lambda_1$.
Thus, the dual sequence $\bzeta^t := - \nabla F \left( \bX \bbeta^t \right)$ can be infeasible, in which case evaluating the dual objective is not meaningful.
Following standard practice in the LASSO literature, we enforce dual feasibility via a simple scaling (radial projection) step,
$\widehat{\bzeta} := \bzeta \cdot \min\!\left\{1,\ \frac{\lambda_1}{\lVert \bX^\top \bzeta \rVert_\infty}\right\}$,
which guarantees $\lVert \bX^\top \widehat{\bzeta} \rVert_\infty \le \lambda_1$ and yields a valid (though potentially loose) dual lower bound for computing a duality gap \citep{fercoq2015mind,dantas2021expanding}.
As a result, when applying our gap-based restart scheme to $\ell_1$-regularized problems, the gap used for restarting should be viewed as an inexact certificate; nevertheless, it still provides an effective restart signal in practice, leading to the linear-convergence behavior observed below.

\begin{figure}[!h]
    \centering
    \includegraphics[width=1.0\textwidth]{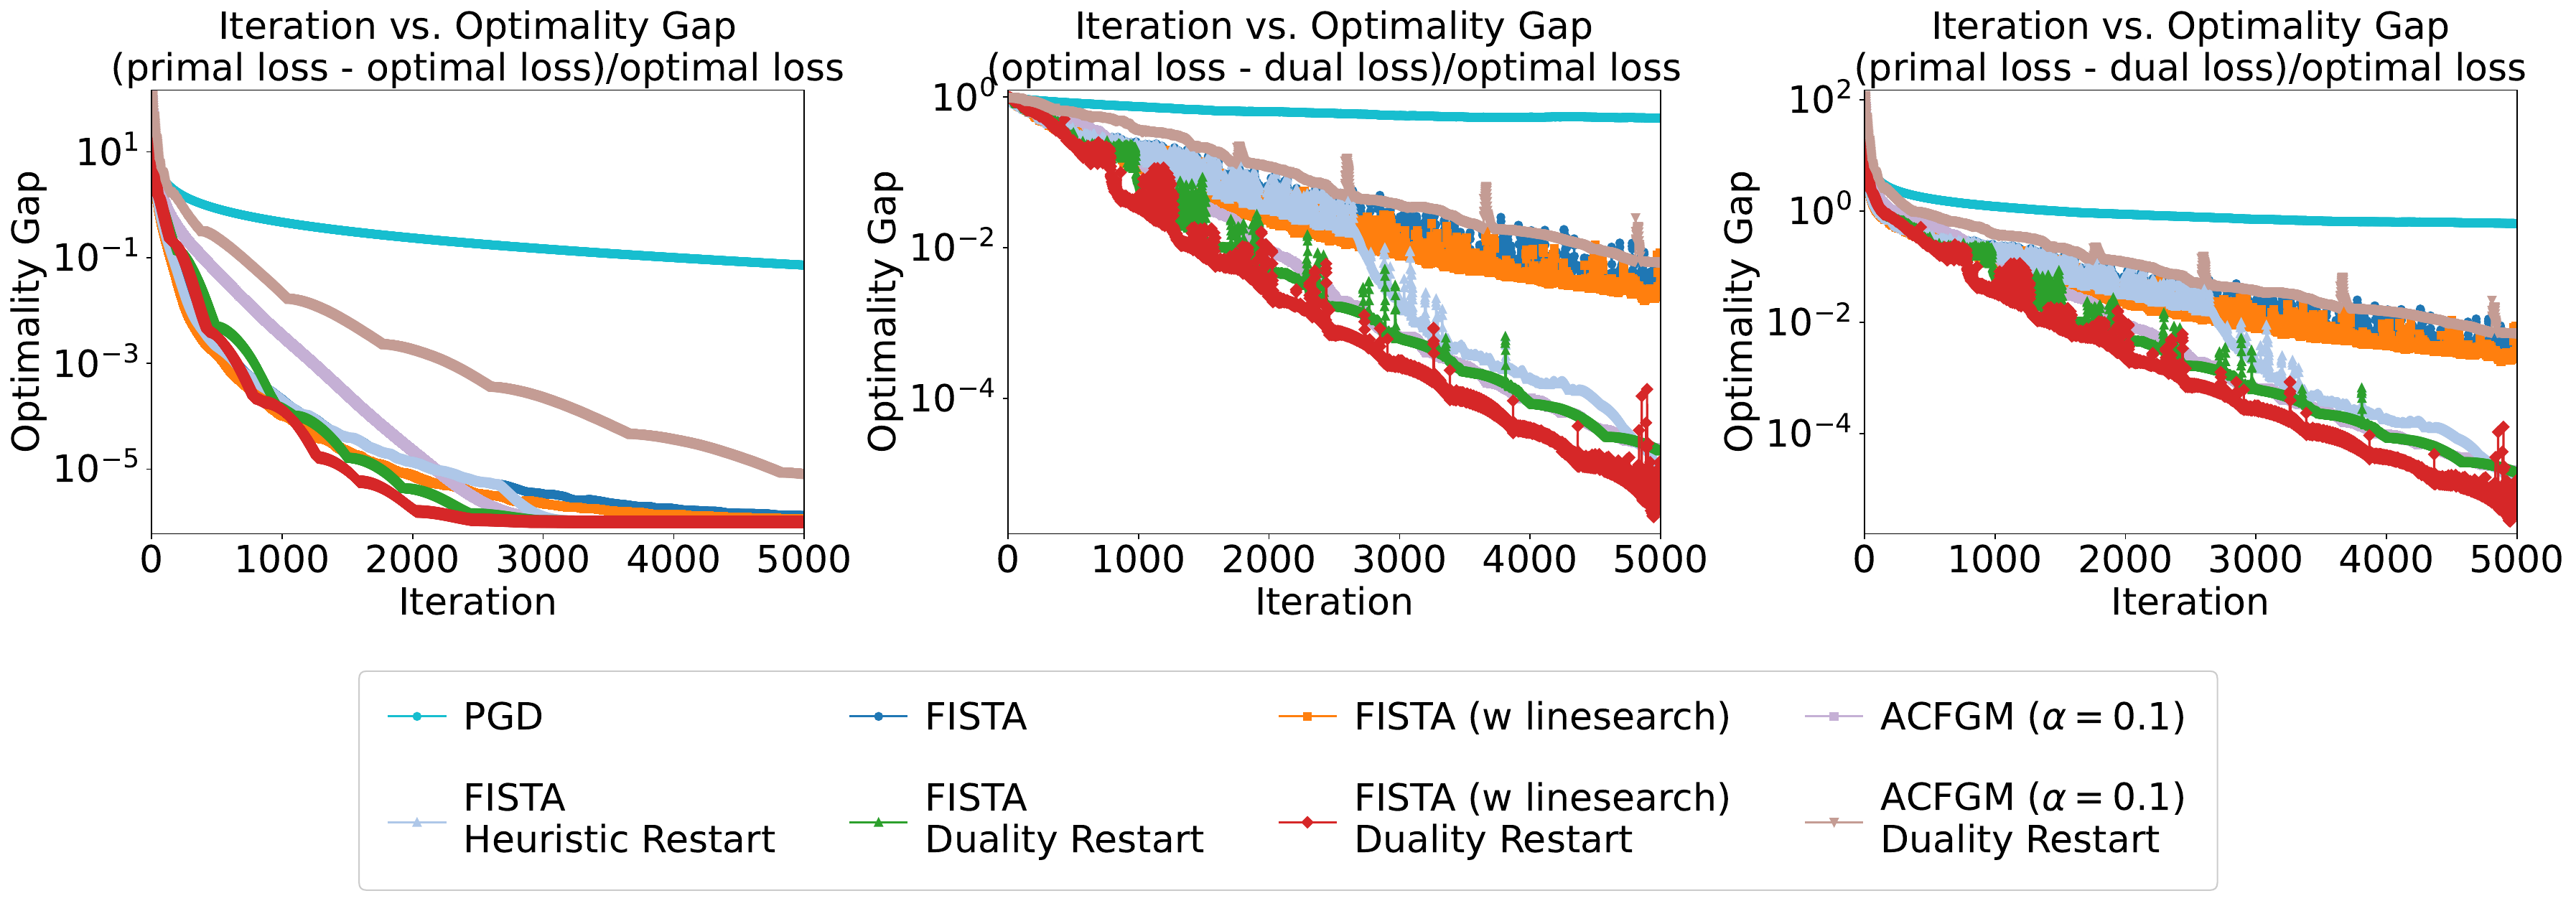}
    \caption{Convergence speed comparison between accelerated methods (with and without restart), on solving the $\ell_1$-regularized problem with the least squares loss.}
    \label{ec_fig:l1_regularized_linear_convergence}
    \vspace{0em}
\end{figure}

\begin{figure}[!h]
    \centering
    \includegraphics[width=1.0\textwidth]{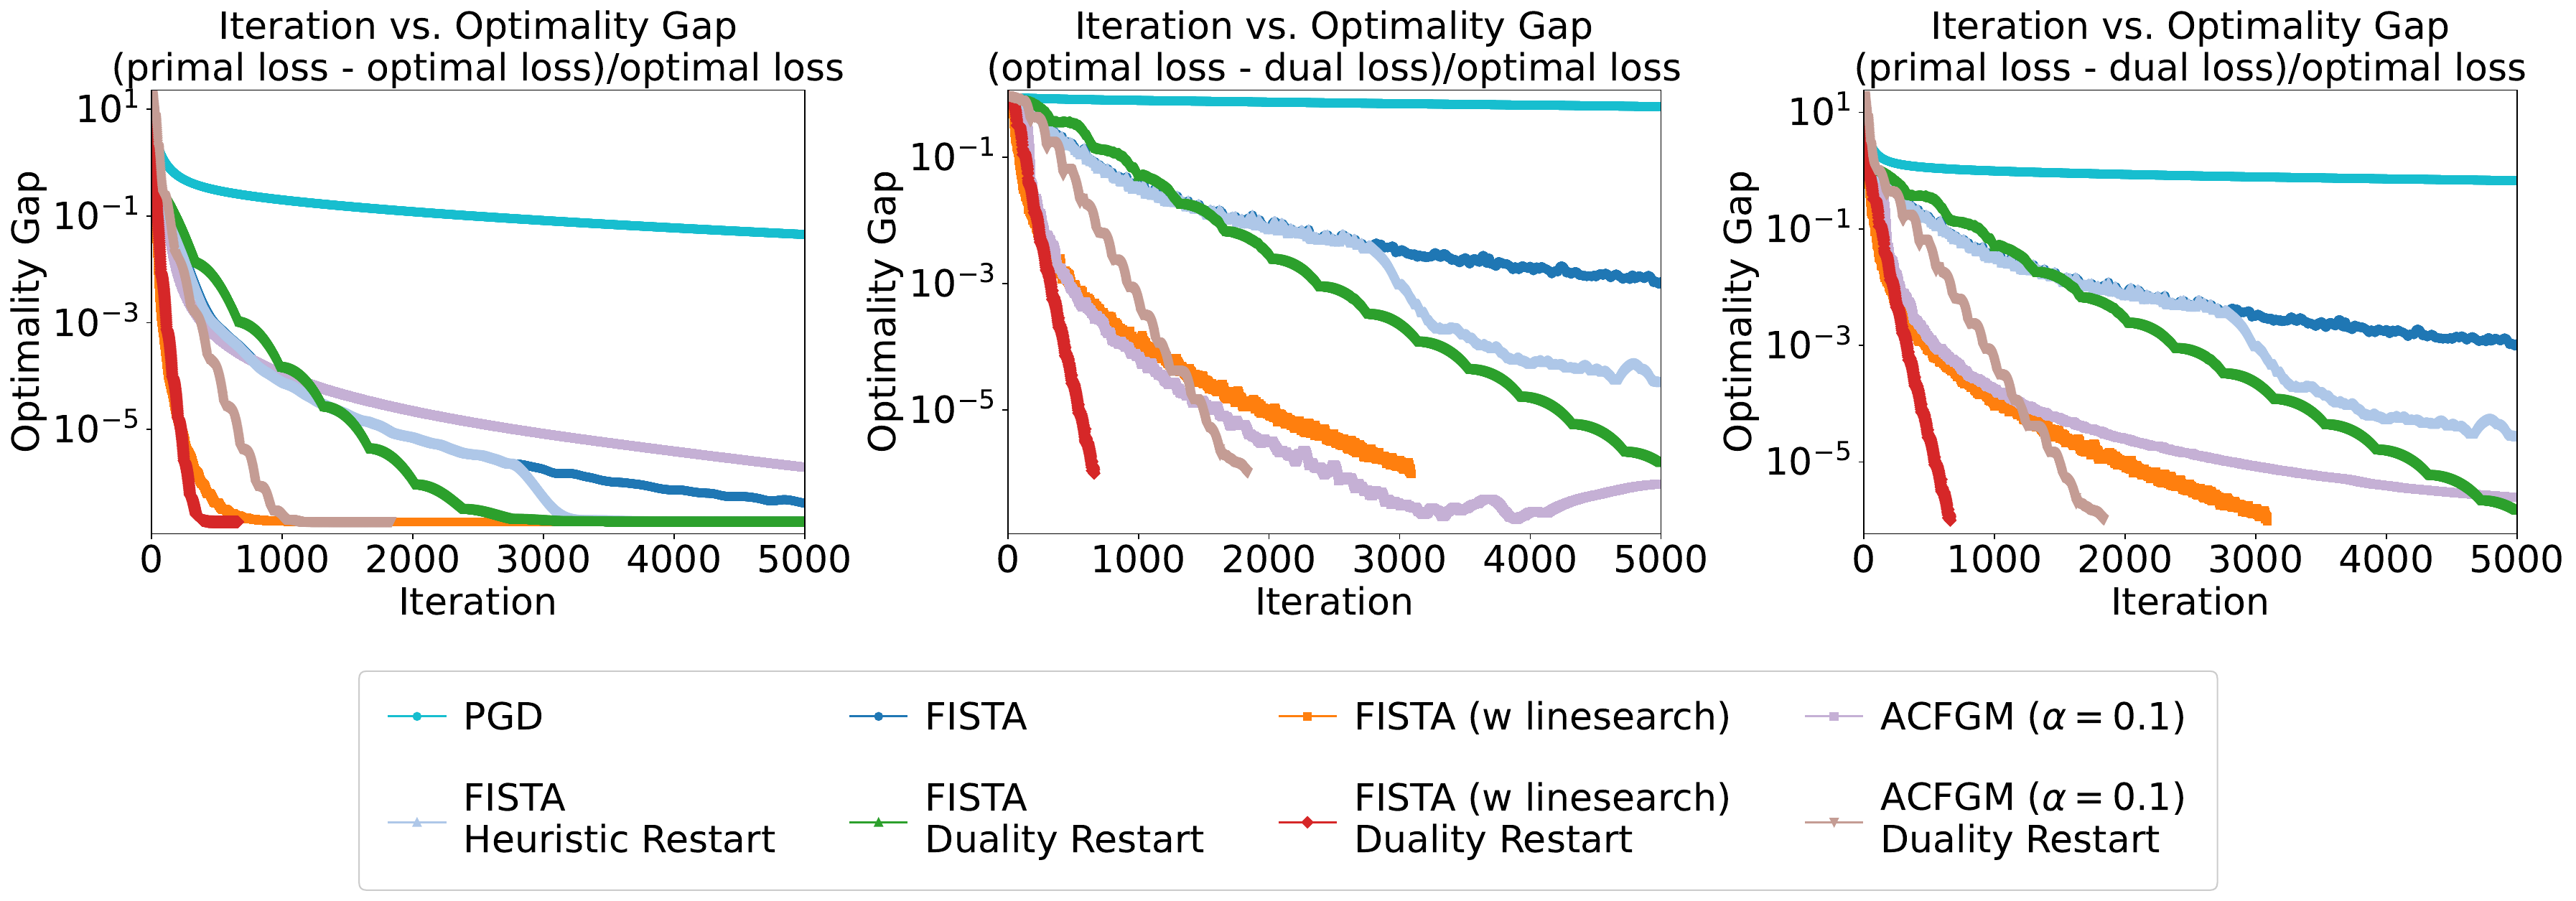}
    \caption{Convergence speed comparison between accelerated methods (with and without restart), on solving the $\ell_1$-regularized problem with the logistic regression loss.}
    \label{ec_fig:l1_regularized_logistic_convergence}
\end{figure}

\clearpage
\subsection{Certifying Optimality}
\label{ec_expt:additional_results_on_certifying_optimality}

\subsubsection{Synthetic Results with $M=3$}
We report additional branch-and-bound results on the synthetic datasets with a larger box constraint $M=3.0$: CPU baselines in Tables~\ref{tab:bnb_linear_M3}--\ref{tab:bnb_logistic_M3} and CPU vs GPU comparisons in Tables~\ref{tab:bnb_gpu_linear_M3}--\ref{tab:bnb_gpu_logistic_M3}.

% Branch-and-bound results for linear regression (M=3)
% Metadata: rows are p-values; columns grouped by method (ours, gurobi, mosek), each with time (0-decimal, TL shown for time>=7200 with LB in parentheses for ours), gap (\% to two decimals; any nonzero gap <0.005 shown as 0.01), and \# nodes; no vertical rules (OPRE); trimmed horizontal rules under method headers; numeric entries rounded accordingly with "-" for unavailable; caption lists k, rho, lambda2, M, and n/p=1.0 (assumed); source is sections/Tables/raw_txt/011825/plots_BnB_synthetic/print_BnB_synthetic.txt for k=10, rho=0.5, lambda2=1.0, M=3.0; method mapping: ours = beamsize5+ourspdrestartedbeckfistalinesearche3; gurobi = gurobinativewarmstart; mosek = moseknativewarmstart; for ours, time shows total time with LB time in parentheses; display names omit "w/ warmstart" while values are from warmstarted baselines; caption notes OOM and TL=7200s when present.
\begin{table}[!ht]
\vspace{0em}
\centering
\caption{BnB results on synthetic (linear) with $k=10$, $\rho=0.5$, $\lambda_2=1.0$, $M=3.0$, $n/p=1.0$. Parentheses show lower-bound time. OOM = out of memory, TL = time $> 7200$s.}
\label{tab:bnb_linear_M3}
\resizebox{1.0\linewidth}{!}{%
\begin{tabular}{rccc ccc ccc}
\hline
 & \multicolumn{3}{c}{ours} & \multicolumn{3}{c}{gurobi} & \multicolumn{3}{c}{mosek} \\
\cmidrule(l{0.8em}r{0.8em}){2-4}\cmidrule(l{0.8em}r{0.8em}){5-7}\cmidrule(l{0.8em}r{0.8em}){8-10}
$p$ & time(s) & gap(\%) & \# nodes & time(s) & gap(\%) & \# nodes & time(s) & gap(\%) & \# nodes \\ \hline
1000 & 31 (3) & 0.00 & 355 & 227 & 0.00 & 653 & 208 & 0.00 & 361 \\
2000 & 16 (2) & 0.00 & 161 & 2091 & 0.00 & 1544 & 758 & 0.00 & 171 \\
4000 & 27 (15) & 0.00 & 77 & 4574 & 0.00 & 97 & 3612 & 0.00 & 73 \\
8000 & 63 (45) & 0.00 & 49 & TL & 100.00 & 1 & TL & 33.57 & 4 \\
16000 & 151 (115) & 0.00 & 33 & TL & 100.00 & 1 & OOM & OOM & OOM \\
\hline
\end{tabular}%
}
\vspace{0em}
\end{table}

% Branch-and-bound results for logistic regression (M=3)
% Metadata: rows are p-values; columns grouped by method (ours, gurobiOA, mosek), each with time (0-decimal, TL shown for time>=7200 with LB in parentheses for ours), gap (\% to two decimals; any nonzero gap <0.005 shown as 0.01), and \# nodes; no vertical rules (OPRE); trimmed horizontal rules under method headers; numeric entries rounded accordingly with "-" for unavailable; caption lists k, rho, lambda2, M, and n/p=1.0 (assumed); source is sections/Tables/raw_txt/011825/plots_BnB_synthetic/print_BnB_synthetic.txt for k=10, rho=0.5, lambda2=1.0, M=3.0; method mapping: ours = beamsize5+ourspdrestartedbeckfistalinesearche3; gurobiOA = gurobinativeoawarmstart; mosek = moseknativewarmstart; for ours, time shows total time with LB time in parentheses; display names omit "w/ warmstart" while values are from warmstarted baselines; caption notes OOM and TL=7200s when present.
\begin{table}[!ht]
\vspace{0em}
\centering
\caption{BnB results on synthetic (logistic) with $k=10$, $\rho=0.5$, $\lambda_2=1.0$, $M=3.0$, $n/p=1.0$. Parentheses show lower-bound time. OOM = out of memory, TL = time $> 7200$s.}
\label{tab:bnb_logistic_M3}
\resizebox{1.0\linewidth}{!}{%
\begin{tabular}{rccc ccc ccc}
\hline
 & \multicolumn{3}{c}{ours} & \multicolumn{3}{c}{gurobiOA} & \multicolumn{3}{c}{mosek} \\
\cmidrule(l{0.8em}r{0.8em}){2-4}\cmidrule(l{0.8em}r{0.8em}){5-7}\cmidrule(l{0.8em}r{0.8em}){8-10}
$p$ & time(s) & gap(\%) & \# nodes & time(s) & gap(\%) & \# nodes & time(s) & gap(\%) & \# nodes \\ \hline
1000 & 771 (37) & 0.00 & 6049 & TL & 67.29 & 417432 & 1871 & 0.00 & 5847 \\
2000 & 630 (81) & 0.00 & 3451 & TL & 87.29 & 443958 & 7031 & 0.00 & 3427 \\
4000 & 384 (168) & 0.00 & 855 & TL & 82.12 & 269137 & TL & 13.97 & 569 \\
8000 & 666 (404) & 0.00 & 459 & TL & 69.86 & 93806 & OOM & OOM & OOM \\
16000 & 1031 (677) & 0.00 & 207 & TL & 56.55 & 35414 & OOM & OOM & OOM \\
\hline
\end{tabular}%
}
\vspace{0em}
\end{table}

% BnB GPU vs CPU results for linear regression (M=3)
% Metadata: rows are p-values; columns grouped by method (ours CPU, ours GPU), each with time (0-decimal, TL shown for time>=7200 with LB time in parentheses), gap (% to two decimals; any nonzero gap <0.005 shown as 0.01), and # nodes; no vertical rules (OPRE); trimmed horizontal rules under method headers; numeric entries rounded accordingly with "-" for unavailable; caption lists k, rho, lambda2, M, and n/p=1.0 (assumed); source is sections/Tables/raw_txt/011825/plots_BnB_synthetic_GPU/print_BnB_synthetic_GPU.txt for k=10, rho=0.5, lambda2=1.0, M=3.0; method mapping: ours CPU = beamsize5+ourspdrestartedbeckfistalinesearche3, ours GPU = beamsize5+oursgpupdrestartedbeckfistalinesearche3.
\begin{table}[!ht]
\centering
\caption{BnB CPU vs GPU results for linear regression with $k=10$, $\rho=0.5$, $\lambda_2=1.0$, $M=3.0$, $n/p=1.0$. Parentheses show lower-bound time.}
\label{tab:bnb_gpu_linear_M3}
\resizebox{0.7\linewidth}{!}{%
\begin{tabular}{rccc ccc}
\hline
 & \multicolumn{3}{c}{ours CPU} & \multicolumn{3}{c}{ours GPU} \\
\cmidrule(l{0.8em}r{0.8em}){2-4}\cmidrule(l{0.8em}r{0.8em}){5-7}
$p$ & time(s) & gap(\%) & \# nodes & time(s) & gap(\%) & \# nodes \\ \hline
1000 & 29 (2) & 0.00 & 355 & 36 (9) & 0.00 & 355 \\
2000 & 15 (2) & 0.00 & 161 & 18 (4) & 0.00 & 161 \\
4000 & 12 (4) & 0.00 & 77 & 9 (2) & 0.00 & 77 \\
8000 & 44 (30) & 0.00 & 49 & 15 (2) & 0.00 & 49 \\
16000 & 78 (53) & 0.00 & 33 & 26 (4) & 0.00 & 33 \\
\hline
\end{tabular}%
}
\end{table}

% BnB GPU vs CPU results for logistic regression (M=3)
% Metadata: rows are p-values; columns grouped by method (ours CPU, ours GPU), each with time (0-decimal, TL shown for time>=7200 with LB time in parentheses), gap (% to two decimals; any nonzero gap <0.005 shown as 0.01), and # nodes; no vertical rules (OPRE); trimmed horizontal rules under method headers; numeric entries rounded accordingly with "-" for unavailable; caption lists k, rho, lambda2, M, and n/p=1.0 (assumed); source is sections/Tables/raw_txt/011825/plots_BnB_synthetic_GPU/print_BnB_synthetic_GPU.txt for k=10, rho=0.5, lambda2=1.0, M=3.0; method mapping: ours CPU = beamsize5+ourspdrestartedbeckfistalinesearche3, ours GPU = beamsize5+oursgpupdrestartedbeckfistalinesearche3.
\begin{table}[!ht]
\centering
\caption{BnB CPU vs GPU results for logistic regression with $k=10$, $\rho=0.5$, $\lambda_2=1.0$, $M=3.0$, $n/p=1.0$. Parentheses show lower-bound time.}
\label{tab:bnb_gpu_logistic_M3}
\resizebox{0.7\linewidth}{!}{%
\begin{tabular}{rccc ccc}
\hline
 & \multicolumn{3}{c}{ours CPU} & \multicolumn{3}{c}{ours GPU} \\
\cmidrule(l{0.8em}r{0.8em}){2-4}\cmidrule(l{0.8em}r{0.8em}){5-7}
$p$ & time(s) & gap(\%) & \# nodes & time(s) & gap(\%) & \# nodes \\ \hline
1000 & 689 (38) & 0.00 & 6049 & 758 (108) & 0.00 & 6049 \\
2000 & 536 (39) & 0.00 & 3451 & 556 (65) & 0.00 & 3451 \\
4000 & 251 (62) & 0.00 & 855 & 203 (21) & 0.00 & 855 \\
8000 & 412 (176) & 0.00 & 459 & 246 (18) & 0.00 & 459 \\
16000 & 533 (276) & 0.00 & 207 & 282 (23) & 0.00 & 207 \\
\hline
\end{tabular}%
}
\end{table}

% \clearpage
\subsubsection{Cross Validation to Select $\lambda_2$, $k$, and $M$ for Real-world Datasets}
\label{ec_expt:cv_select_lambda2_k_M_realworld}

To select the hyperparameters $(\lambda_2,k,M)$ for the real-world datasets, we conduct a 5-fold cross-validation study.
For both SantanderBank and DOROTHEA, we evaluate $\lambda_2 \in \{0.01, 0.1, 1.0, 2.0, 3.0, 10.0\}$ and $k \in \{2,3,\ldots,30\}$; during this grid-search step, we fix $M=100$ so that the box constraint is effectively inactive and does not influence model selection. For each $(\lambda_2,k)$ pair, we compute a heuristic solution on each training fold using the beamsearch method of~\citet{liu2024okridge} and report performance on both training and validation folds (squared error for linear regression; log-loss, accuracy, and AUC for logistic regression) as a function of $\lambda_2$ and $k$; see Figure~\ref{ec_fig:beamsearch_cv_santander_lambda2_grid} (SantanderBank) and Figures~\ref{ec_fig:beamsearch_cv_dorothea_lambda2_0p01_0p1}--\ref{ec_fig:beamsearch_cv_dorothea_lambda2_3_10} (DOROTHEA). Based on these results, we select $(\lambda_2,k)=(1.0,10)$ for SantanderBank and $(\lambda_2,k)=(1.0,6)$ for DOROTHEA; under these settings, the maximum absolute coefficient values in the beamsearch solutions are $4.96$ and $4.95$, respectively, so we set $M=10.0$ in the experiments to ensure the box constraint does not affect solution quality.

\clearpage
\begin{figure}[!h]
    \centering
    \includegraphics[width=1.0\textwidth]{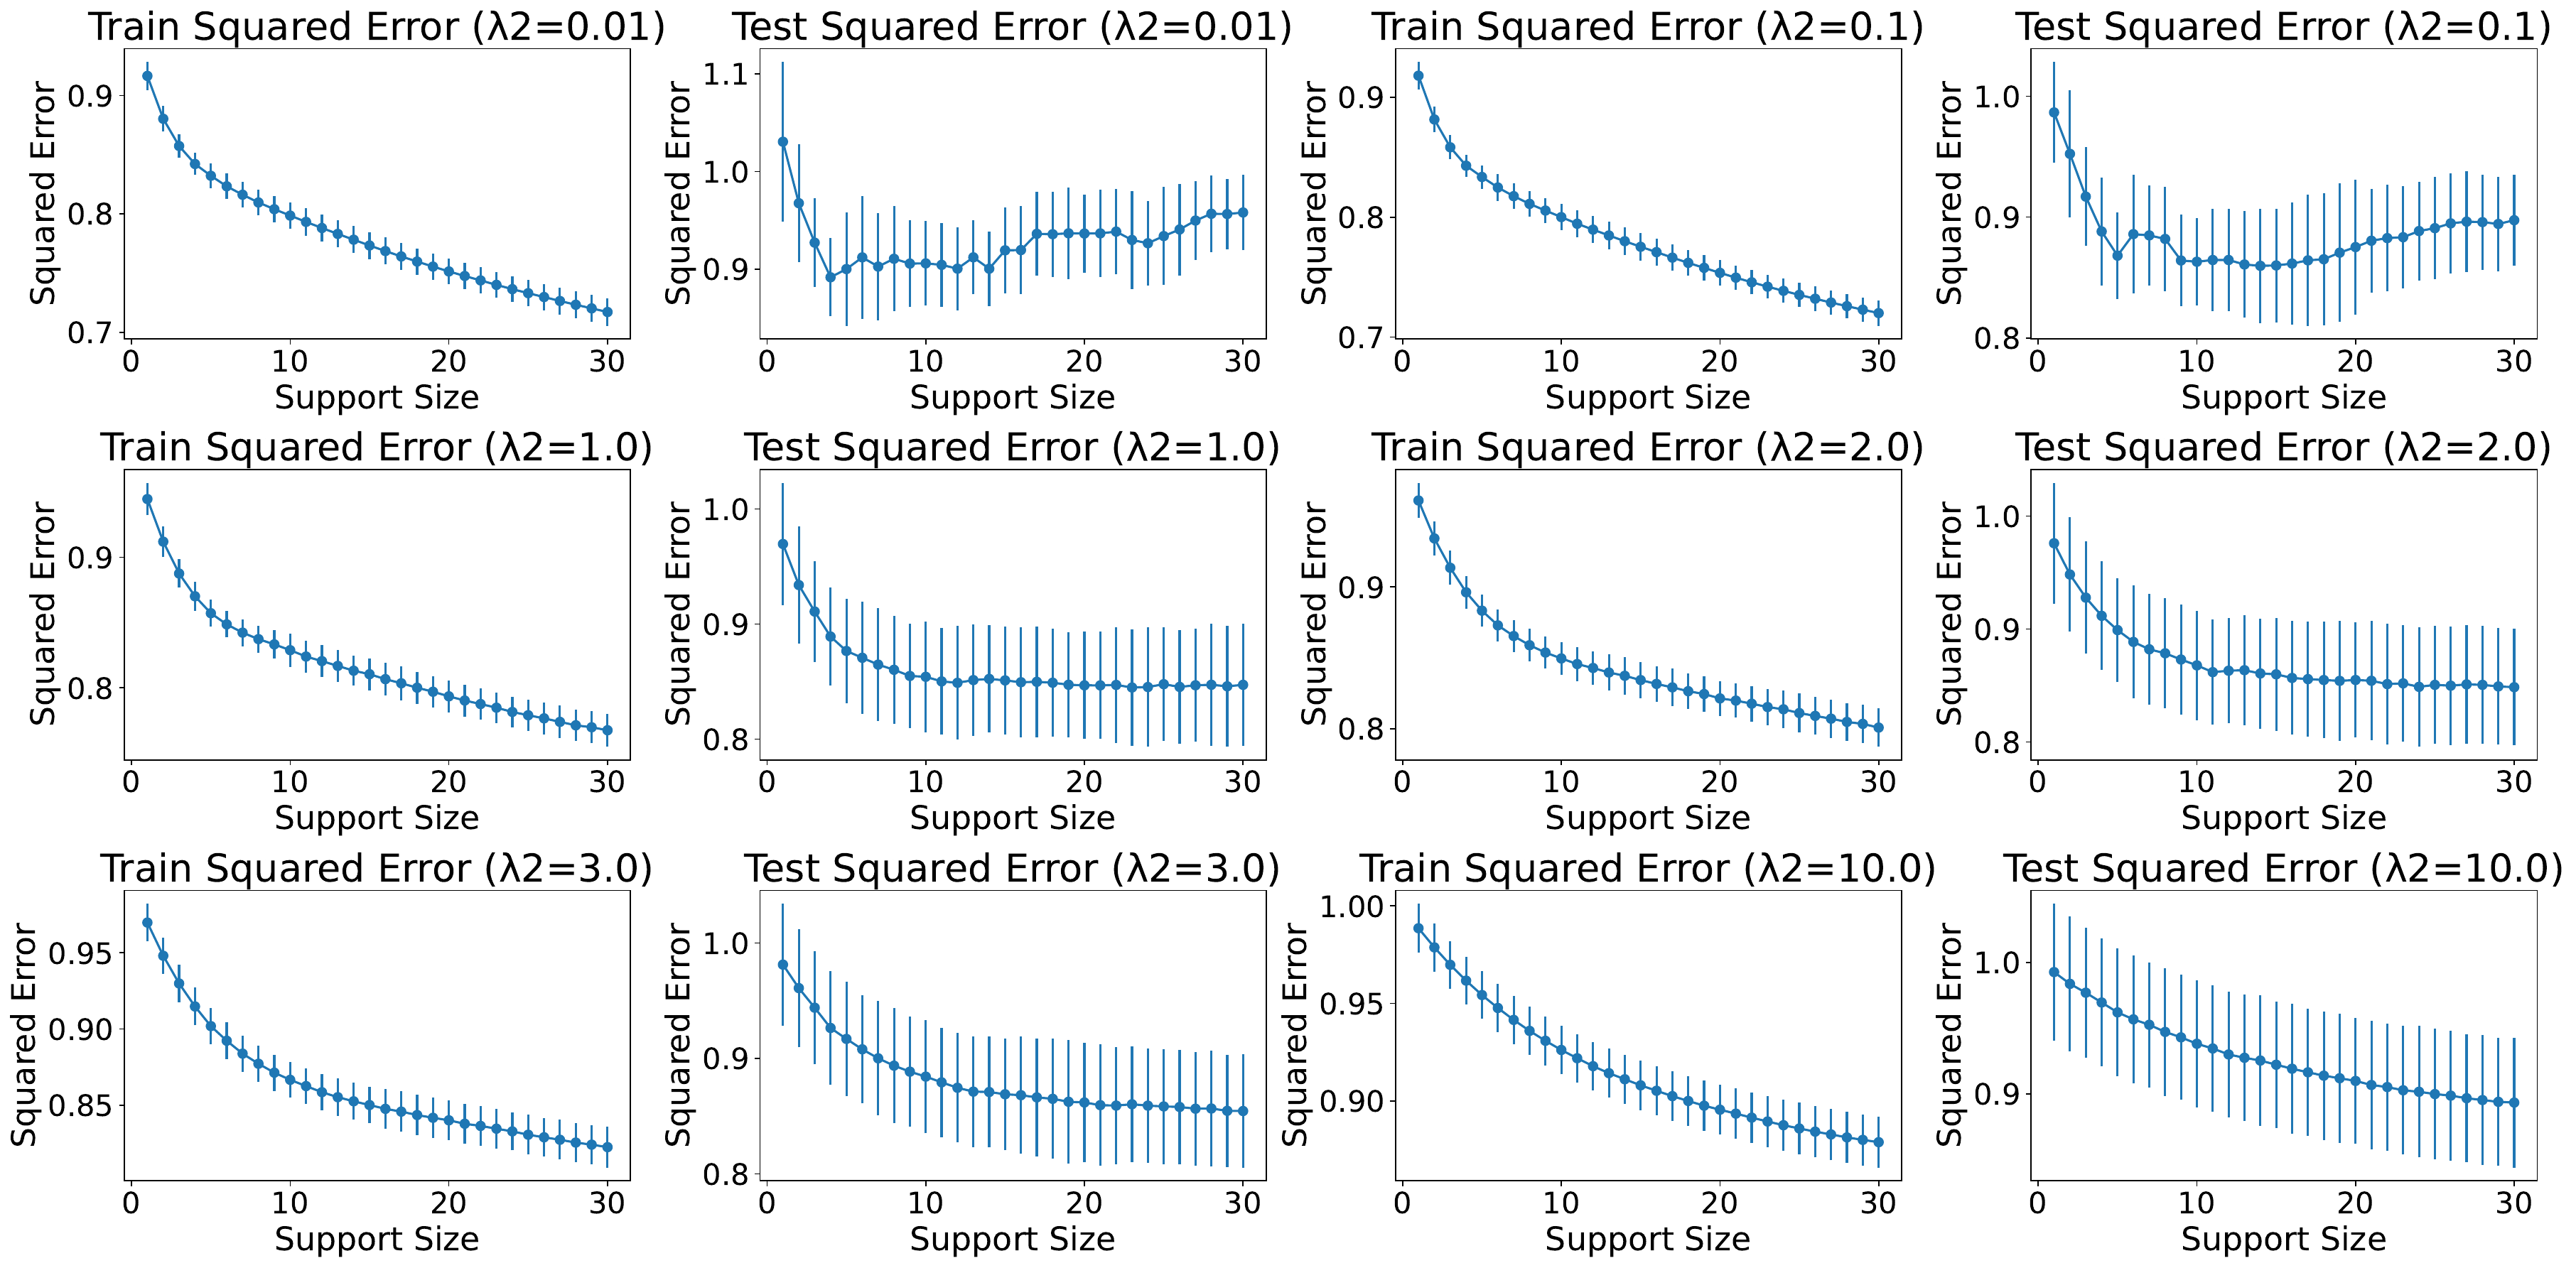}
    \caption{Beamsearch cross-validation results on the SantanderBank dataset with $\lambda_2 \in \{0.01, 0.1, 1.0, 2.0, 3.0, 10.0\}$.}
    \label{ec_fig:beamsearch_cv_santander_lambda2_grid}
    \vspace{0em}
\end{figure}

\begin{figure}[!h]
    \centering
    \includegraphics[width=1.0\textwidth]{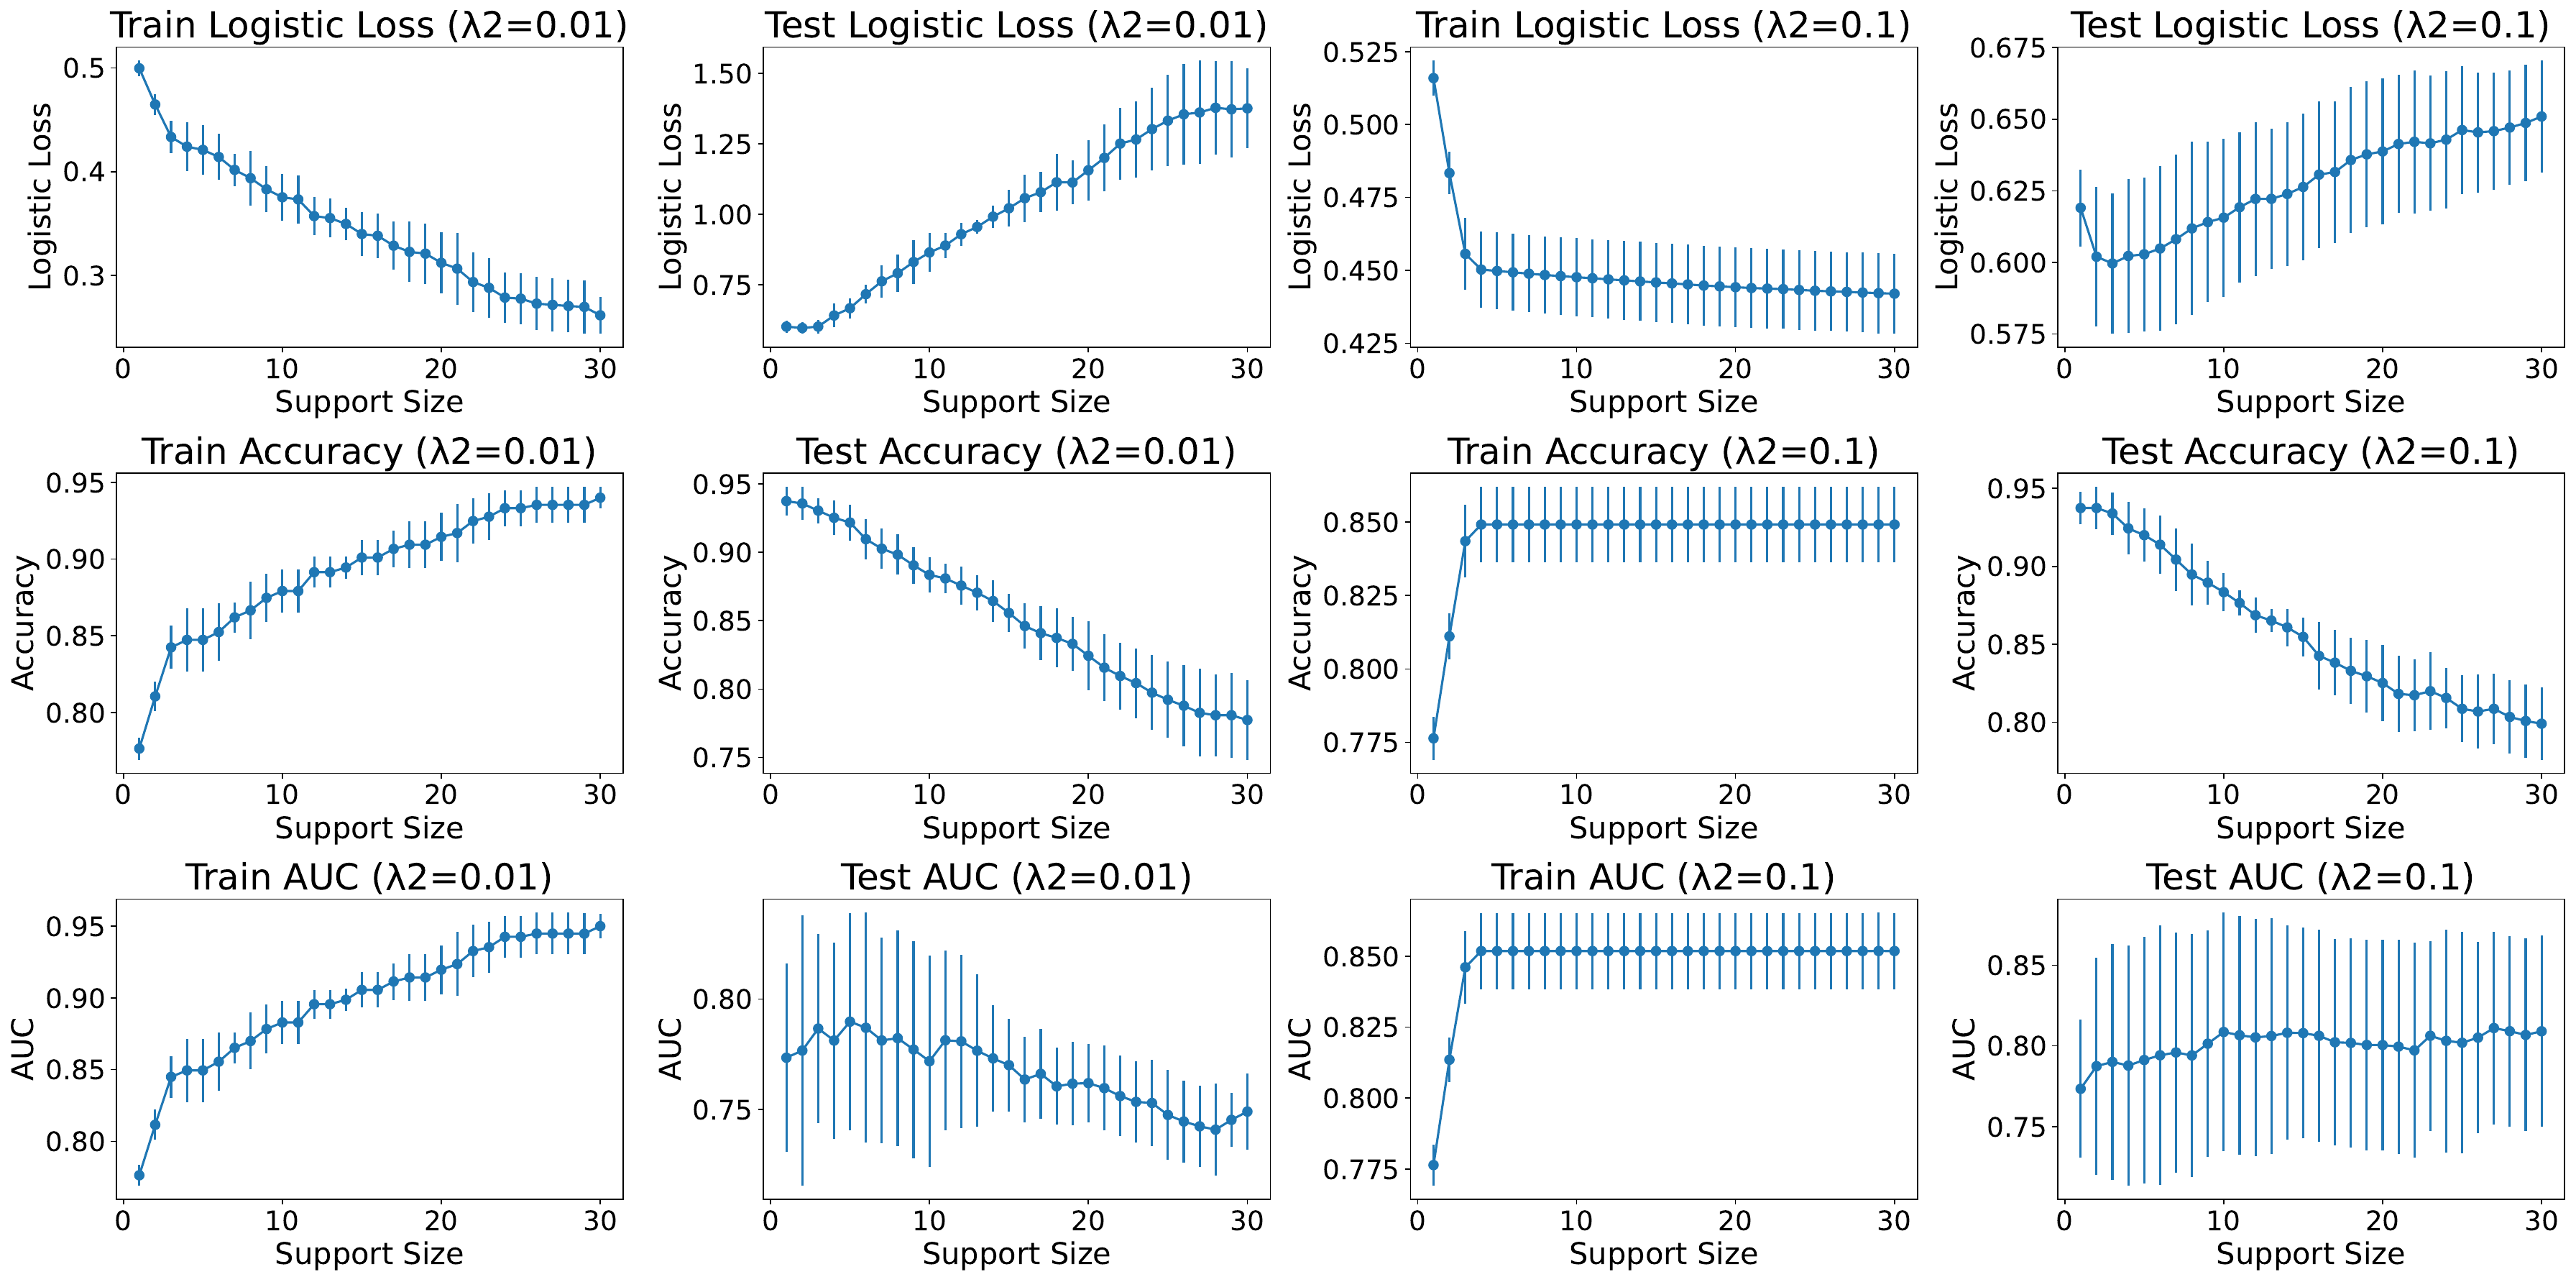}
    \caption{Beamsearch cross-validation results on the DOROTHEA dataset with $\lambda_2 \in \{0.01, 0.1\}$.}
    \label{ec_fig:beamsearch_cv_dorothea_lambda2_0p01_0p1}
    \vspace{0em}
\end{figure}

\clearpage
\begin{figure}[!h]
    \centering
    \includegraphics[width=1.0\textwidth]{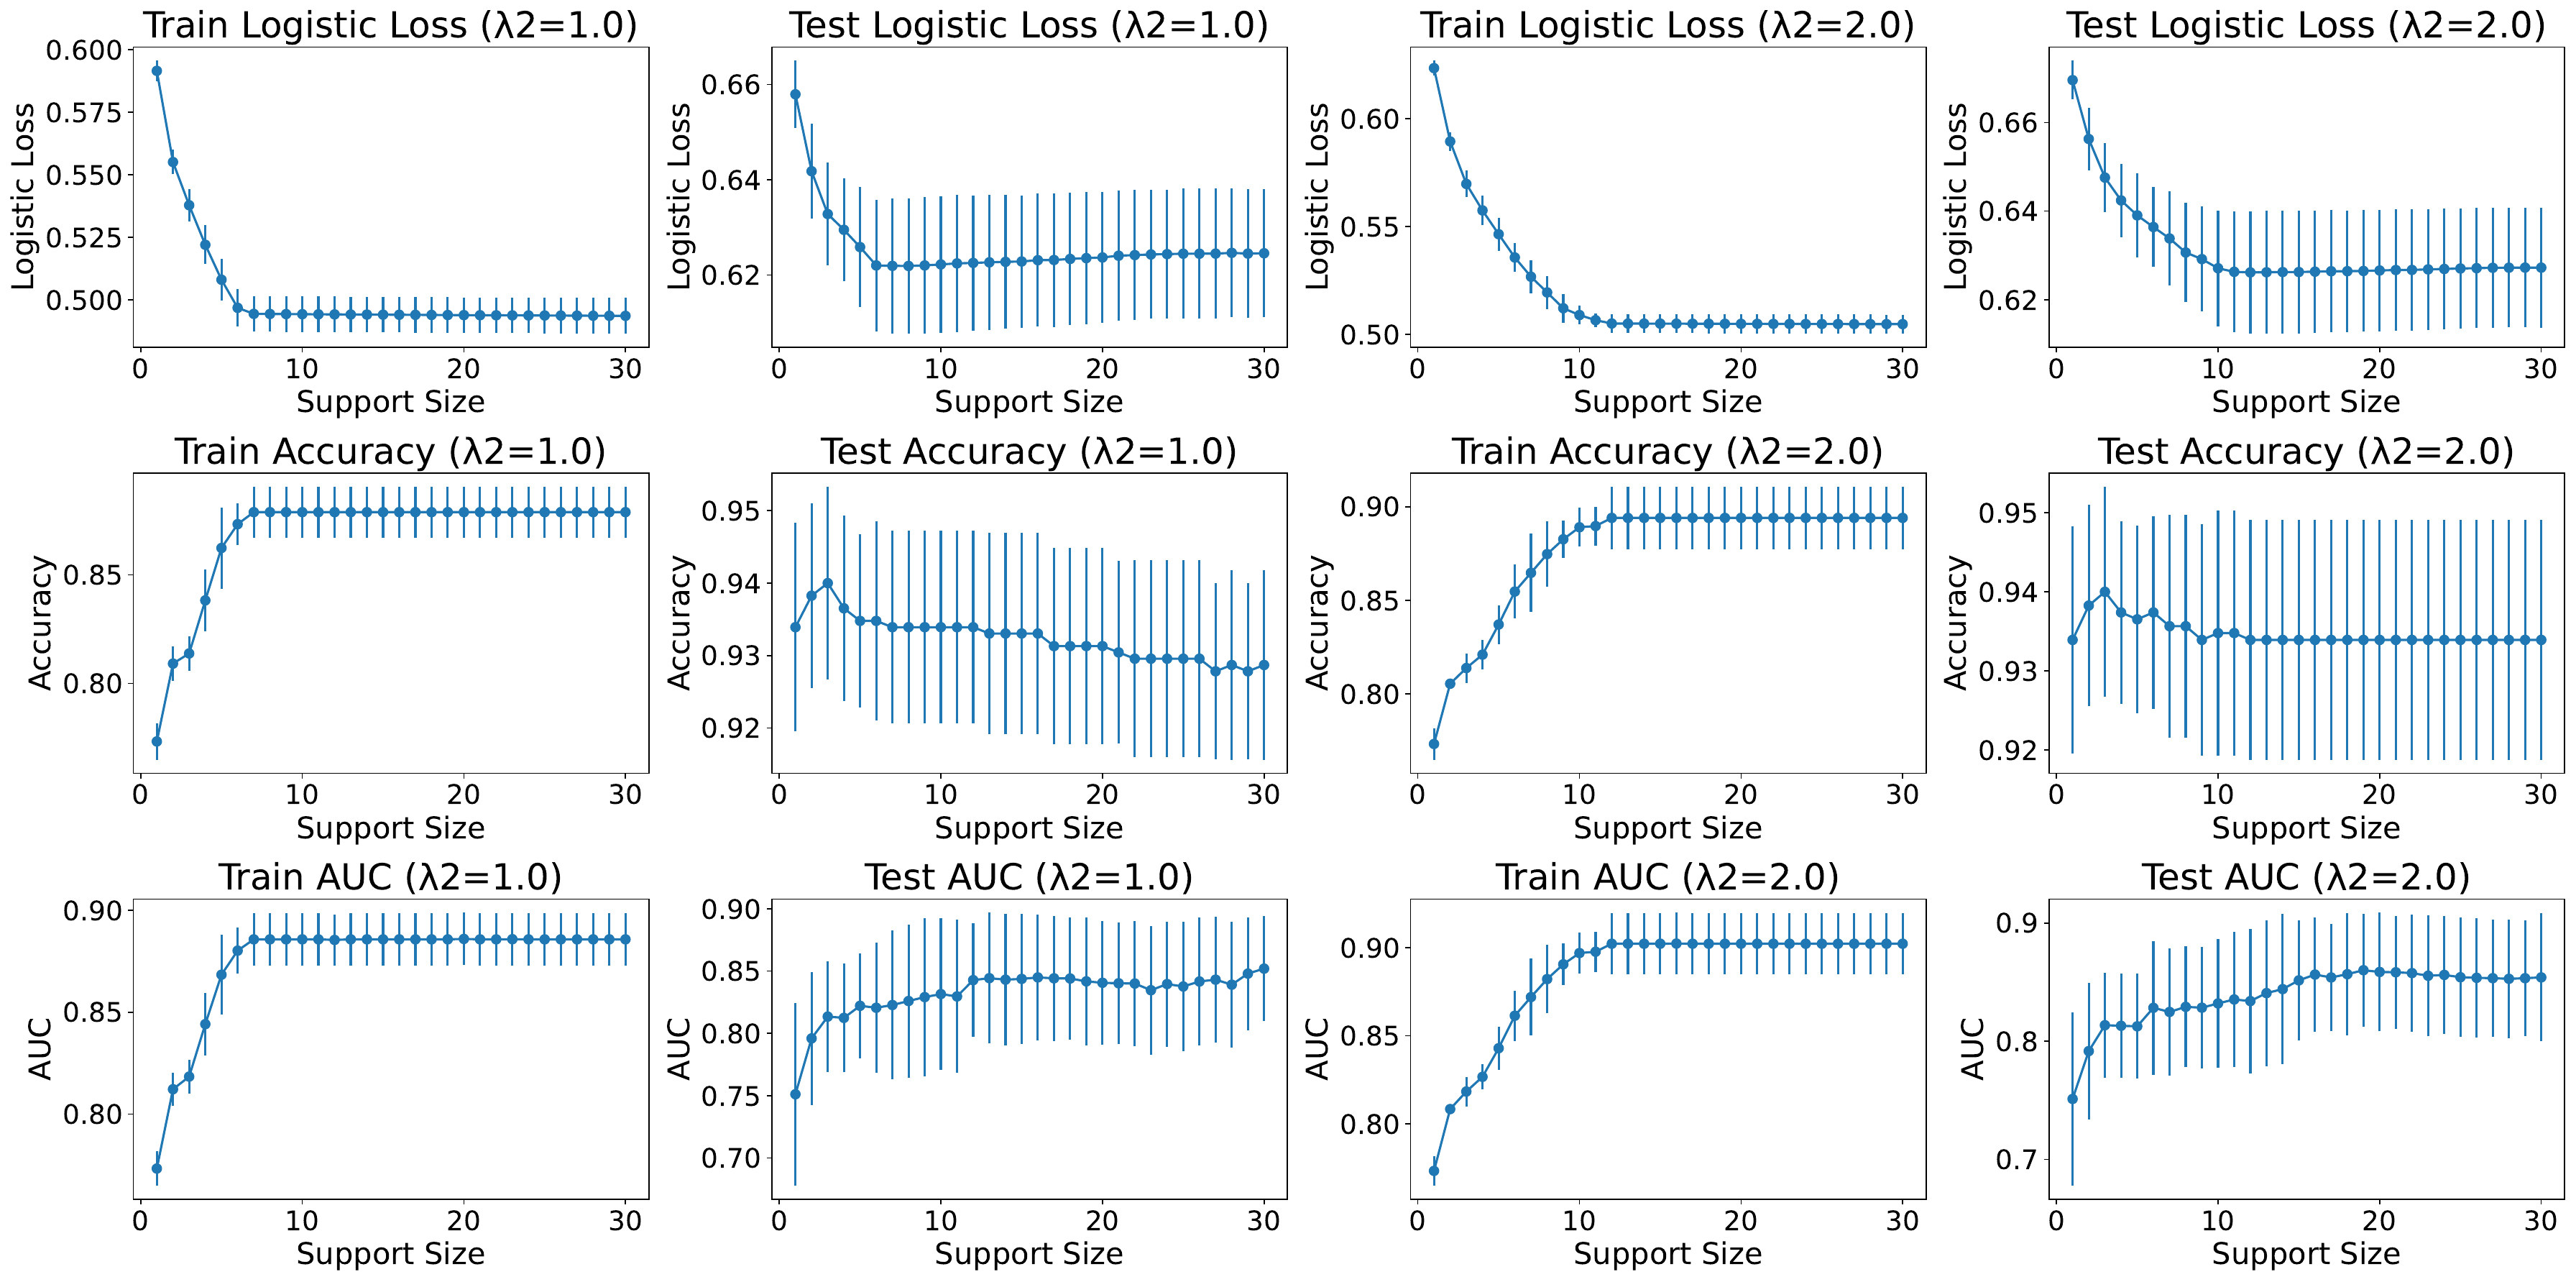}
    \caption{Beamsearch cross-validation results on the DOROTHEA dataset with $\lambda_2 \in \{1.0, 2.0\}$.}
    \label{ec_fig:beamsearch_cv_dorothea_lambda2_1_2}
    \vspace{0em}
\end{figure}

\begin{figure}[!h]
    \centering
    \includegraphics[width=1.0\textwidth]{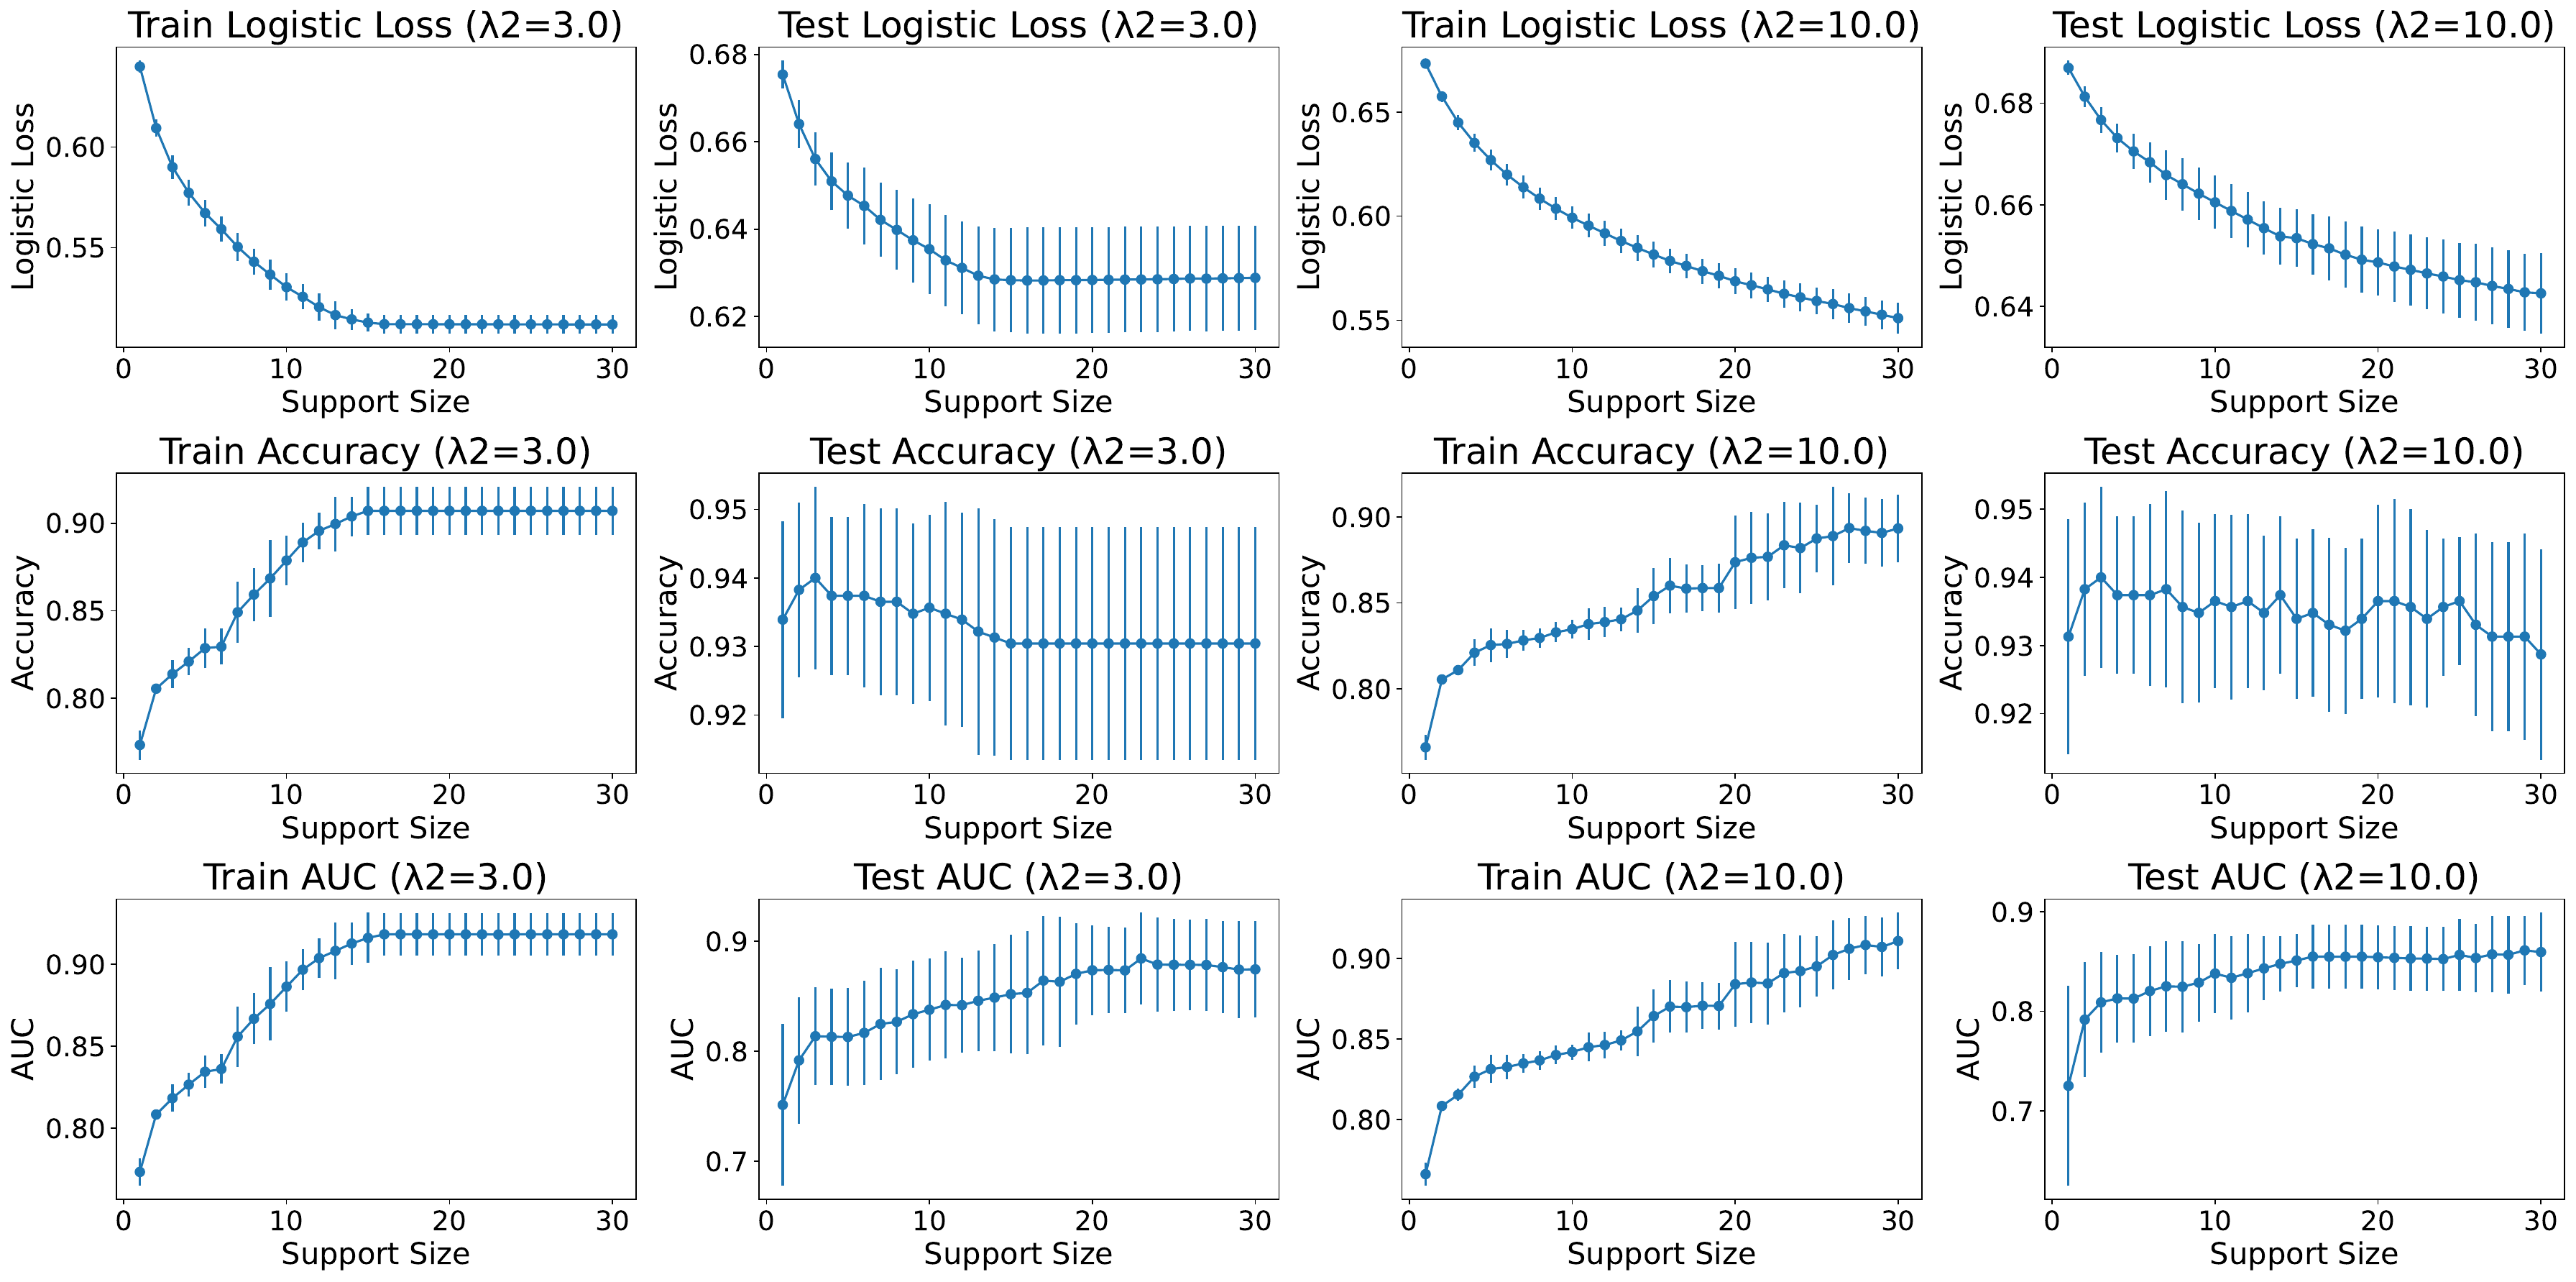}
    \caption{Beamsearch cross-validation results on the DOROTHEA dataset with $\lambda_2 \in \{3.0, 10.0\}$.}
    \label{ec_fig:beamsearch_cv_dorothea_lambda2_3_10}
\end{figure}
