# Supplementary material for: GPU-friendly and Linearly Convergent First-order Methods for Certifying Optimal $k$-sparse GLMs
Source: arXiv:2603.01306 source file (2026-03-01)
Supplement: Supplementary file 2 [file additional_expt_results.tex]

\section{Additional Experimental Results}
\label{ec:additional_results}

\subsection{Solving the Perspective Relaxation}
\label{ec_expt:perturbation_study_on_solving_the_perspective_relaxation}

We provide perturbation studies on solving the perspective relaxation by varying the box constraint $M$, the $\ell_2$ regularization coefficient $\lambda_2$, and the sample-to-feature ($n$-to-$p$) ratio. Unless otherwise noted, settings match Figure~\ref{fig:solve_convex_relaxation_main_paper} ($M=2.0$, $\lambda_2=1.0$, $n$-to-$p$ ratio $=1$).

Figure~\ref{ec_fig:convex_relaxation_M_1.2} and Figure~\ref{ec_fig:convex_relaxation_M_5.0} tighten and loosen the box constraint to $M=1.2$ and $M=5.0$, respectively. Figure~\ref{ec_fig:convex_relaxation_lambda2_0.1} and Figure~\ref{ec_fig:convex_relaxation_lambda2_10} vary the $\ell_2$ penalty to $\lambda_2 = 0.1$ and $\lambda_2 = 10$. Figure~\ref{ec_fig:convex_relaxation_n_p_ratio_10.0} and Figure~\ref{ec_fig:convex_relaxation_n_p_ratio_0.1} adjust the $n$-to-$p$ ratio to $10.0$ and $0.1$ while keeping $M=2.0$ and $\lambda_2=1.0$.

\begin{figure}[!h]
    \vspace{0em}
    \centering
    \includegraphics[width=1.0\textwidth]{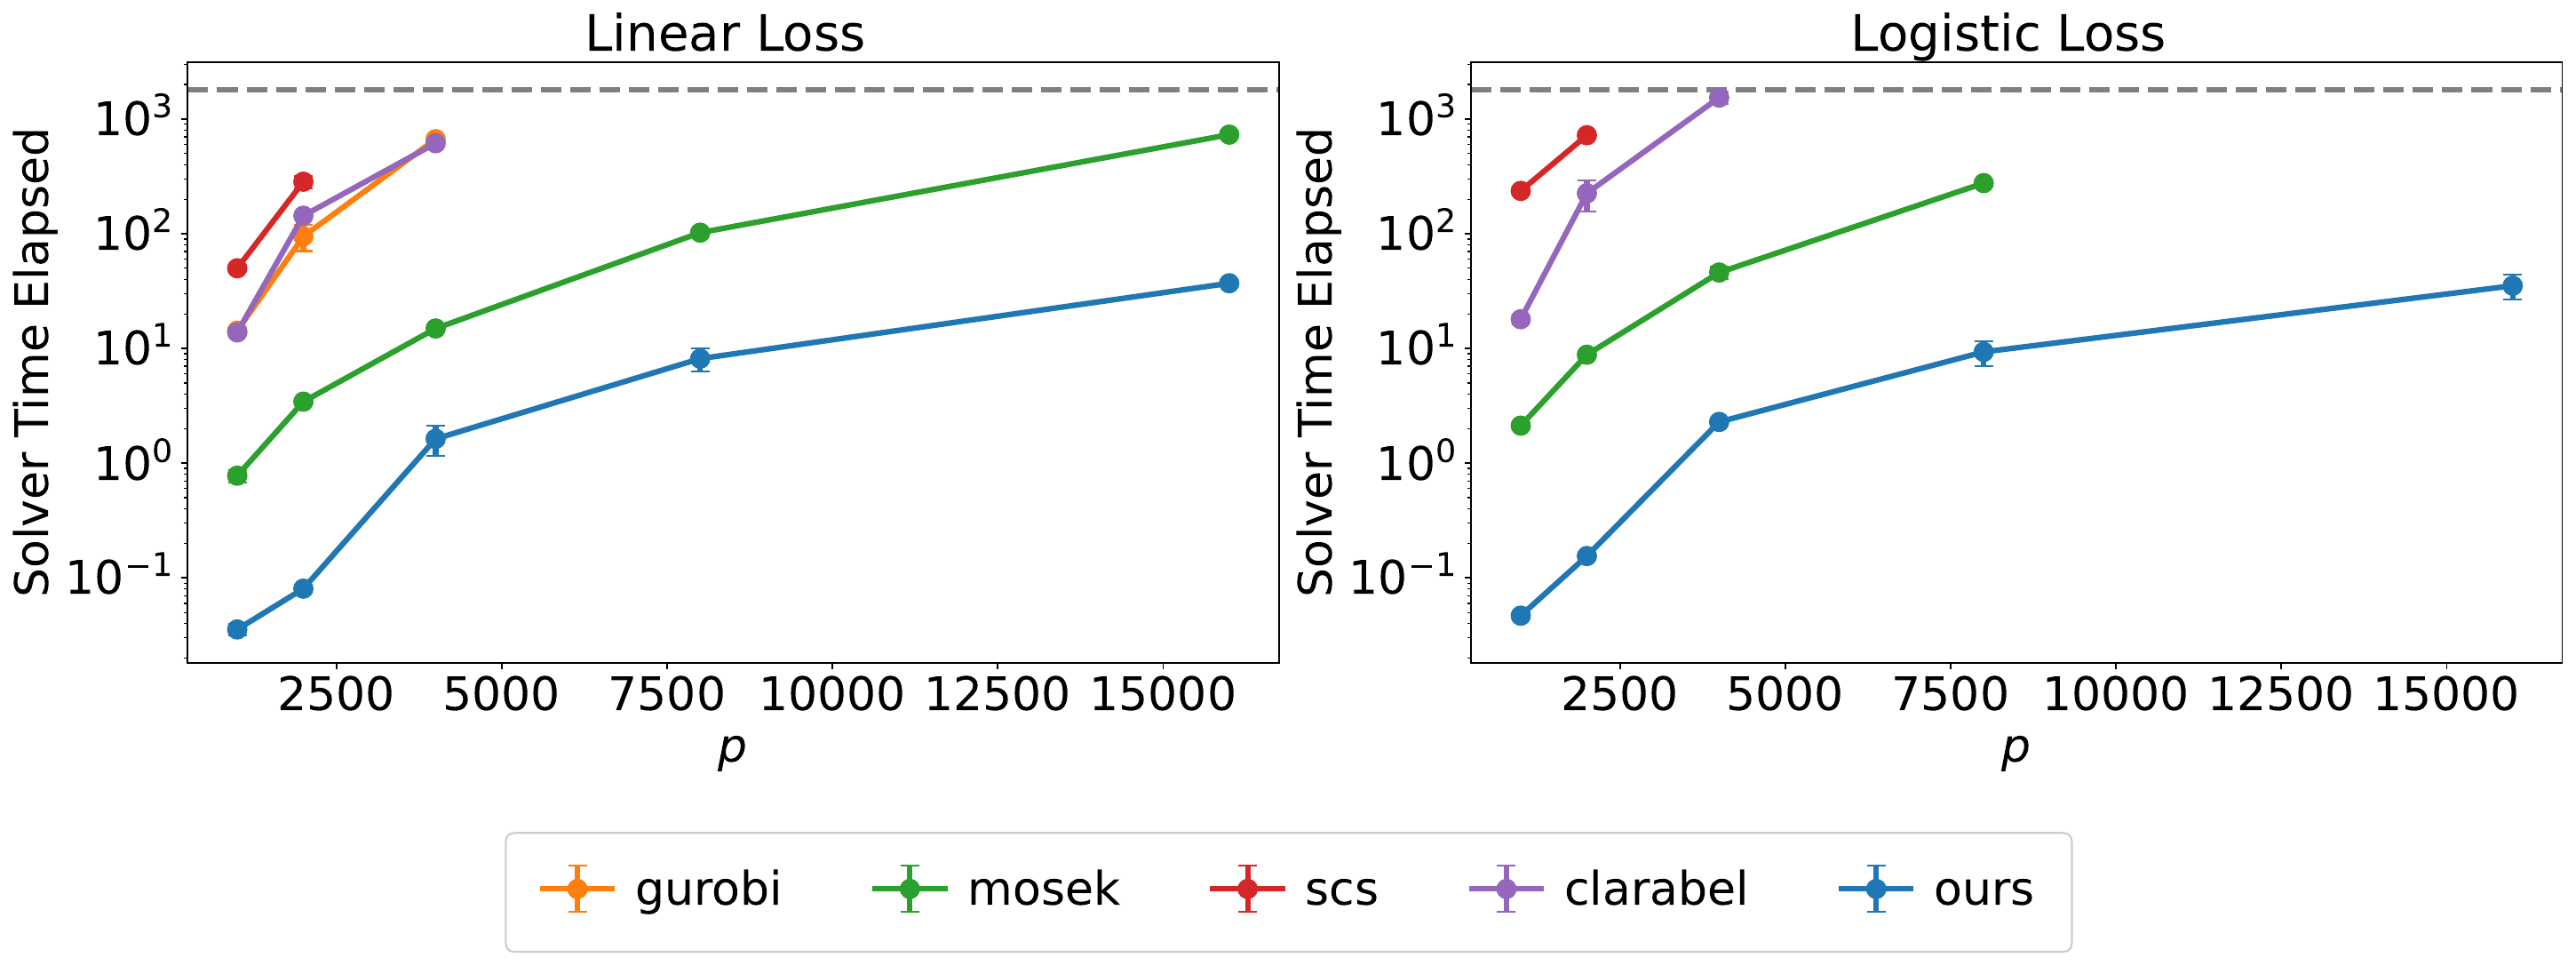}
    \caption{Running time comparison of solving Problem~\ref{obj:perspective_relaxation} when the box constraint is tightened to $M=1.2$.}
    \label{ec_fig:convex_relaxation_M_1.2}
    \vspace{0em}
\end{figure}

\begin{figure}[!h]
    \vspace{0em}
    \centering
    \includegraphics[width=1.0\textwidth]{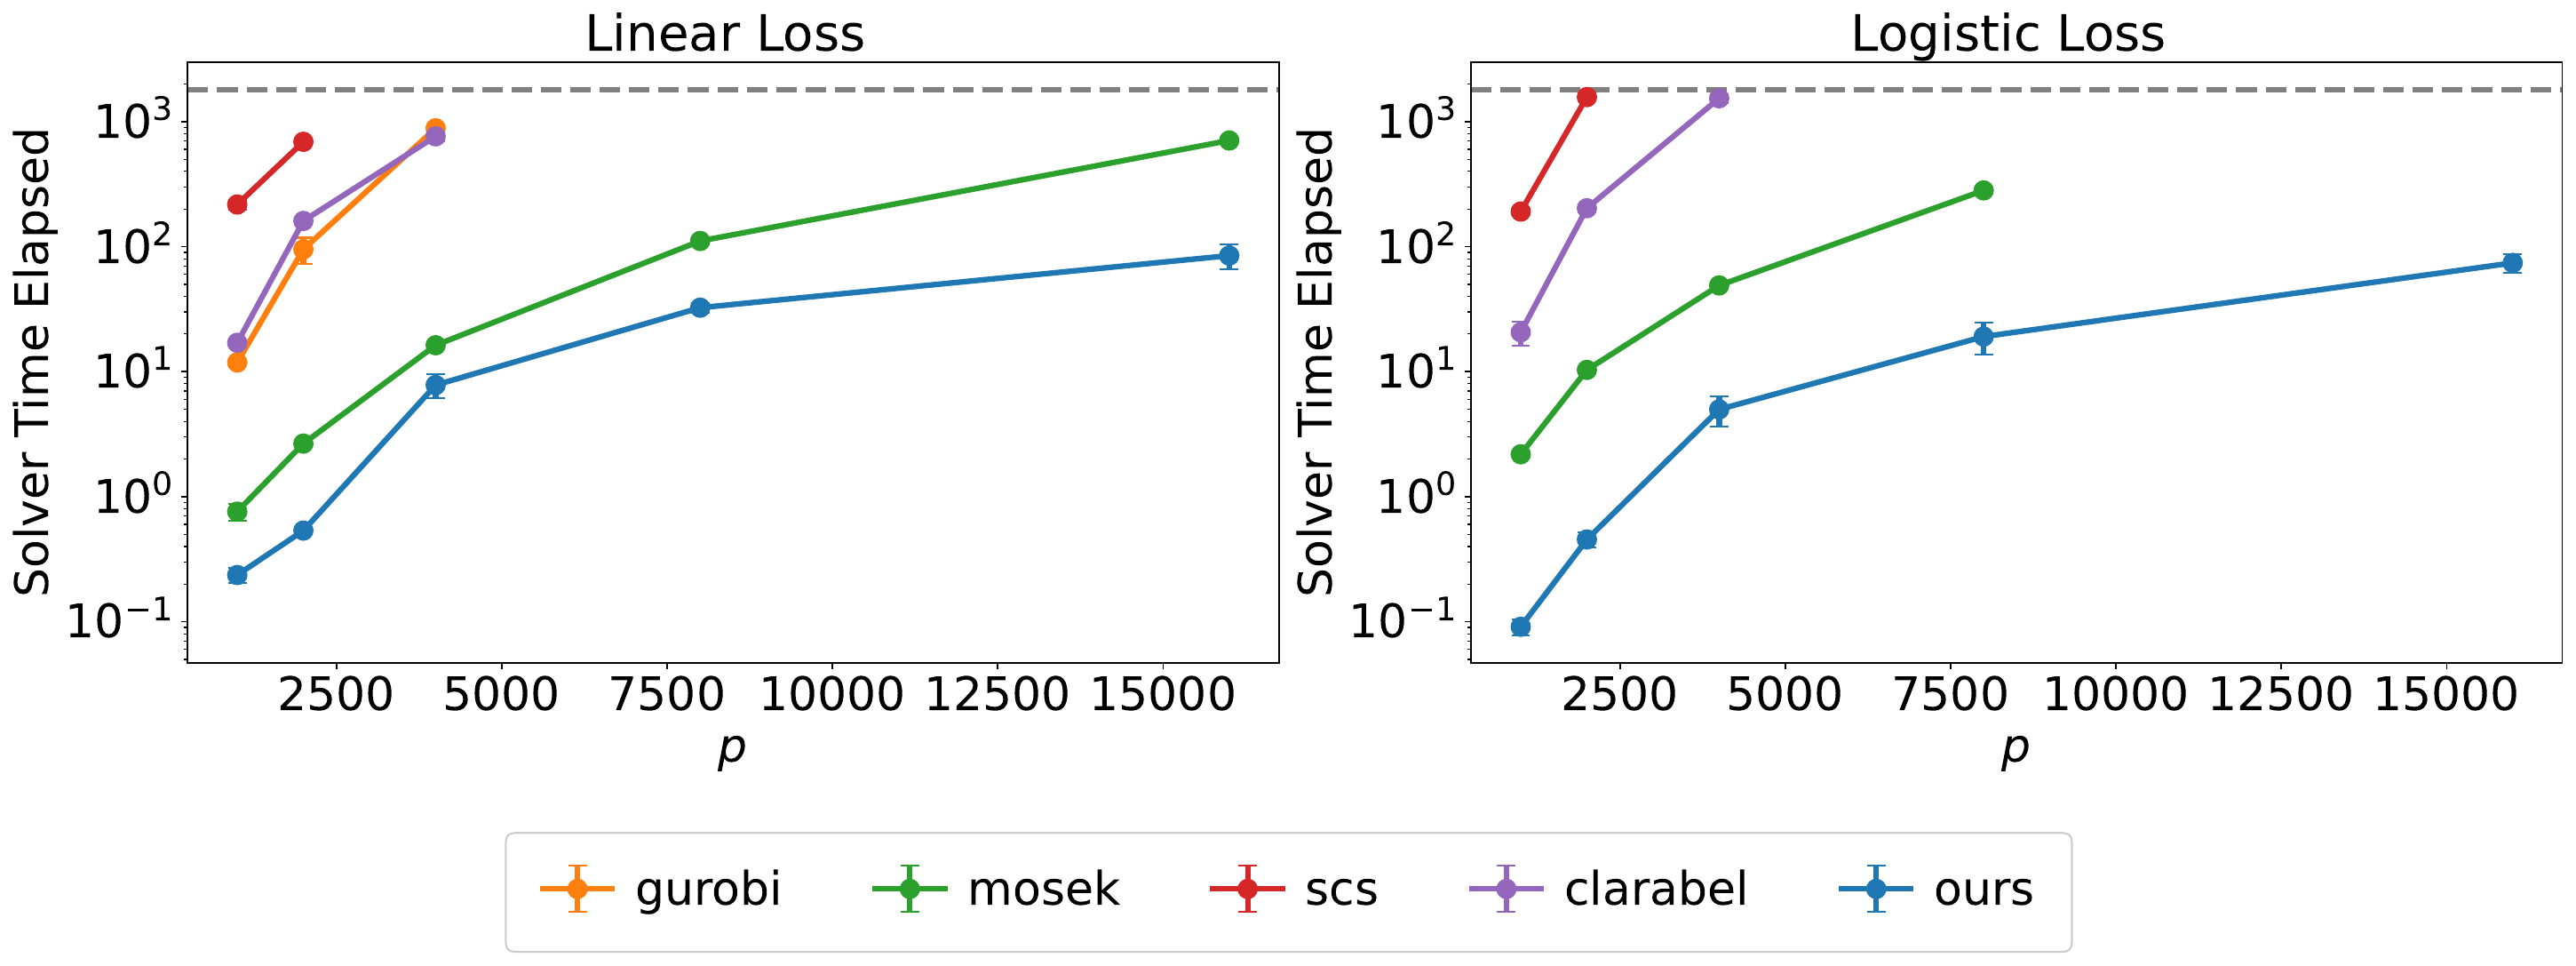}
    \caption{Running time comparison of solving Problem~\ref{obj:perspective_relaxation} when the box constraint is relaxed to $M=5.0$.}
    \label{ec_fig:convex_relaxation_M_5.0}
    \vspace{0em}
\end{figure}

\clearpage

\begin{figure}[!h]
    \centering
    \includegraphics[width=1.0\textwidth]{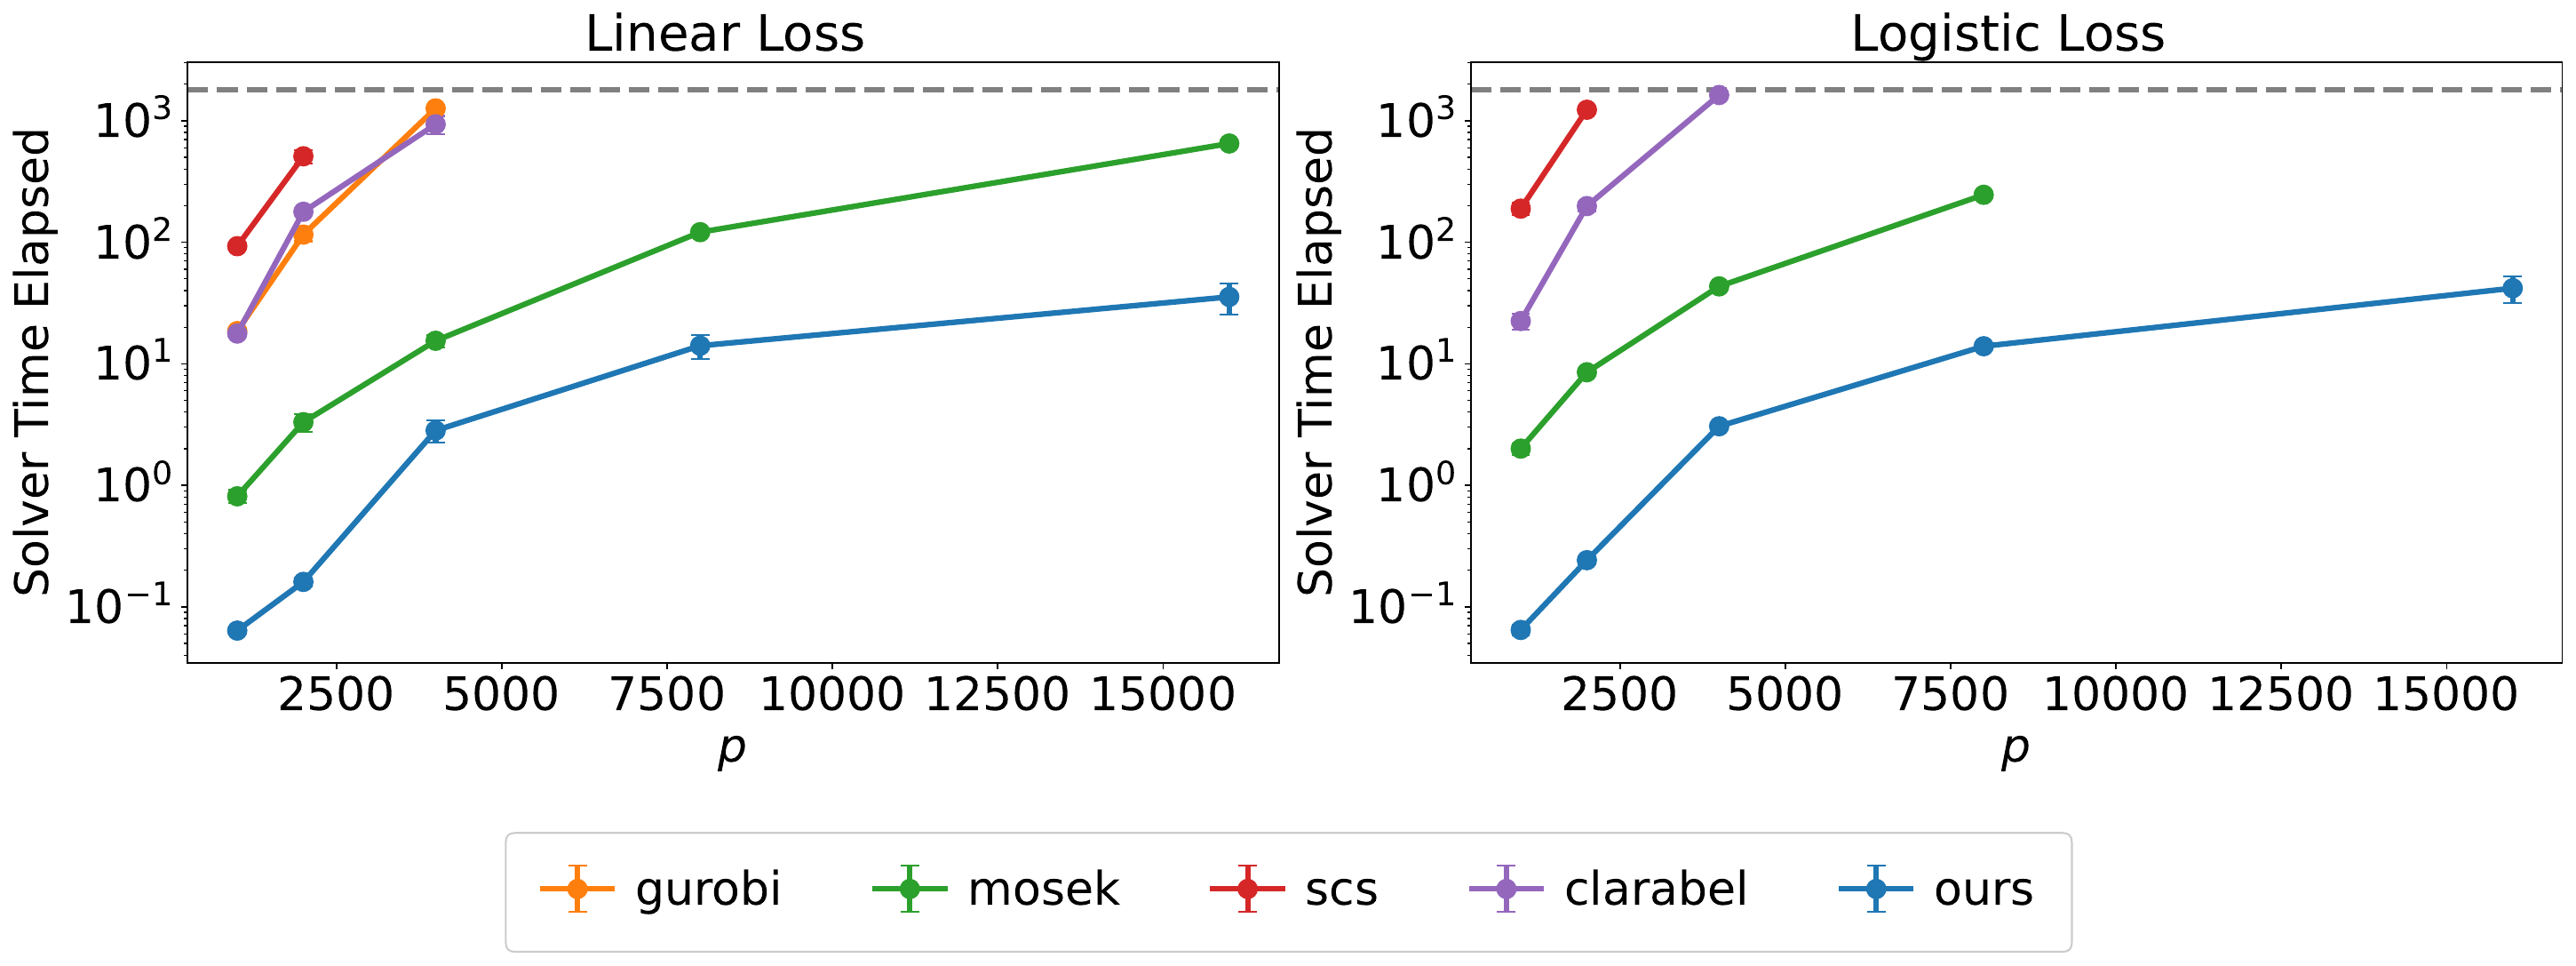}
    \caption{Running time comparison of solving Problem~\ref{obj:perspective_relaxation} with the $\ell_2$ regularization reduced to $\lambda_2 = 0.1$.}
    \label{ec_fig:convex_relaxation_lambda2_0.1}
    \vspace{0em}
\end{figure}

\begin{figure}[!h]
    \centering
    \includegraphics[width=1.0\textwidth]{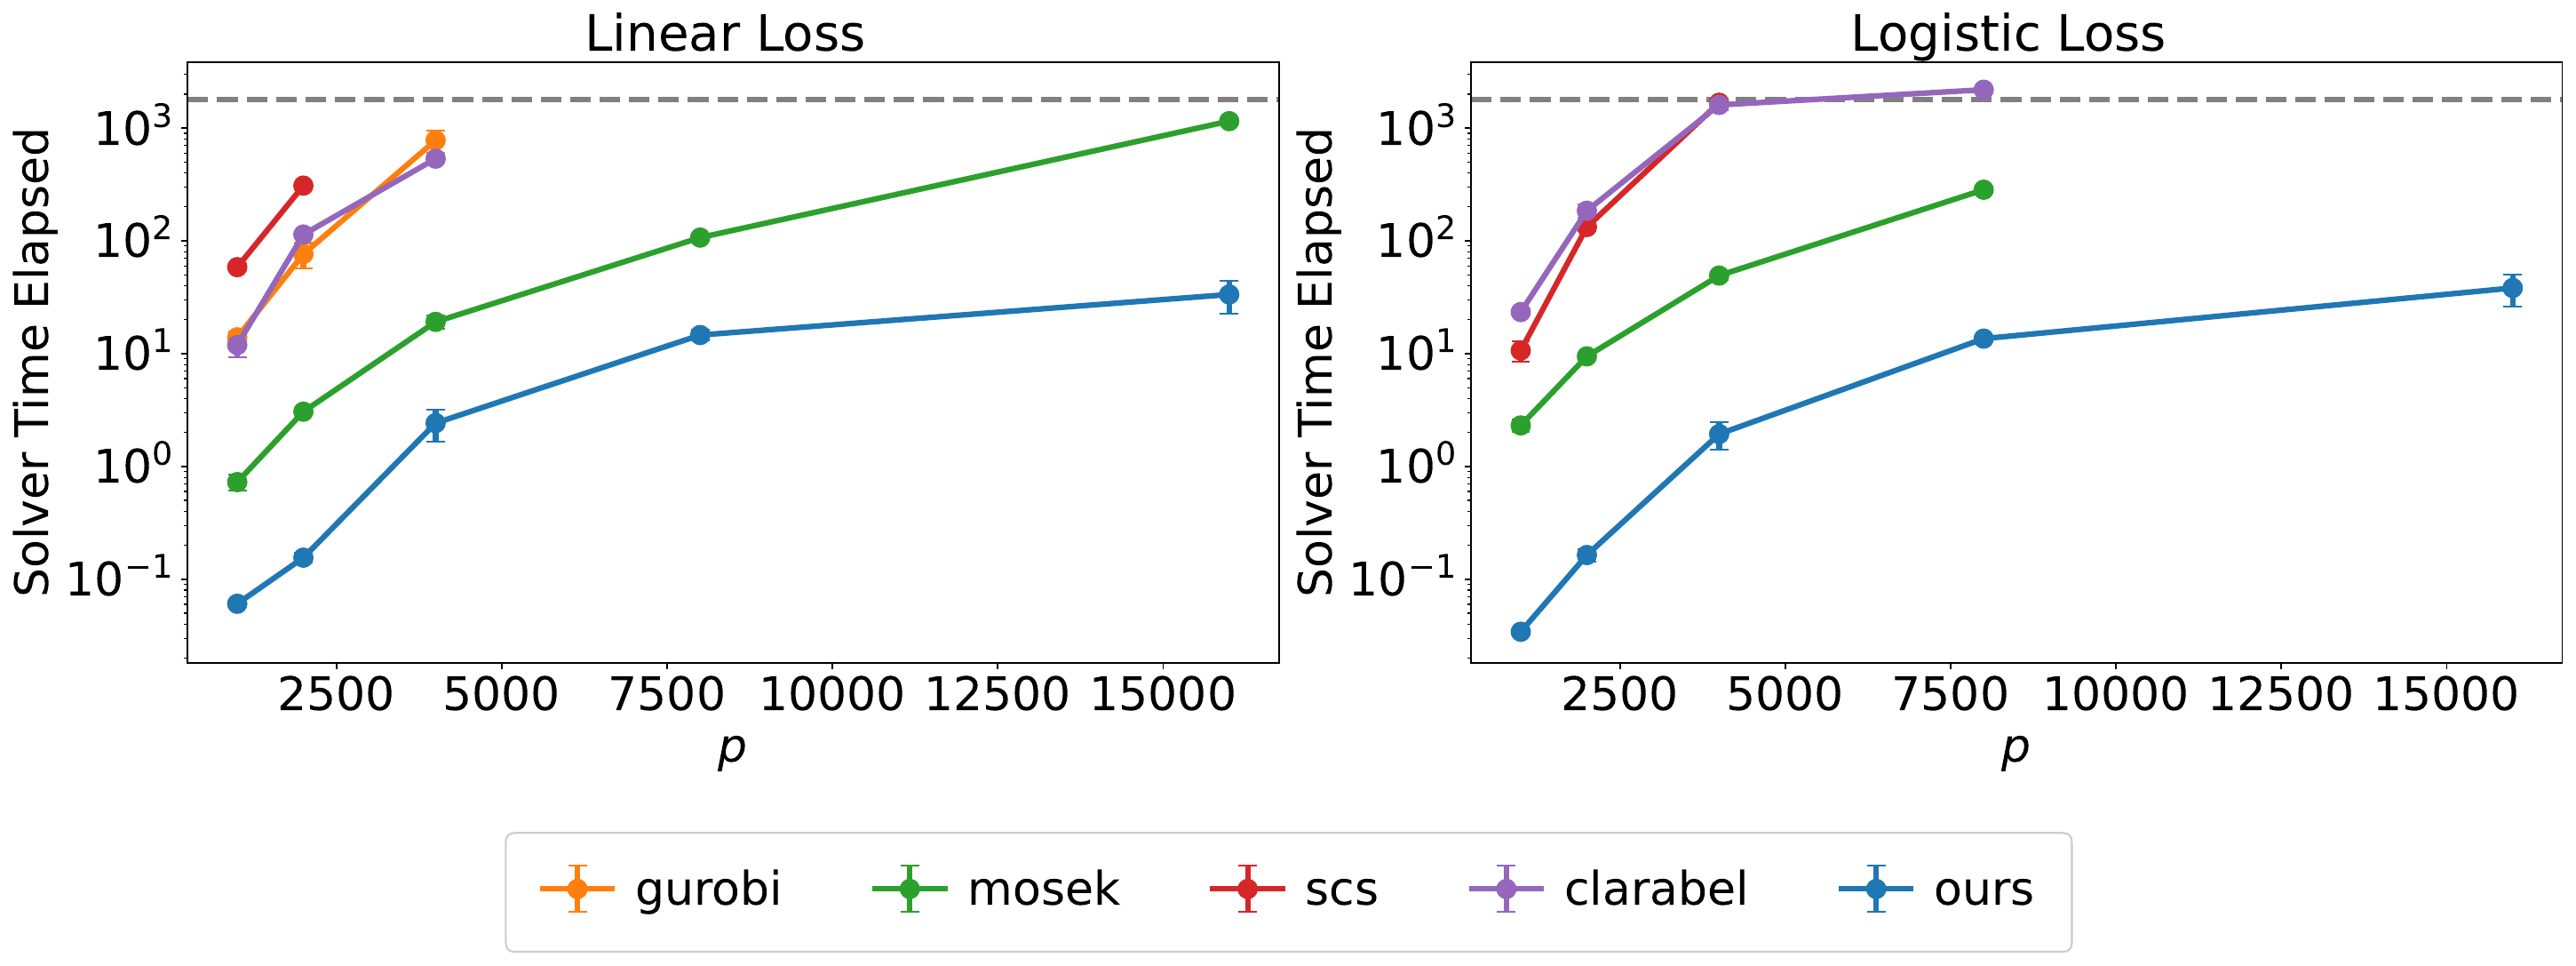}
    \caption{Running time comparison of solving Problem~\ref{obj:perspective_relaxation} with the $\ell_2$ regularization increased to $\lambda_2 = 10$.}
    \label{ec_fig:convex_relaxation_lambda2_10}
    \vspace{0em}
\end{figure}

\clearpage

\begin{figure}[!h]
    \centering
    \includegraphics[width=1.0\textwidth]{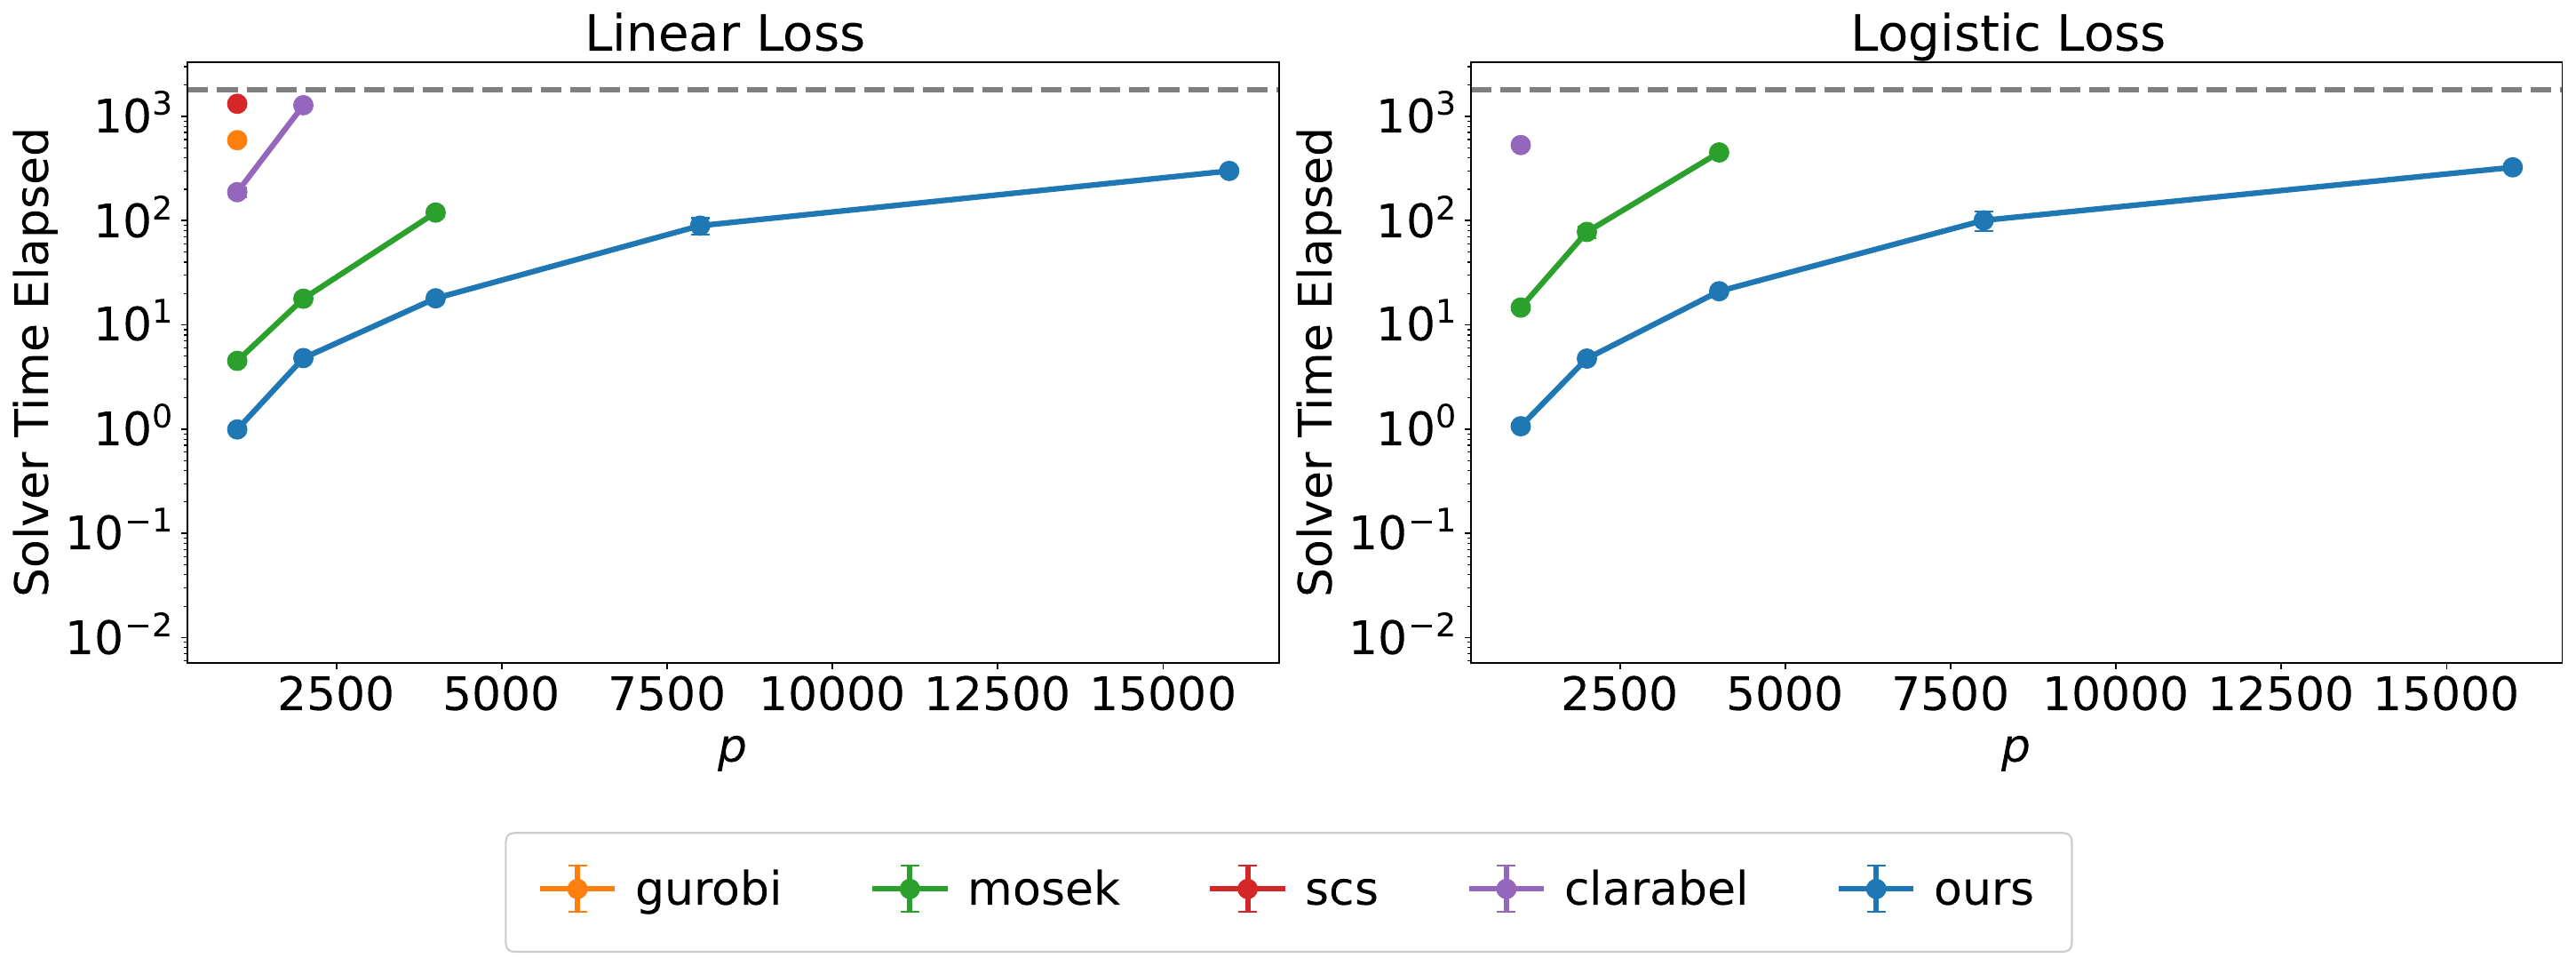}
    \caption{Running time comparison of solving Problem~\ref{obj:perspective_relaxation} when the $n$-to-$p$ ratio is increased to $10.0$.}
    \label{ec_fig:convex_relaxation_n_p_ratio_10.0}
    \vspace{0em}
\end{figure}

\begin{figure}[!h]
    \centering
    \includegraphics[width=1.0\textwidth]{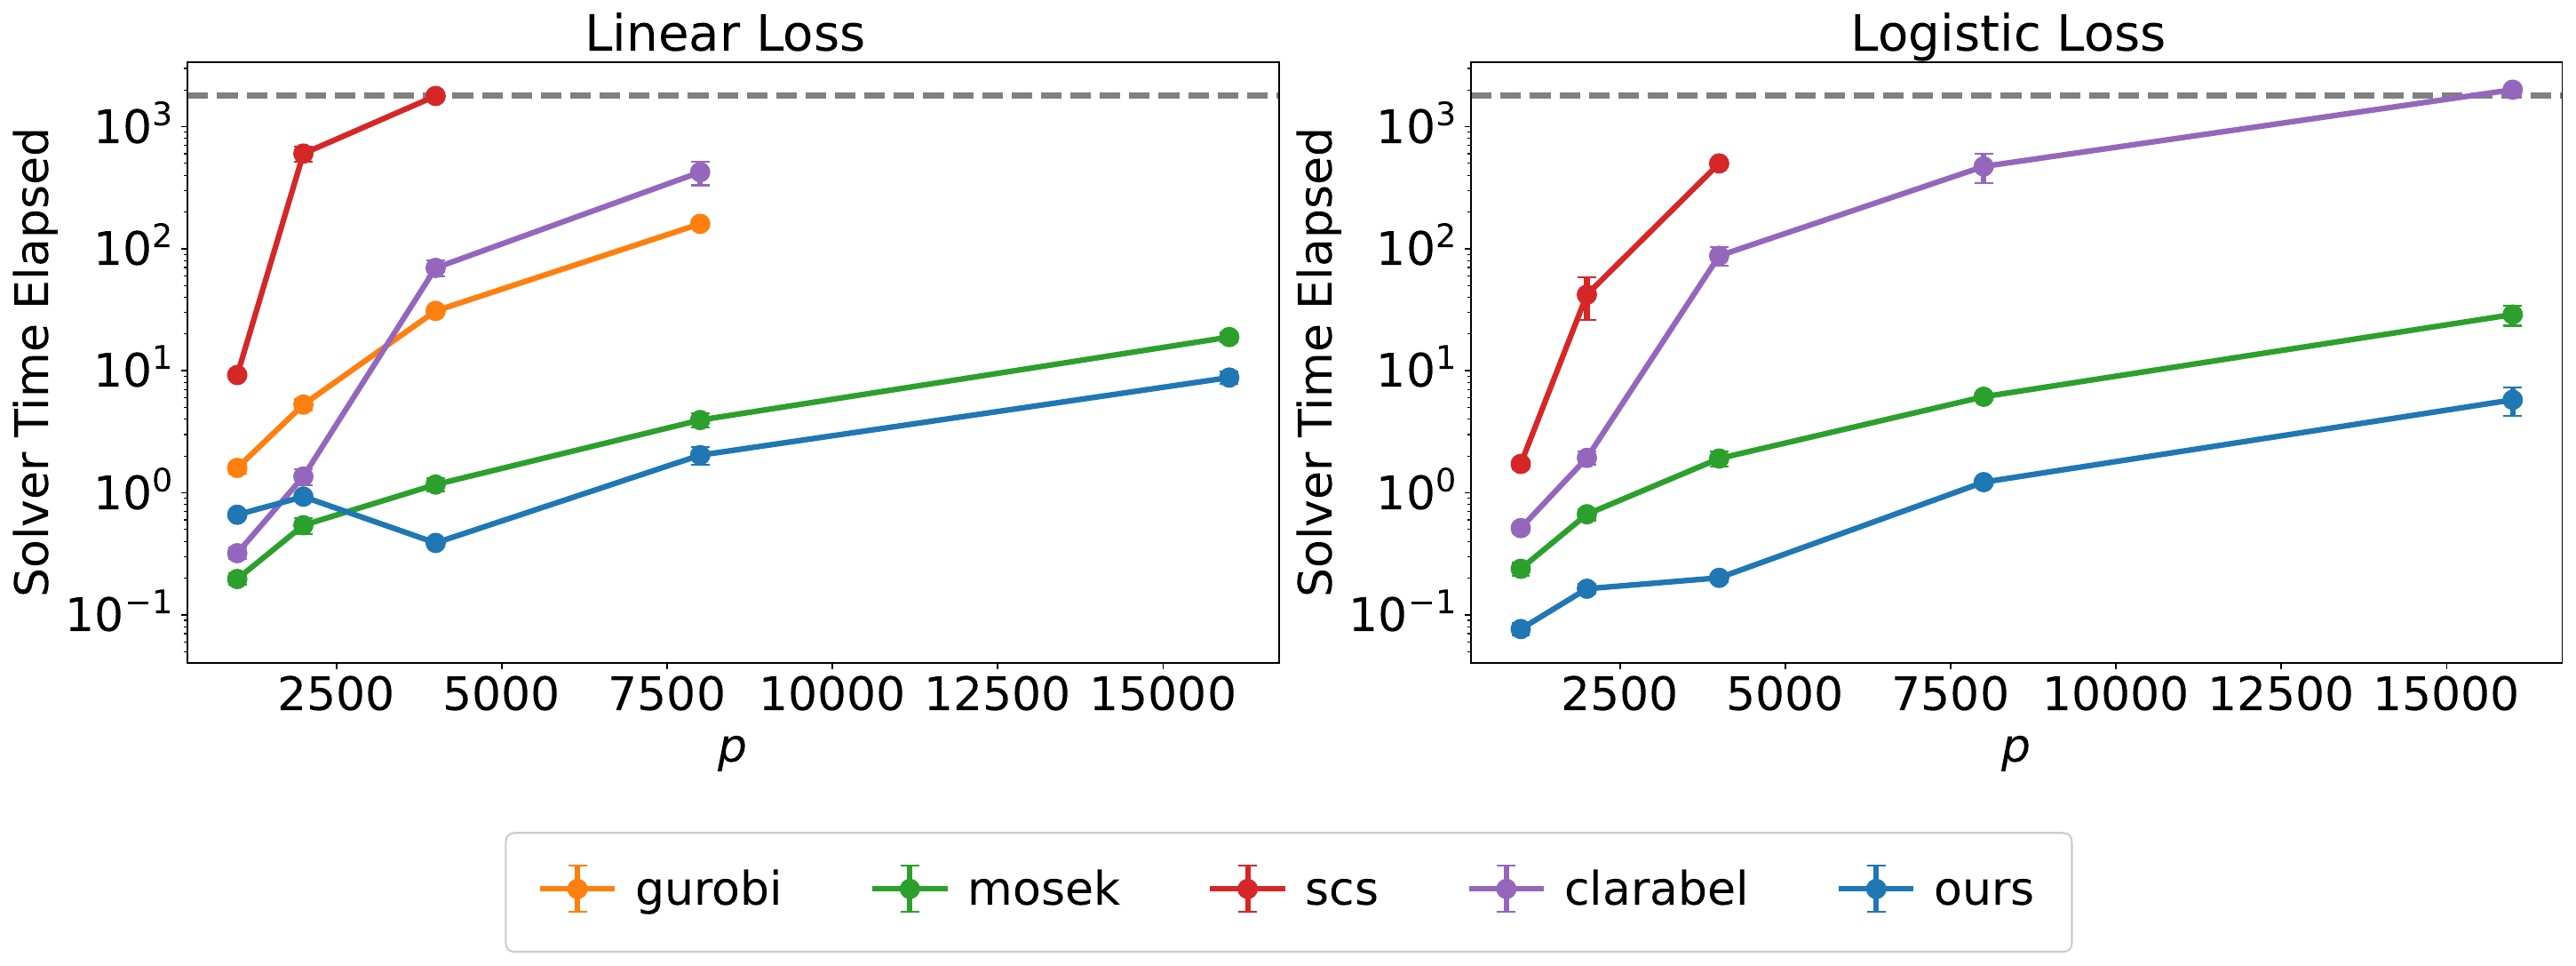}
    \caption{Running time comparison of solving Problem~\ref{obj:perspective_relaxation} when the $n$-to-$p$ ratio is decreased to $0.1$.}
    \label{ec_fig:convex_relaxation_n_p_ratio_0.1}
\end{figure}

\clearpage

\subsection{Shrink Factor in Duality-based Restart Scheme}
\label{ec_expt:shrink_factor_in_duality_based_restart_scheme}
In the main paper, we noted that the duality-based restart scheme can work with any decrease factor $\eta>1$, but the choice of $\eta$ affects practical running speed.
We compare $\eta \in \{e, e^2, e^3\}$ to illustrate this effect.
The results are shown in Figure~\ref{ec_fig:PDRestart_achieves_linear_convergence_rate_exponents_linear} and Figure~\ref{ec_fig:PDRestart_achieves_linear_convergence_rate_exponents_logistic}.
We are able to improve the practical speeds of all methods by changing $\eta$ from $e$ to $e^2$ and $e^3$, which matches the theoretical prediction in Theorem~\ref{theorem:optimal_restart_eta_choice} and discussion at the end of Section~\ref{subsec:restart_scheme}.

\begin{figure}[!h]
    \vspace{0em}
    \centering
    \includegraphics[width=1.0\textwidth]{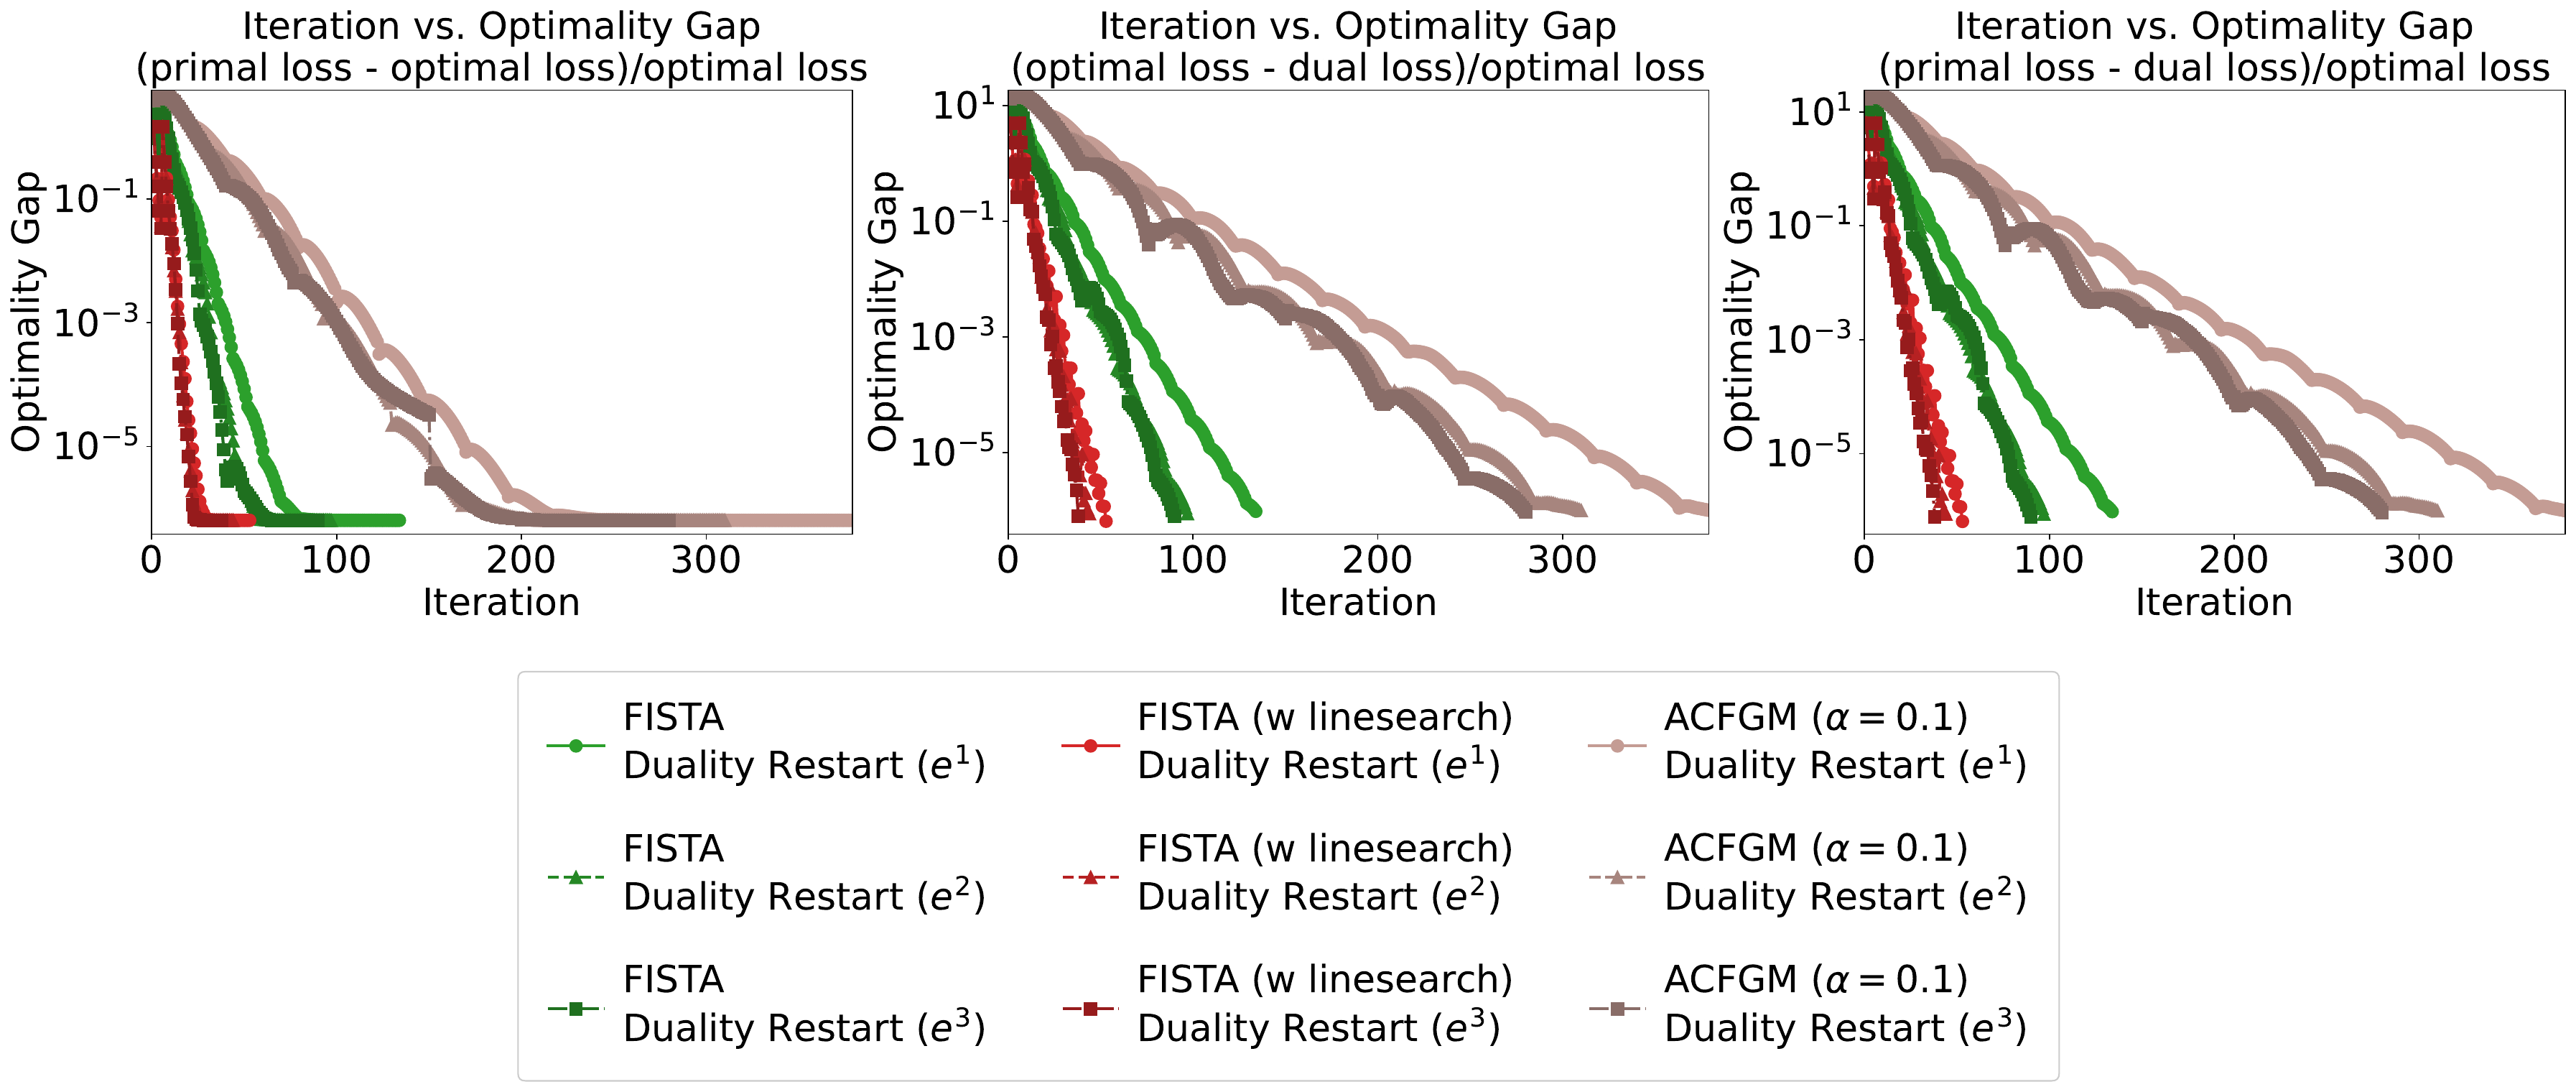}
    \caption{Convergence speed comparison of FISTA methods (with and without line search) and ACFGM (with duality-gap-based restarted ) for $\eta=e$, $\eta=e^2$, and $\eta=e^3$ on solving the perspective relaxation in Problem~\ref{obj:perspective_relaxation} with the linear regression loss, $n= 16000$, $p= 16000$, $k= 10$, $\rho= 0.5$, $\lambda_2 = 1.0$, and $M = 2.0$.}
    \label{ec_fig:PDRestart_achieves_linear_convergence_rate_exponents_linear}
    \vspace{0em}
\end{figure}

\begin{figure}[!h]
    \vspace{0em}
    \centering
    \includegraphics[width=1.0\textwidth]{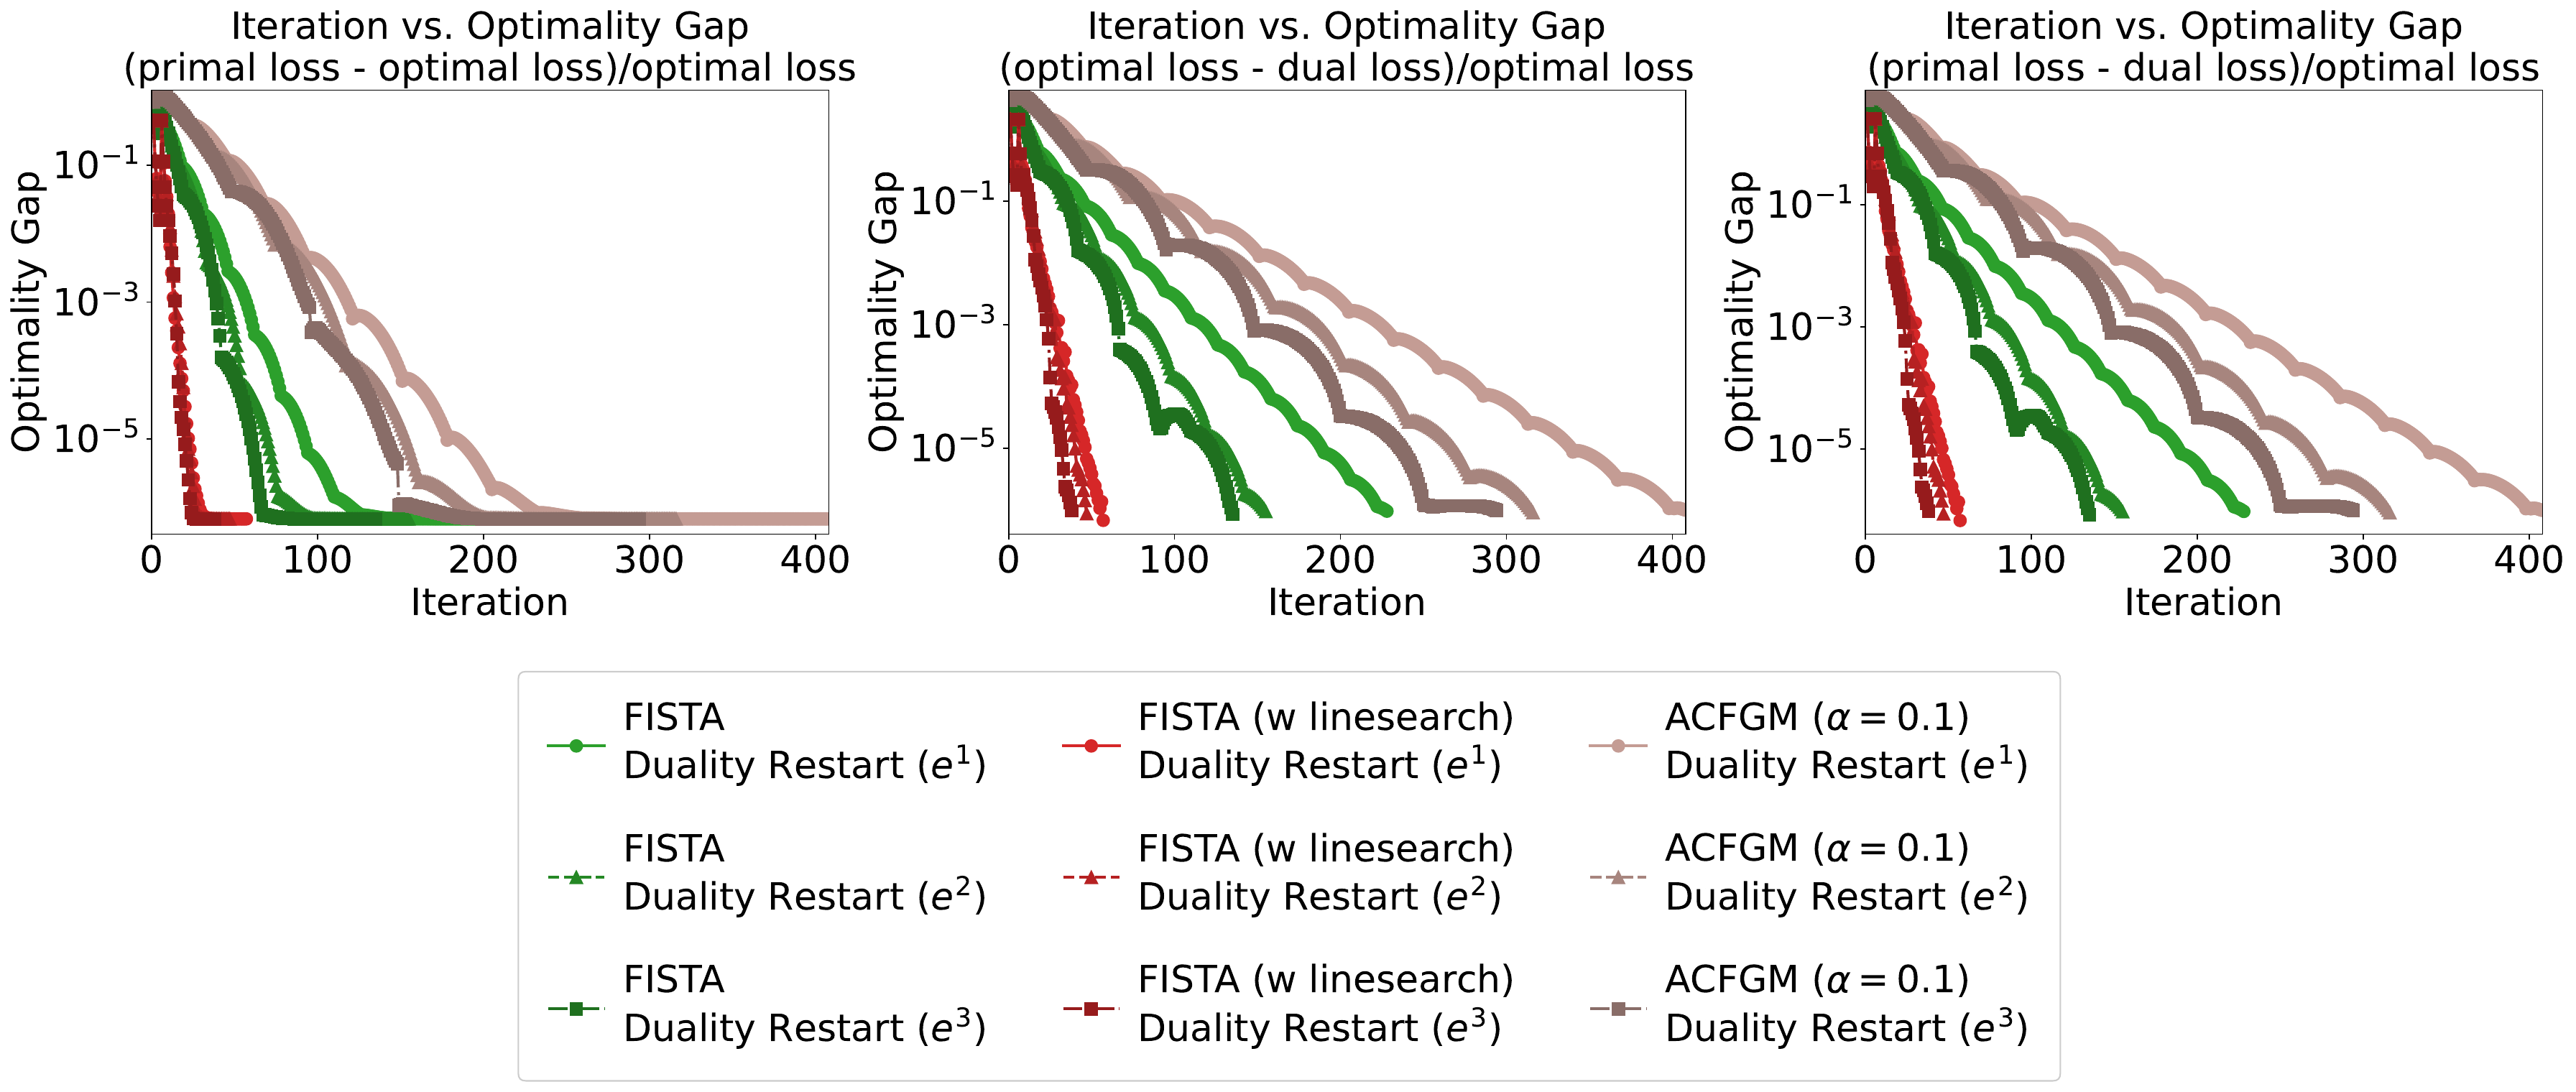}
    \caption{Convergence speed comparison of FISTA methods (with and without line search) and ACFGM (with duality-gap-based restarted ) for $\eta=e$, $\eta=e^2$, and $\eta=e^3$ on solving the perspective relaxation in Problem~\ref{obj:perspective_relaxation} with the logistic regression loss, $n= 16000$, $p= 16000$, $k= 10$, $\rho= 0.5$, $\lambda_2 = 1.0$, and $M = 2.0$.}
    \label{ec_fig:PDRestart_achieves_linear_convergence_rate_exponents_logistic}
\end{figure}

\clearpage
\subsection{Can Our Restart Scheme Benefit Other Problems Beyond Perspective Relaxations?}
\label{ec_expt:restart_beyond_perspective_relaxations}
To demonstrate the broader applicability of our duality-gap-based restart scheme beyond perspective relaxations, we apply it to accelerate proximal gradient methods for solving LASSO problems.
We report results for both an $\ell_1$-ball constrained formulation, where $G(\bbeta) := \delta_{\lVert \bbeta \rVert_1 \leq C}(\bbeta)$, and an $\ell_1$-regularized formulation, where $G(\bbeta) := \lambda_1 \lVert \bbeta \rVert_1$.
See Appendix~\ref{ec_expt:setup_for_restart_generality_lasso} for the experimental setup and parameter choices.
The results are shown in Figure~\ref{ec_fig:l1_constrained_linear_convergence}--Figure~\ref{ec_fig:l1_regularized_logistic_convergence}.
Like in the main paper for solving the perspective relaxation, we observe that our restart scheme accelerates both FISTA and ACFGM to achieve linear convergence rates.

\begin{figure}[!h]
    \centering
    \includegraphics[width=1.0\textwidth]{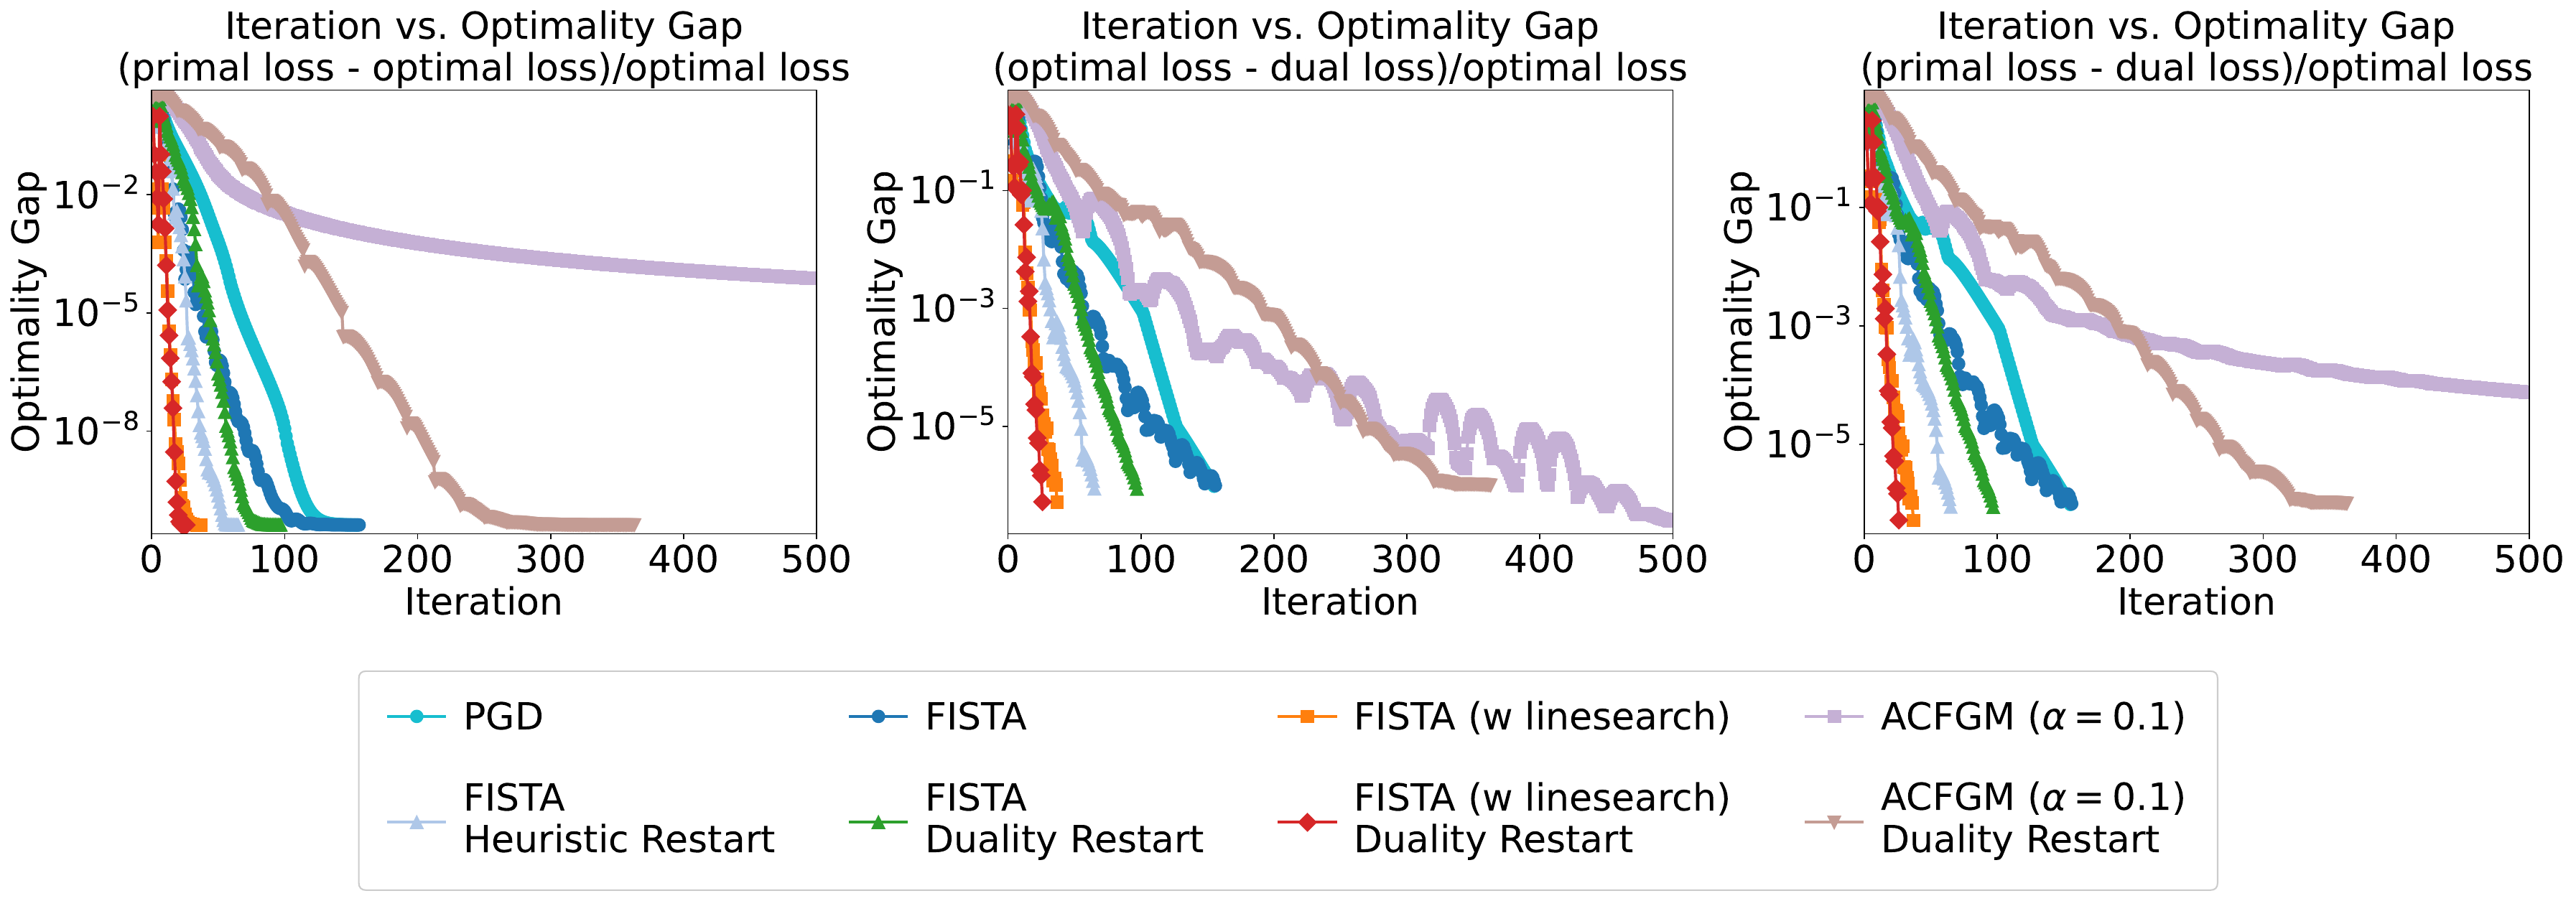}
    \caption{Convergence speed comparison between accelerated methods (with and without restart), on solving the $\ell_1$-ball constrained problem with the least squares loss.}
    \label{ec_fig:l1_constrained_linear_convergence}
    \vspace{0em}
\end{figure}

\begin{figure}[!h]
    \centering
    \includegraphics[width=1.0\textwidth]{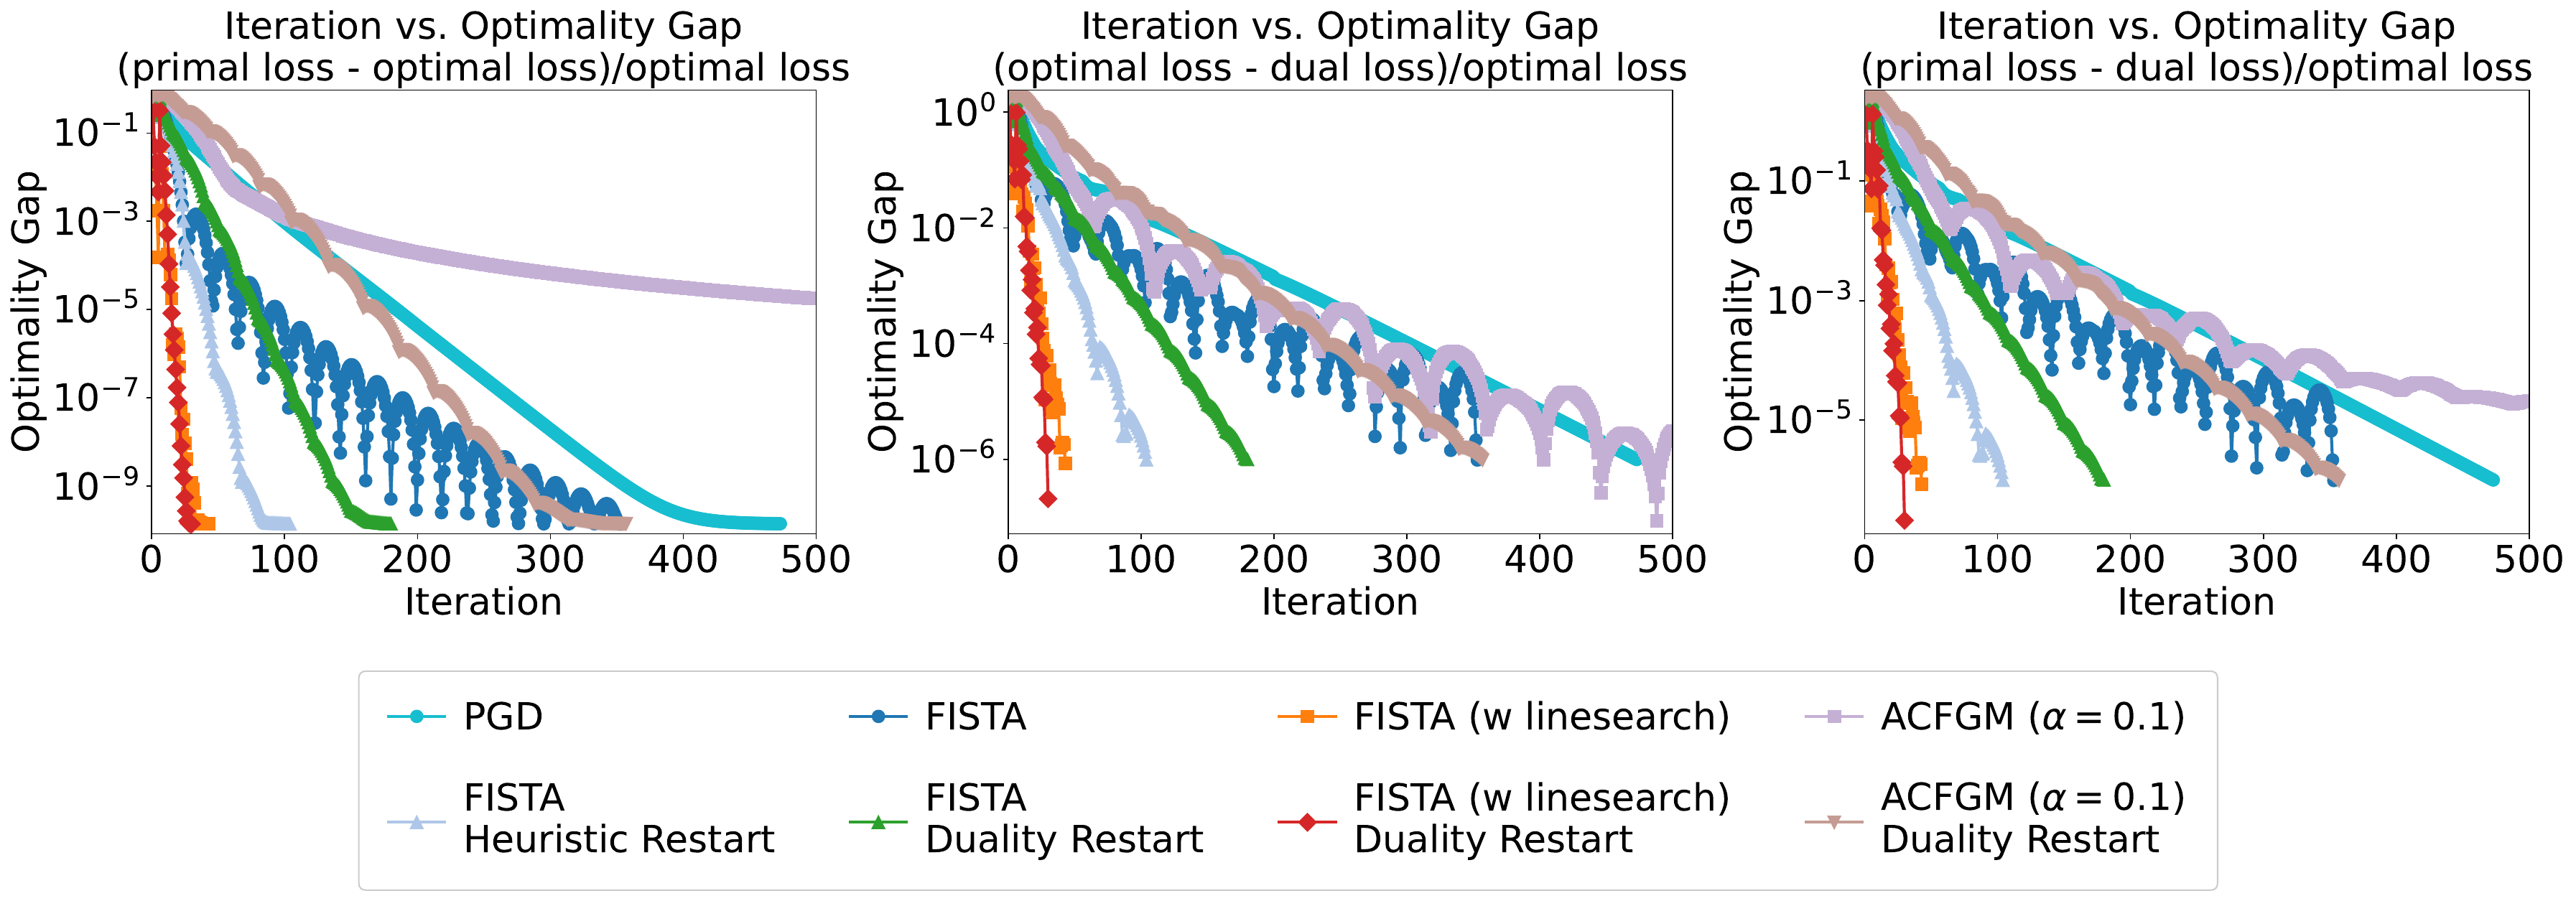}
    \caption{Convergence speed comparison between accelerated methods (with and without restart), on solving the $\ell_1$-ball constrained problem with the logistic regression loss.}
    \label{ec_fig:l1_constrained_logistic_convergence}
    \vspace{0em}
\end{figure}

\paragraph{Dual feasibility for $\ell_1$-regularized problems.}
For the $\ell_1$-regularized formulation, the Fenchel conjugate of the regularization term $G(\bbeta) = \lambda_1 \lVert \bbeta \rVert_1$ is $G^*(\bu) = \delta_{\lVert \bu \rVert_\infty \le \lambda_1}(\bu)$, and hence the dual objective is finite only when $\lVert \bX^\top \bzeta \rVert_\infty \le \lambda_1$.
Thus, the dual sequence $\bzeta^t := - \nabla F \left( \bX \bbeta^t \right)$ can be infeasible, in which case evaluating the dual objective is not meaningful.
Following standard practice in the LASSO literature, we enforce dual feasibility via a simple scaling (radial projection) step,
$\widehat{\bzeta} := \bzeta \cdot \min\!\left\{1,\ \frac{\lambda_1}{\lVert \bX^\top \bzeta \rVert_\infty}\right\}$,
which guarantees $\lVert \bX^\top \widehat{\bzeta} \rVert_\infty \le \lambda_1$ and yields a valid (though potentially loose) dual lower bound for computing a duality gap \citep{fercoq2015mind,dantas2021expanding}.
As a result, when applying our gap-based restart scheme to $\ell_1$-regularized problems, the gap used for restarting should be viewed as an inexact certificate; nevertheless, it still provides an effective restart signal in practice, leading to the linear-convergence behavior observed below.

\begin{figure}[!h]
    \centering
    \includegraphics[width=1.0\textwidth]{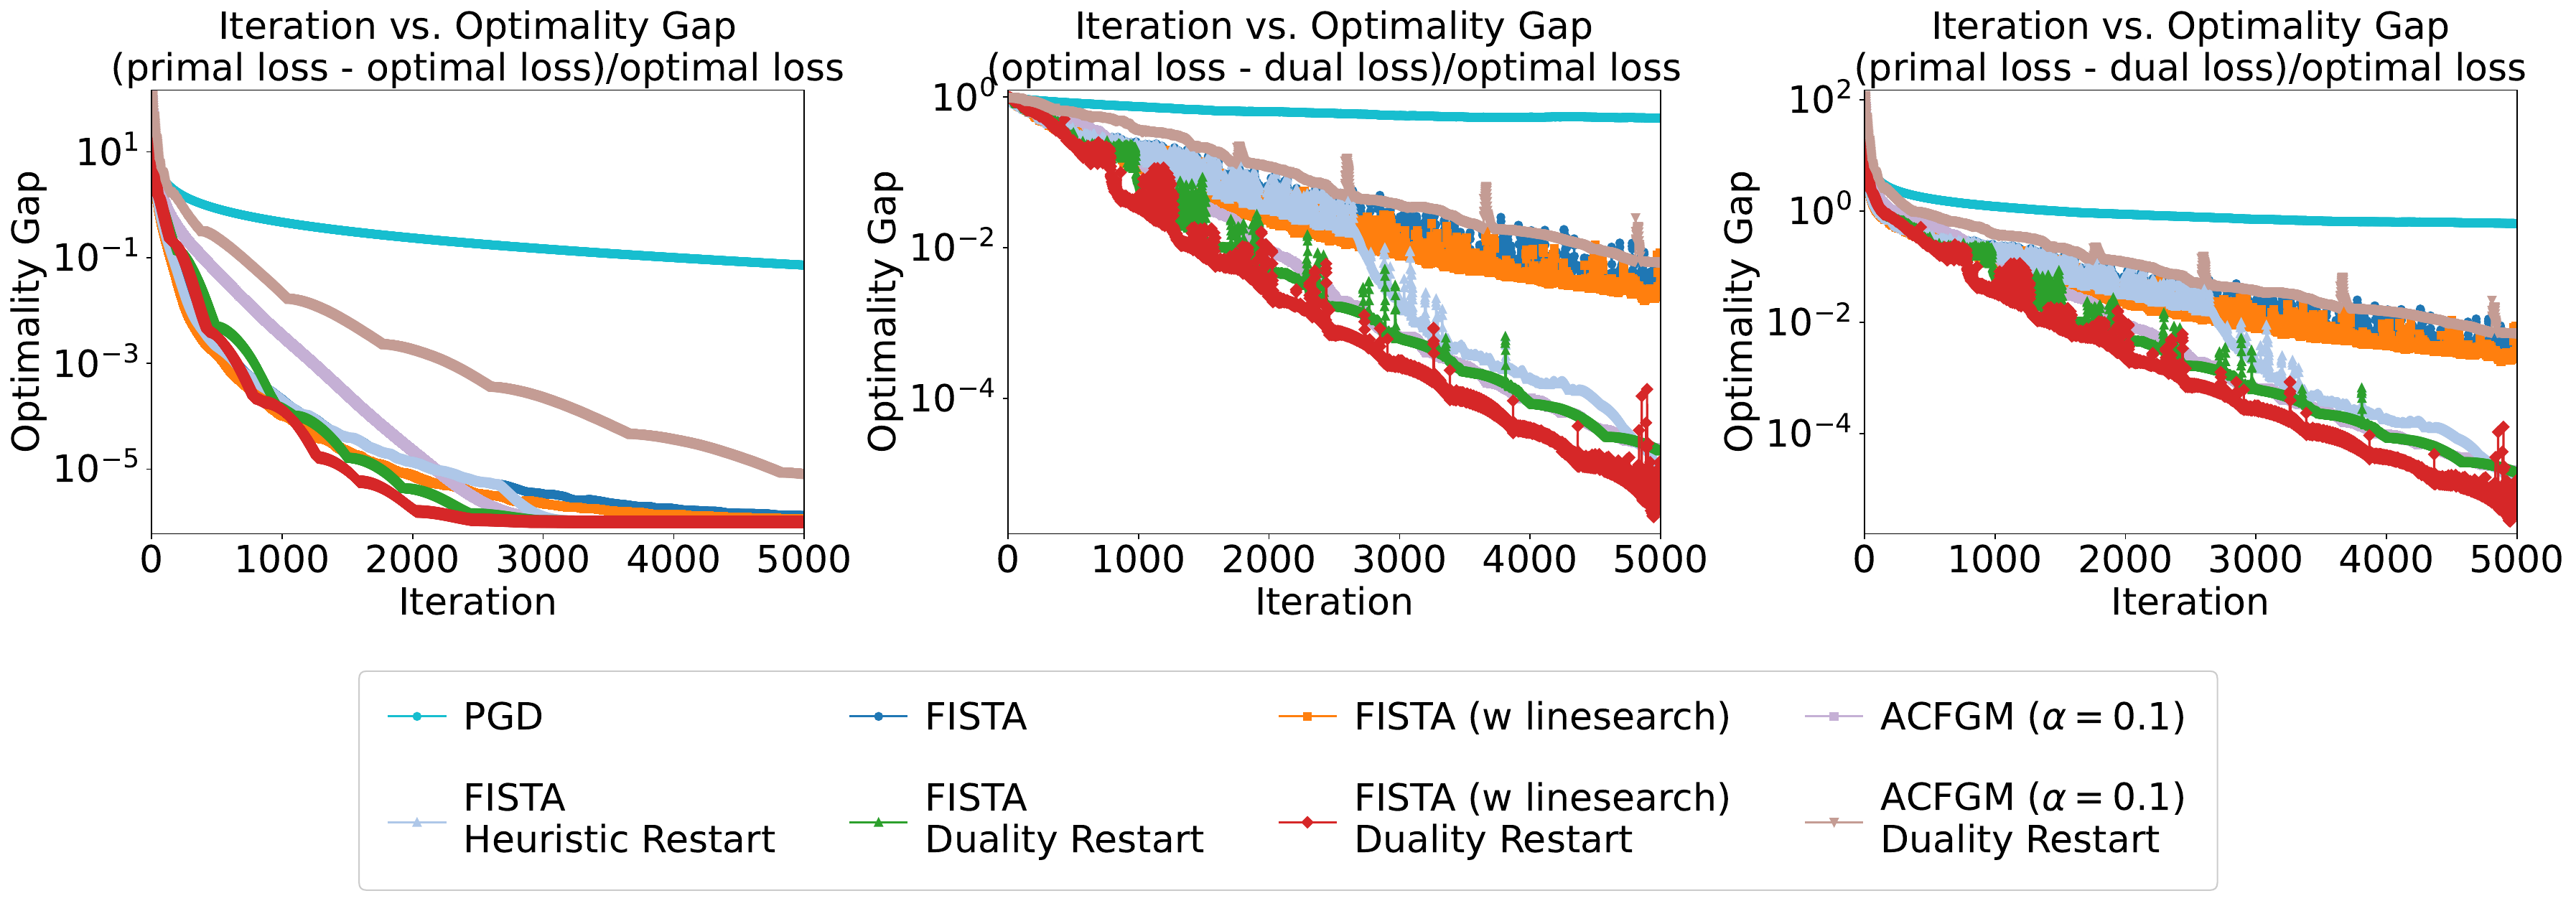}
    \caption{Convergence speed comparison between accelerated methods (with and without restart), on solving the $\ell_1$-regularized problem with the least squares loss.}
    \label{ec_fig:l1_regularized_linear_convergence}
    \vspace{0em}
\end{figure}

\begin{figure}[!h]
    \centering
    \includegraphics[width=1.0\textwidth]{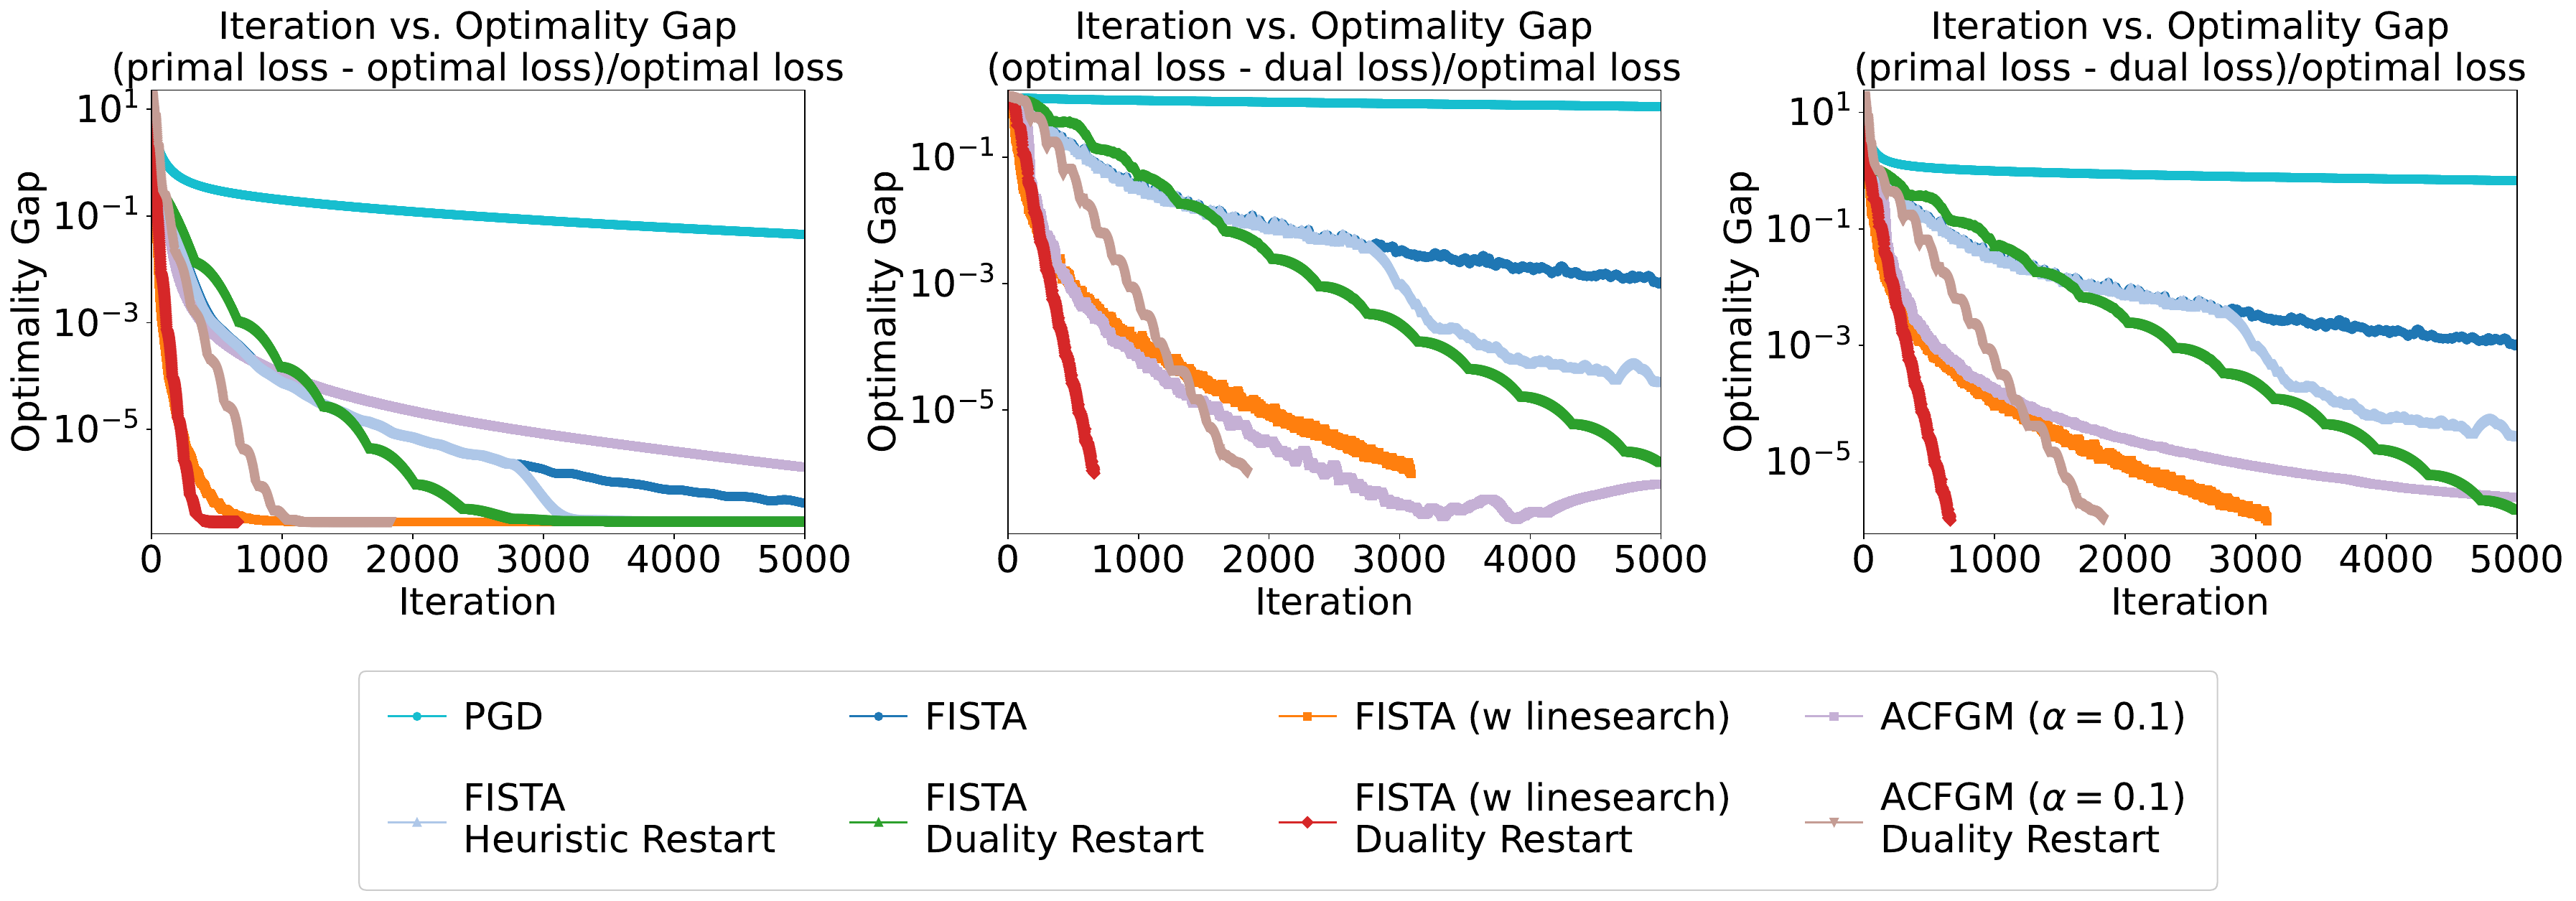}
    \caption{Convergence speed comparison between accelerated methods (with and without restart), on solving the $\ell_1$-regularized problem with the logistic regression loss.}
    \label{ec_fig:l1_regularized_logistic_convergence}
\end{figure}

\clearpage
\subsection{Certifying Optimality}
\label{ec_expt:additional_results_on_certifying_optimality}

\subsubsection{Synthetic Results with $M=3$}
We report additional branch-and-bound results on the synthetic datasets with a larger box constraint $M=3.0$: CPU baselines in Tables~\ref{tab:bnb_linear_M3}--\ref{tab:bnb_logistic_M3} and CPU vs GPU comparisons in Tables~\ref{tab:bnb_gpu_linear_M3}--\ref{tab:bnb_gpu_logistic_M3}.

% Branch-and-bound results for linear regression (M=3)
% Metadata: rows are p-values; columns grouped by method (ours, gurobi, mosek), each with time (0-decimal, TL shown for time>=7200 with LB in parentheses for ours), gap (\% to two decimals; any nonzero gap <0.005 shown as 0.01), and \# nodes; no vertical rules (OPRE); trimmed horizontal rules under method headers; numeric entries rounded accordingly with "-" for unavailable; caption lists k, rho, lambda2, M, and n/p=1.0 (assumed); source is sections/Tables/raw_txt/011825/plots_BnB_synthetic/print_BnB_synthetic.txt for k=10, rho=0.5, lambda2=1.0, M=3.0; method mapping: ours = beamsize5+ourspdrestartedbeckfistalinesearche3; gurobi = gurobinativewarmstart; mosek = moseknativewarmstart; for ours, time shows total time with LB time in parentheses; display names omit "w/ warmstart" while values are from warmstarted baselines; caption notes OOM and TL=7200s when present.
\begin{table}[!ht]
\vspace{0em}
\centering
\caption{BnB results on synthetic (linear) with $k=10$, $\rho=0.5$, $\lambda_2=1.0$, $M=3.0$, $n/p=1.0$. Parentheses show lower-bound time. OOM = out of memory, TL = time $> 7200$s.}
\label{tab:bnb_linear_M3}
\resizebox{1.0\linewidth}{!}{%
\begin{tabular}{rccc ccc ccc}
\hline
 & \multicolumn{3}{c}{ours} & \multicolumn{3}{c}{gurobi} & \multicolumn{3}{c}{mosek} \\
\cmidrule(l{0.8em}r{0.8em}){2-4}\cmidrule(l{0.8em}r{0.8em}){5-7}\cmidrule(l{0.8em}r{0.8em}){8-10}
$p$ & time(s) & gap(\%) & \# nodes & time(s) & gap(\%) & \# nodes & time(s) & gap(\%) & \# nodes \\ \hline
1000 & 31 (3) & 0.00 & 355 & 227 & 0.00 & 653 & 208 & 0.00 & 361 \\
2000 & 16 (2) & 0.00 & 161 & 2091 & 0.00 & 1544 & 758 & 0.00 & 171 \\
4000 & 27 (15) & 0.00 & 77 & 4574 & 0.00 & 97 & 3612 & 0.00 & 73 \\
8000 & 63 (45) & 0.00 & 49 & TL & 100.00 & 1 & TL & 33.57 & 4 \\
16000 & 151 (115) & 0.00 & 33 & TL & 100.00 & 1 & OOM & OOM & OOM \\
\hline
\end{tabular}%
}
\vspace{0em}
\end{table}

% Branch-and-bound results for logistic regression (M=3)
% Metadata: rows are p-values; columns grouped by method (ours, gurobiOA, mosek), each with time (0-decimal, TL shown for time>=7200 with LB in parentheses for ours), gap (\% to two decimals; any nonzero gap <0.005 shown as 0.01), and \# nodes; no vertical rules (OPRE); trimmed horizontal rules under method headers; numeric entries rounded accordingly with "-" for unavailable; caption lists k, rho, lambda2, M, and n/p=1.0 (assumed); source is sections/Tables/raw_txt/011825/plots_BnB_synthetic/print_BnB_synthetic.txt for k=10, rho=0.5, lambda2=1.0, M=3.0; method mapping: ours = beamsize5+ourspdrestartedbeckfistalinesearche3; gurobiOA = gurobinativeoawarmstart; mosek = moseknativewarmstart; for ours, time shows total time with LB time in parentheses; display names omit "w/ warmstart" while values are from warmstarted baselines; caption notes OOM and TL=7200s when present.
\begin{table}[!ht]
\vspace{0em}
\centering
\caption{BnB results on synthetic (logistic) with $k=10$, $\rho=0.5$, $\lambda_2=1.0$, $M=3.0$, $n/p=1.0$. Parentheses show lower-bound time. OOM = out of memory, TL = time $> 7200$s.}
\label{tab:bnb_logistic_M3}
\resizebox{1.0\linewidth}{!}{%
\begin{tabular}{rccc ccc ccc}
\hline
 & \multicolumn{3}{c}{ours} & \multicolumn{3}{c}{gurobiOA} & \multicolumn{3}{c}{mosek} \\
\cmidrule(l{0.8em}r{0.8em}){2-4}\cmidrule(l{0.8em}r{0.8em}){5-7}\cmidrule(l{0.8em}r{0.8em}){8-10}
$p$ & time(s) & gap(\%) & \# nodes & time(s) & gap(\%) & \# nodes & time(s) & gap(\%) & \# nodes \\ \hline
1000 & 771 (37) & 0.00 & 6049 & TL & 67.29 & 417432 & 1871 & 0.00 & 5847 \\
2000 & 630 (81) & 0.00 & 3451 & TL & 87.29 & 443958 & 7031 & 0.00 & 3427 \\
4000 & 384 (168) & 0.00 & 855 & TL & 82.12 & 269137 & TL & 13.97 & 569 \\
8000 & 666 (404) & 0.00 & 459 & TL & 69.86 & 93806 & OOM & OOM & OOM \\
16000 & 1031 (677) & 0.00 & 207 & TL & 56.55 & 35414 & OOM & OOM & OOM \\
\hline
\end{tabular}%
}
\vspace{0em}
\end{table}

% BnB GPU vs CPU results for linear regression (M=3)
% Metadata: rows are p-values; columns grouped by method (ours CPU, ours GPU), each with time (0-decimal, TL shown for time>=7200 with LB time in parentheses), gap (% to two decimals; any nonzero gap <0.005 shown as 0.01), and # nodes; no vertical rules (OPRE); trimmed horizontal rules under method headers; numeric entries rounded accordingly with "-" for unavailable; caption lists k, rho, lambda2, M, and n/p=1.0 (assumed); source is sections/Tables/raw_txt/011825/plots_BnB_synthetic_GPU/print_BnB_synthetic_GPU.txt for k=10, rho=0.5, lambda2=1.0, M=3.0; method mapping: ours CPU = beamsize5+ourspdrestartedbeckfistalinesearche3, ours GPU = beamsize5+oursgpupdrestartedbeckfistalinesearche3.
\begin{table}[!ht]
\centering
\caption{BnB CPU vs GPU results for linear regression with $k=10$, $\rho=0.5$, $\lambda_2=1.0$, $M=3.0$, $n/p=1.0$. Parentheses show lower-bound time.}
\label{tab:bnb_gpu_linear_M3}
\resizebox{0.7\linewidth}{!}{%
\begin{tabular}{rccc ccc}
\hline
 & \multicolumn{3}{c}{ours CPU} & \multicolumn{3}{c}{ours GPU} \\
\cmidrule(l{0.8em}r{0.8em}){2-4}\cmidrule(l{0.8em}r{0.8em}){5-7}
$p$ & time(s) & gap(\%) & \# nodes & time(s) & gap(\%) & \# nodes \\ \hline
1000 & 29 (2) & 0.00 & 355 & 36 (9) & 0.00 & 355 \\
2000 & 15 (2) & 0.00 & 161 & 18 (4) & 0.00 & 161 \\
4000 & 12 (4) & 0.00 & 77 & 9 (2) & 0.00 & 77 \\
8000 & 44 (30) & 0.00 & 49 & 15 (2) & 0.00 & 49 \\
16000 & 78 (53) & 0.00 & 33 & 26 (4) & 0.00 & 33 \\
\hline
\end{tabular}%
}
\end{table}

% BnB GPU vs CPU results for logistic regression (M=3)
% Metadata: rows are p-values; columns grouped by method (ours CPU, ours GPU), each with time (0-decimal, TL shown for time>=7200 with LB time in parentheses), gap (% to two decimals; any nonzero gap <0.005 shown as 0.01), and # nodes; no vertical rules (OPRE); trimmed horizontal rules under method headers; numeric entries rounded accordingly with "-" for unavailable; caption lists k, rho, lambda2, M, and n/p=1.0 (assumed); source is sections/Tables/raw_txt/011825/plots_BnB_synthetic_GPU/print_BnB_synthetic_GPU.txt for k=10, rho=0.5, lambda2=1.0, M=3.0; method mapping: ours CPU = beamsize5+ourspdrestartedbeckfistalinesearche3, ours GPU = beamsize5+oursgpupdrestartedbeckfistalinesearche3.
\begin{table}[!ht]
\centering
\caption{BnB CPU vs GPU results for logistic regression with $k=10$, $\rho=0.5$, $\lambda_2=1.0$, $M=3.0$, $n/p=1.0$. Parentheses show lower-bound time.}
\label{tab:bnb_gpu_logistic_M3}
\resizebox{0.7\linewidth}{!}{%
\begin{tabular}{rccc ccc}
\hline
 & \multicolumn{3}{c}{ours CPU} & \multicolumn{3}{c}{ours GPU} \\
\cmidrule(l{0.8em}r{0.8em}){2-4}\cmidrule(l{0.8em}r{0.8em}){5-7}
$p$ & time(s) & gap(\%) & \# nodes & time(s) & gap(\%) & \# nodes \\ \hline
1000 & 689 (38) & 0.00 & 6049 & 758 (108) & 0.00 & 6049 \\
2000 & 536 (39) & 0.00 & 3451 & 556 (65) & 0.00 & 3451 \\
4000 & 251 (62) & 0.00 & 855 & 203 (21) & 0.00 & 855 \\
8000 & 412 (176) & 0.00 & 459 & 246 (18) & 0.00 & 459 \\
16000 & 533 (276) & 0.00 & 207 & 282 (23) & 0.00 & 207 \\
\hline
\end{tabular}%
}
\end{table}

% \clearpage
\subsubsection{Cross Validation to Select $\lambda_2$, $k$, and $M$ for Real-world Datasets}
\label{ec_expt:cv_select_lambda2_k_M_realworld}

To select the hyperparameters $(\lambda_2,k,M)$ for the real-world datasets, we conduct a 5-fold cross-validation study.
For both SantanderBank and DOROTHEA, we evaluate $\lambda_2 \in \{0.01, 0.1, 1.0, 2.0, 3.0, 10.0\}$ and $k \in \{2,3,\ldots,30\}$; during this grid-search step, we fix $M=100$ so that the box constraint is effectively inactive and does not influence model selection. For each $(\lambda_2,k)$ pair, we compute a heuristic solution on each training fold using the beamsearch method of~\citet{liu2024okridge} and report performance on both training and validation folds (squared error for linear regression; log-loss, accuracy, and AUC for logistic regression) as a function of $\lambda_2$ and $k$; see Figure~\ref{ec_fig:beamsearch_cv_santander_lambda2_grid} (SantanderBank) and Figures~\ref{ec_fig:beamsearch_cv_dorothea_lambda2_0p01_0p1}--\ref{ec_fig:beamsearch_cv_dorothea_lambda2_3_10} (DOROTHEA). Based on these results, we select $(\lambda_2,k)=(1.0,10)$ for SantanderBank and $(\lambda_2,k)=(1.0,6)$ for DOROTHEA; under these settings, the maximum absolute coefficient values in the beamsearch solutions are $4.96$ and $4.95$, respectively, so we set $M=10.0$ in the experiments to ensure the box constraint does not affect solution quality.

\clearpage
\begin{figure}[!h]
    \centering
    \includegraphics[width=1.0\textwidth]{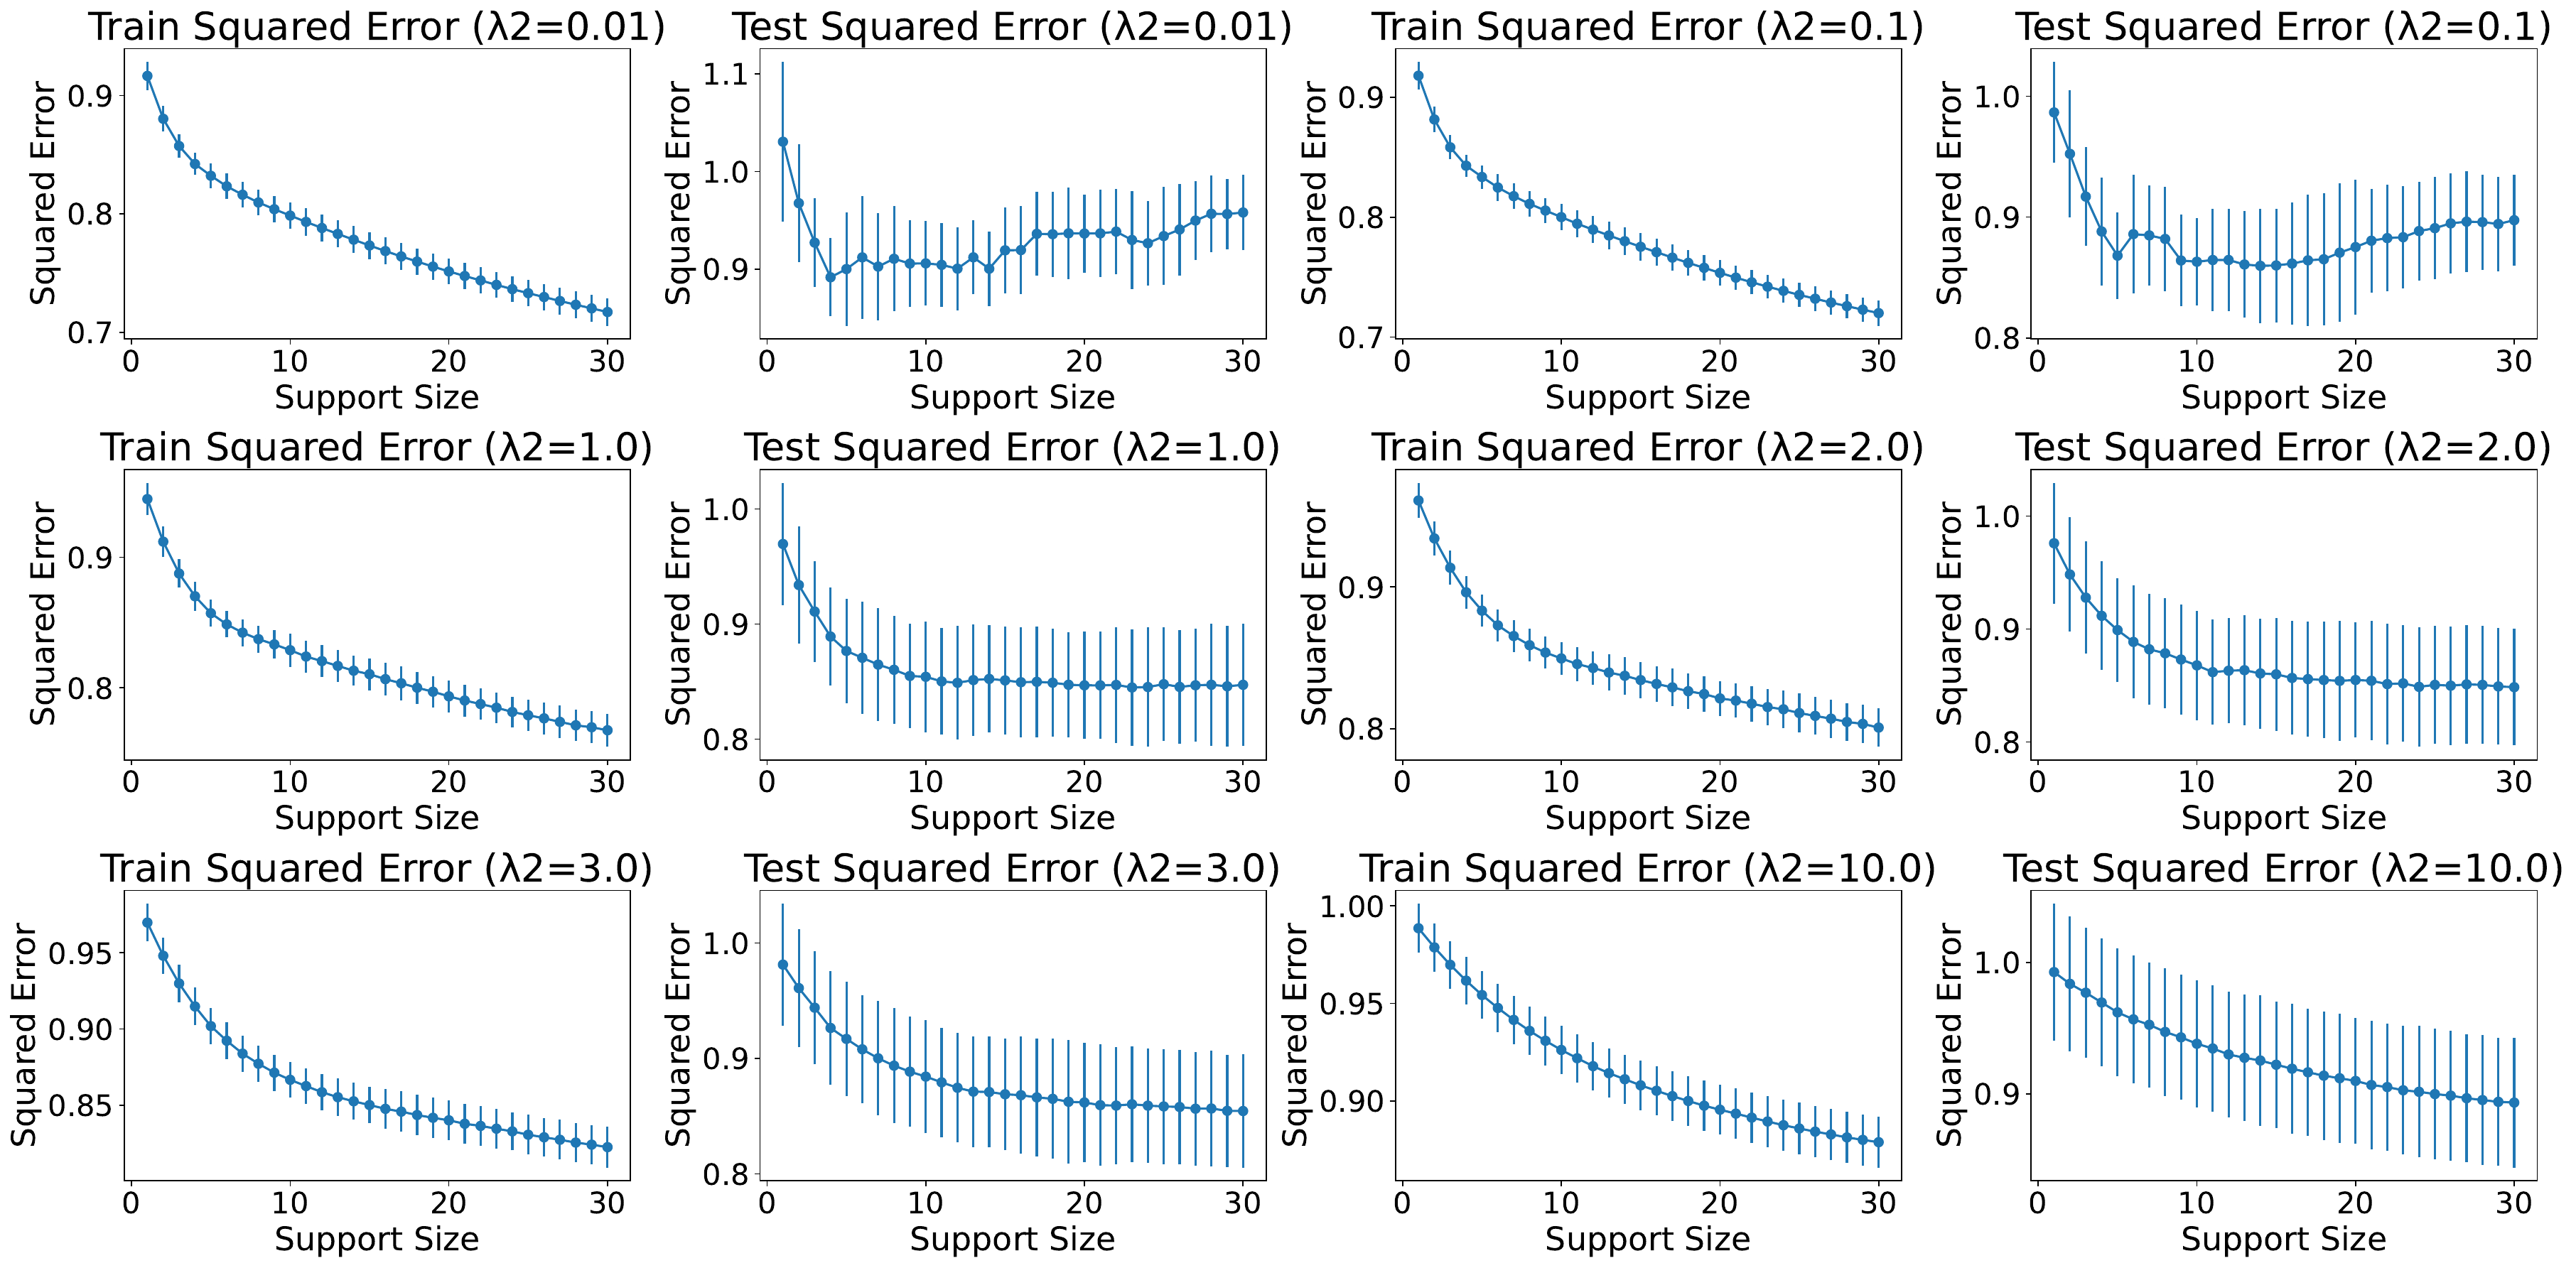}
    \caption{Beamsearch cross-validation results on the SantanderBank dataset with $\lambda_2 \in \{0.01, 0.1, 1.0, 2.0, 3.0, 10.0\}$.}
    \label{ec_fig:beamsearch_cv_santander_lambda2_grid}
    \vspace{0em}
\end{figure}

\begin{figure}[!h]
    \centering
    \includegraphics[width=1.0\textwidth]{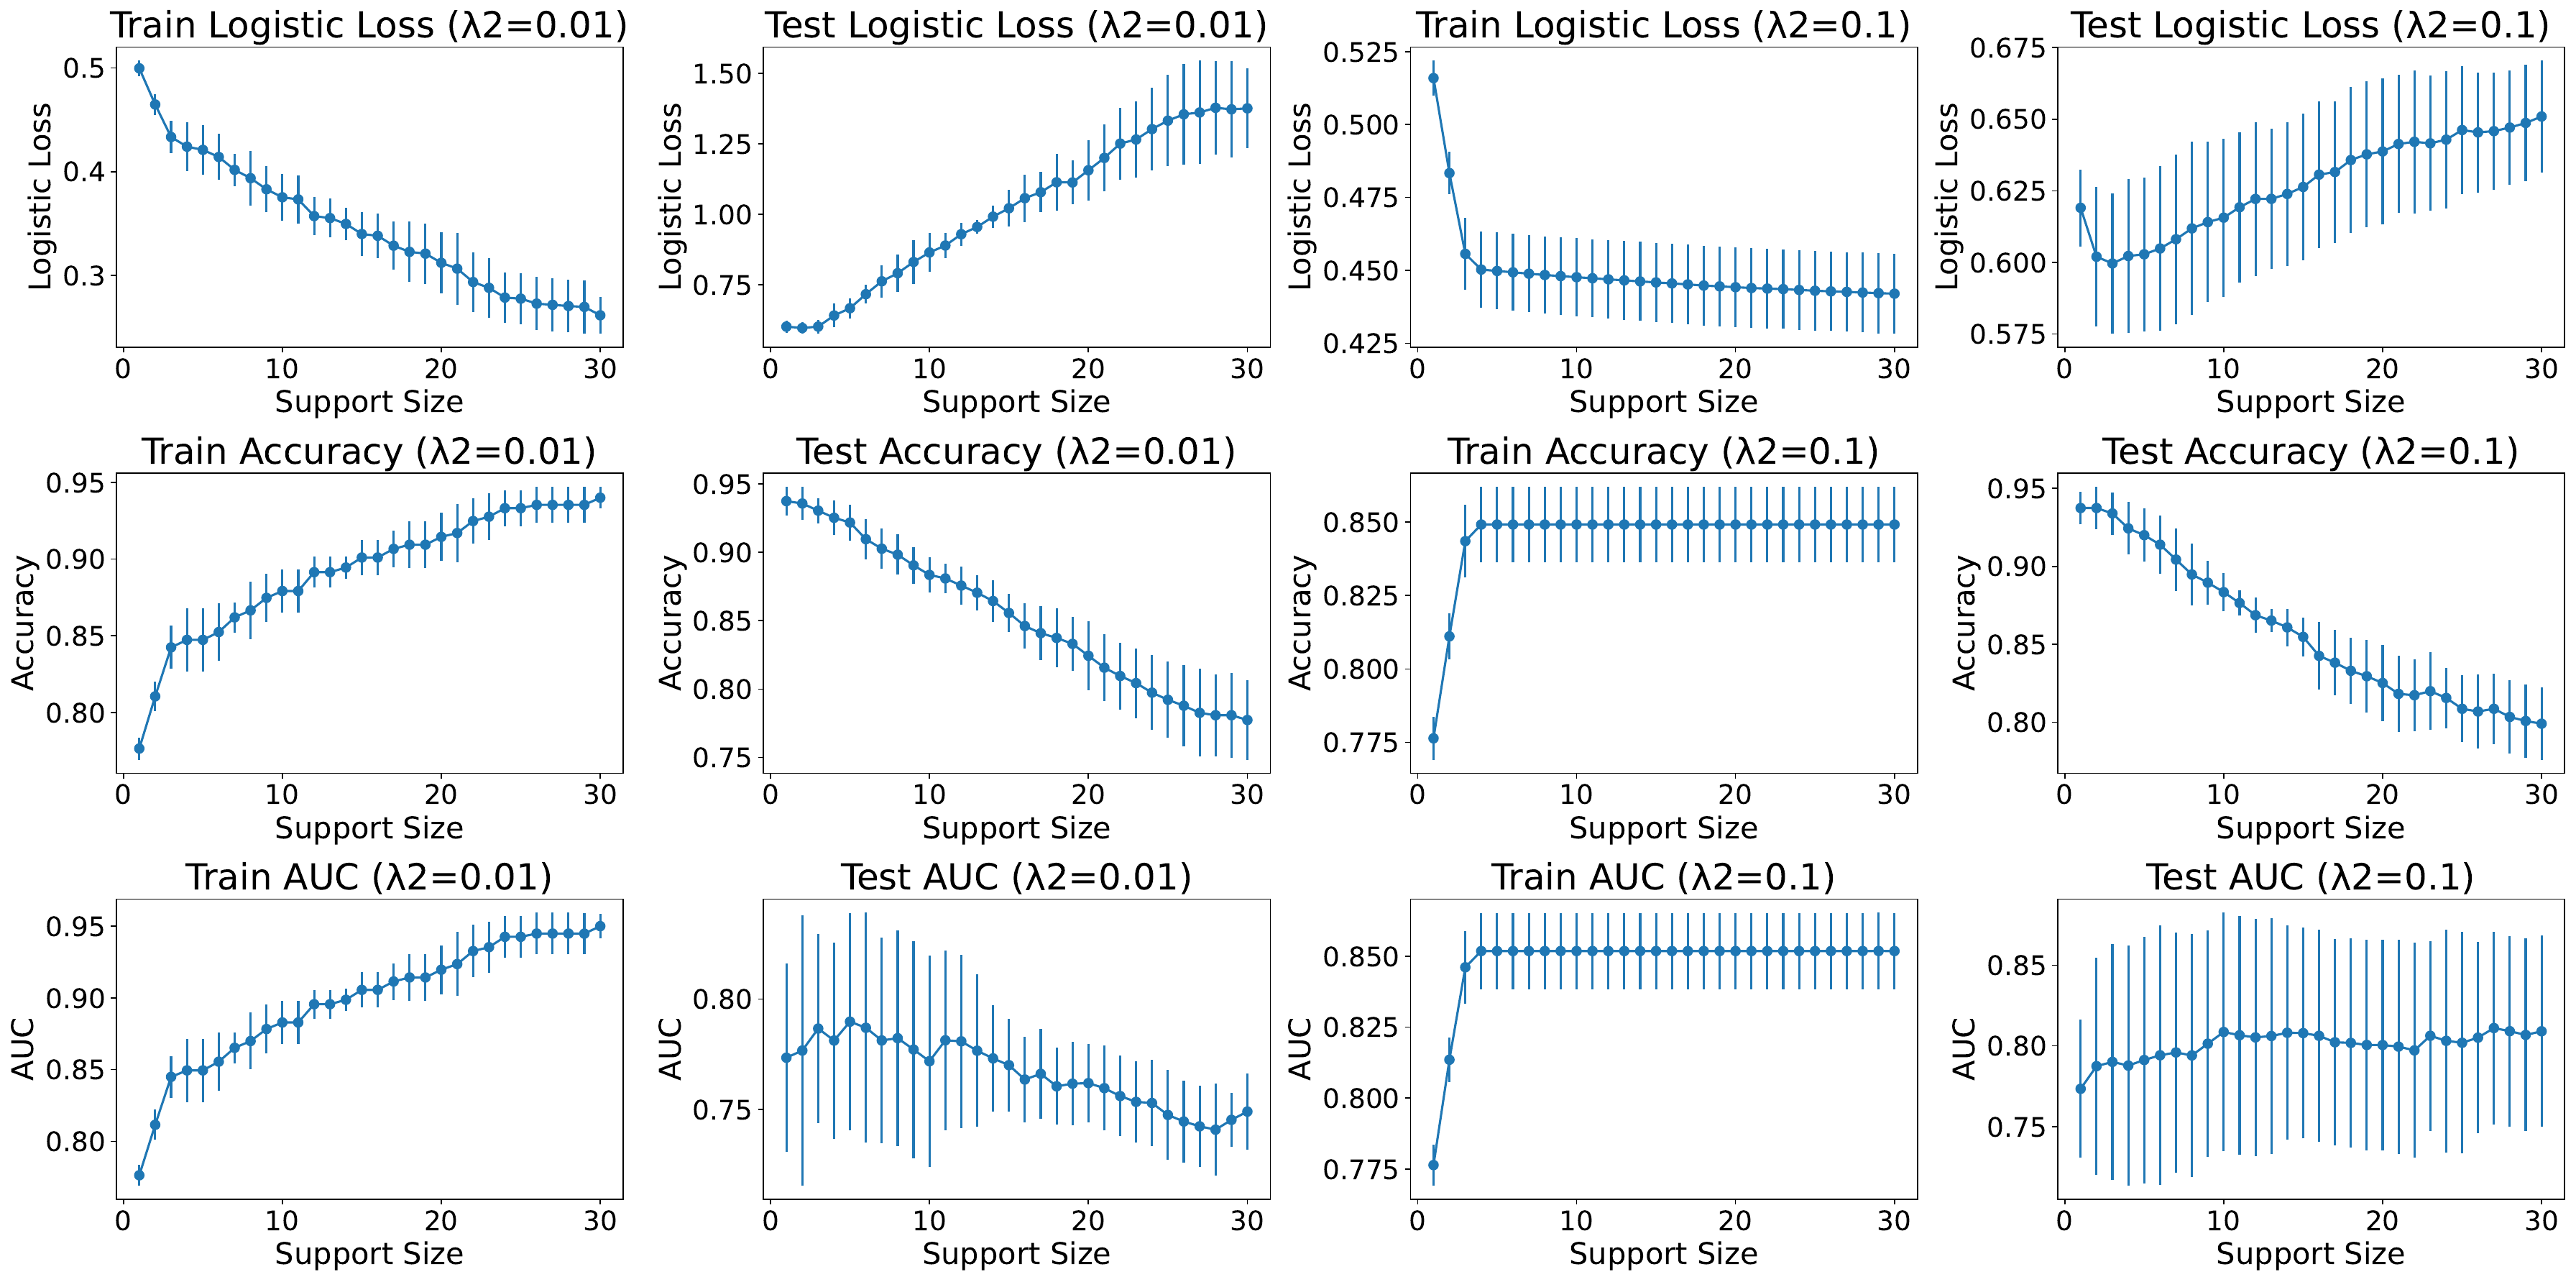}
    \caption{Beamsearch cross-validation results on the DOROTHEA dataset with $\lambda_2 \in \{0.01, 0.1\}$.}
    \label{ec_fig:beamsearch_cv_dorothea_lambda2_0p01_0p1}
    \vspace{0em}
\end{figure}

\clearpage
\begin{figure}[!h]
    \centering
    \includegraphics[width=1.0\textwidth]{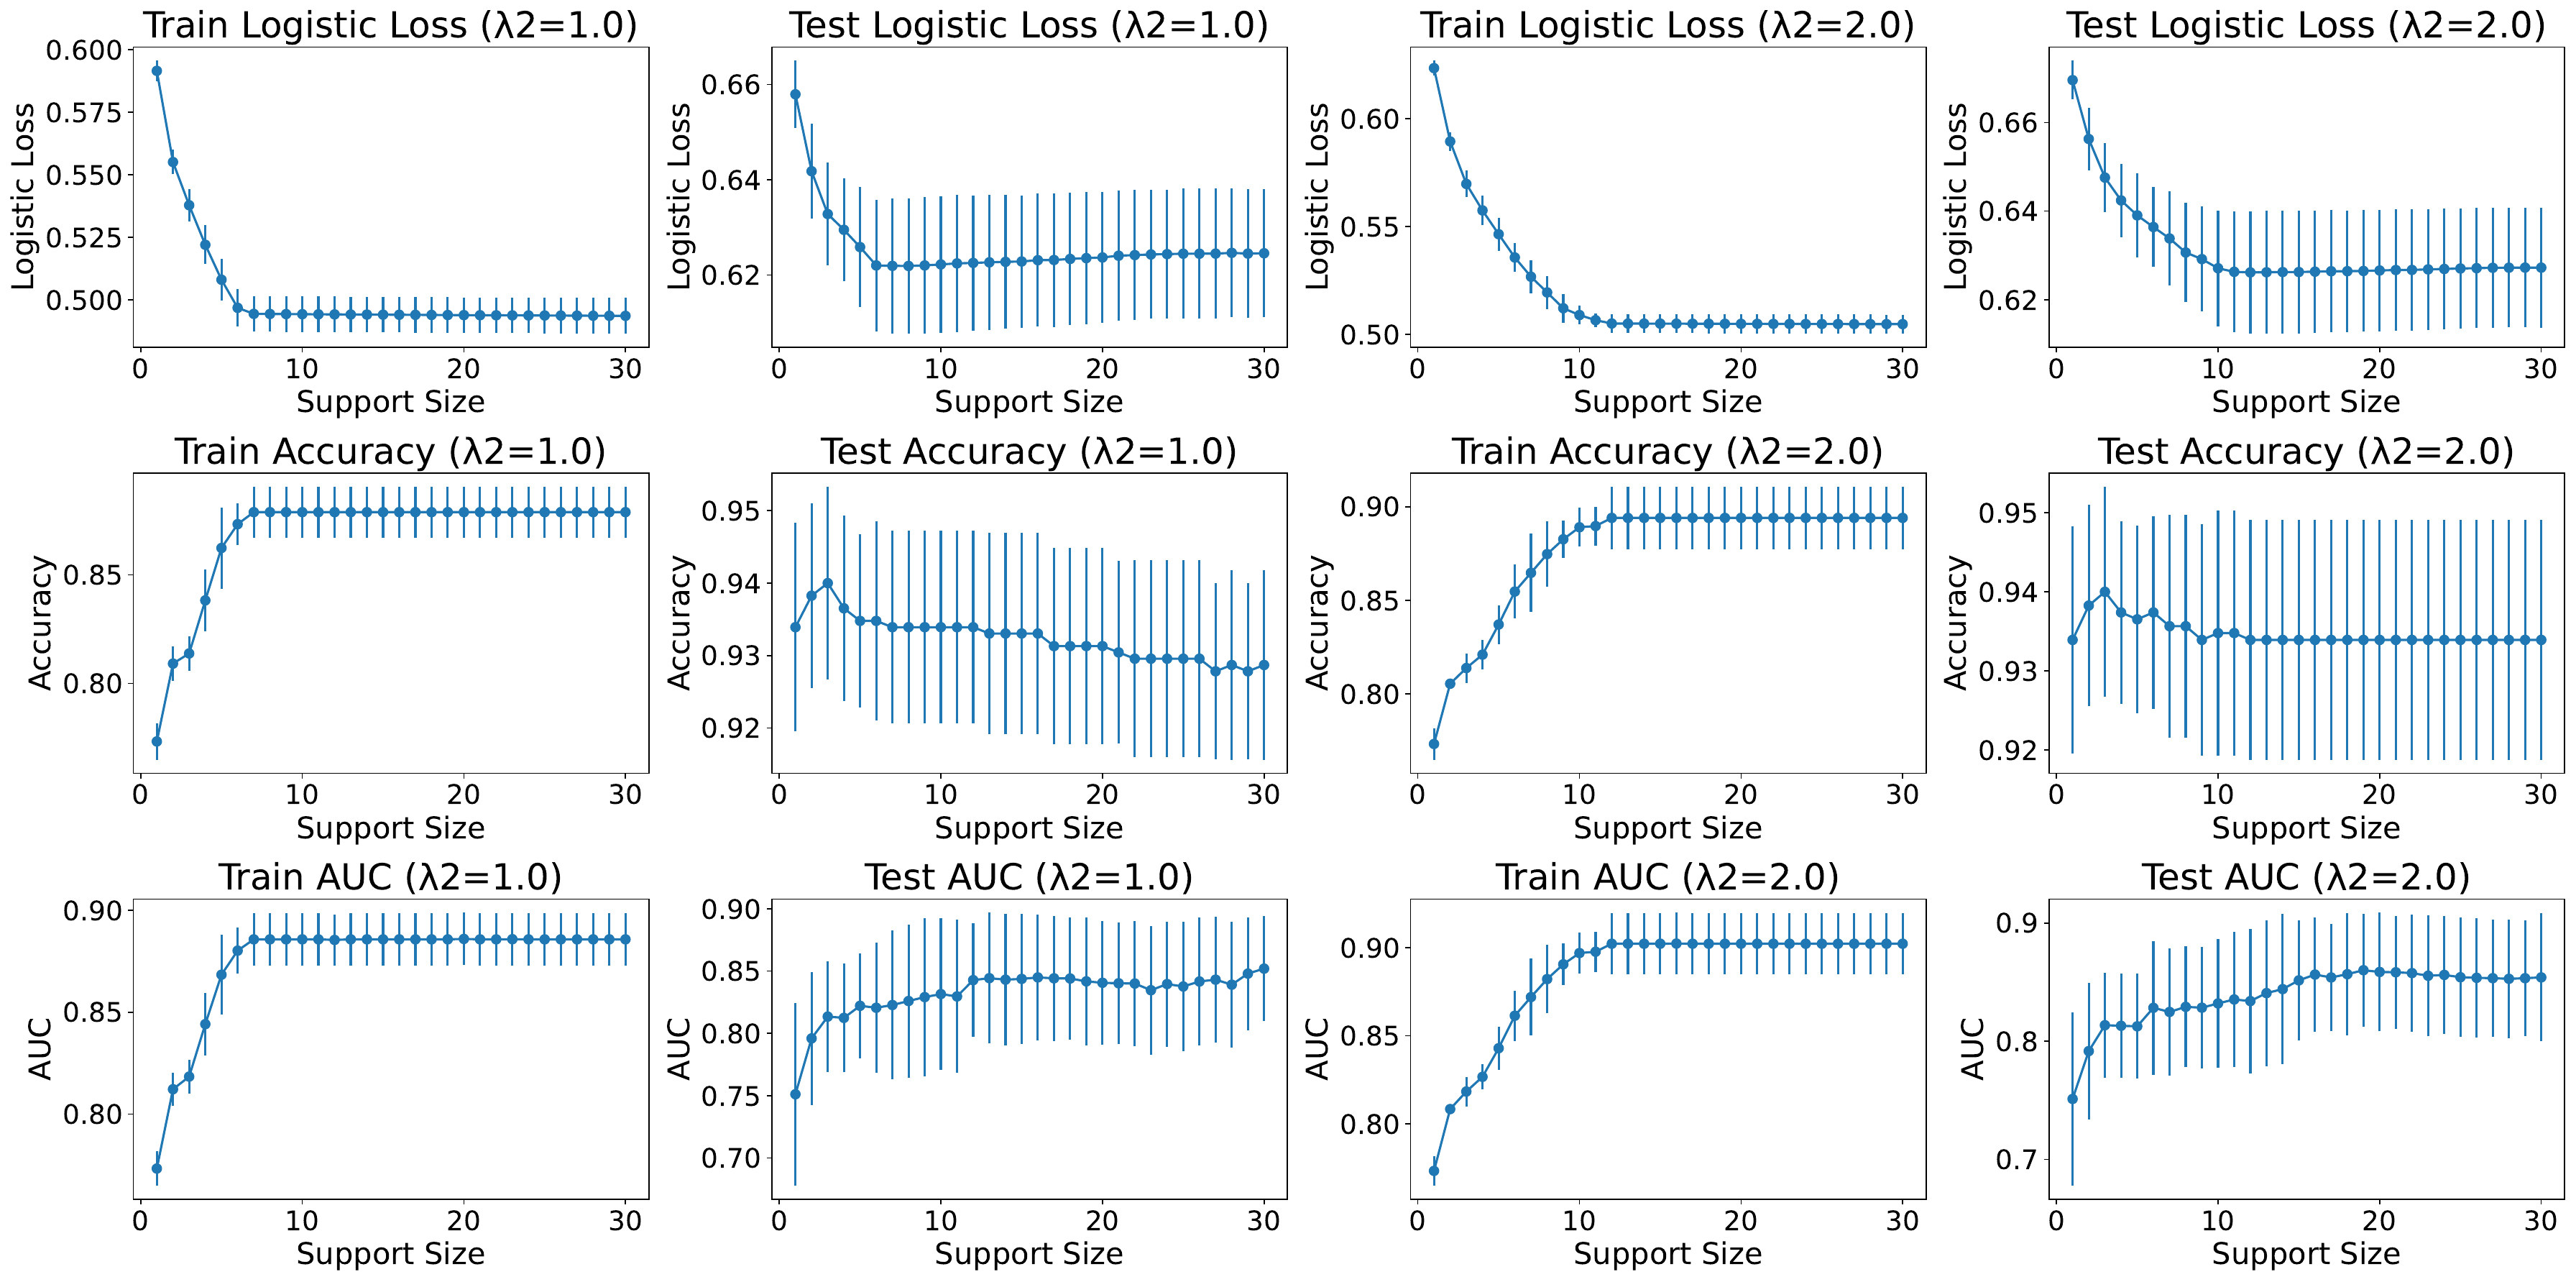}
    \caption{Beamsearch cross-validation results on the DOROTHEA dataset with $\lambda_2 \in \{1.0, 2.0\}$.}
    \label{ec_fig:beamsearch_cv_dorothea_lambda2_1_2}
    \vspace{0em}
\end{figure}

\begin{figure}[!h]
    \centering
    \includegraphics[width=1.0\textwidth]{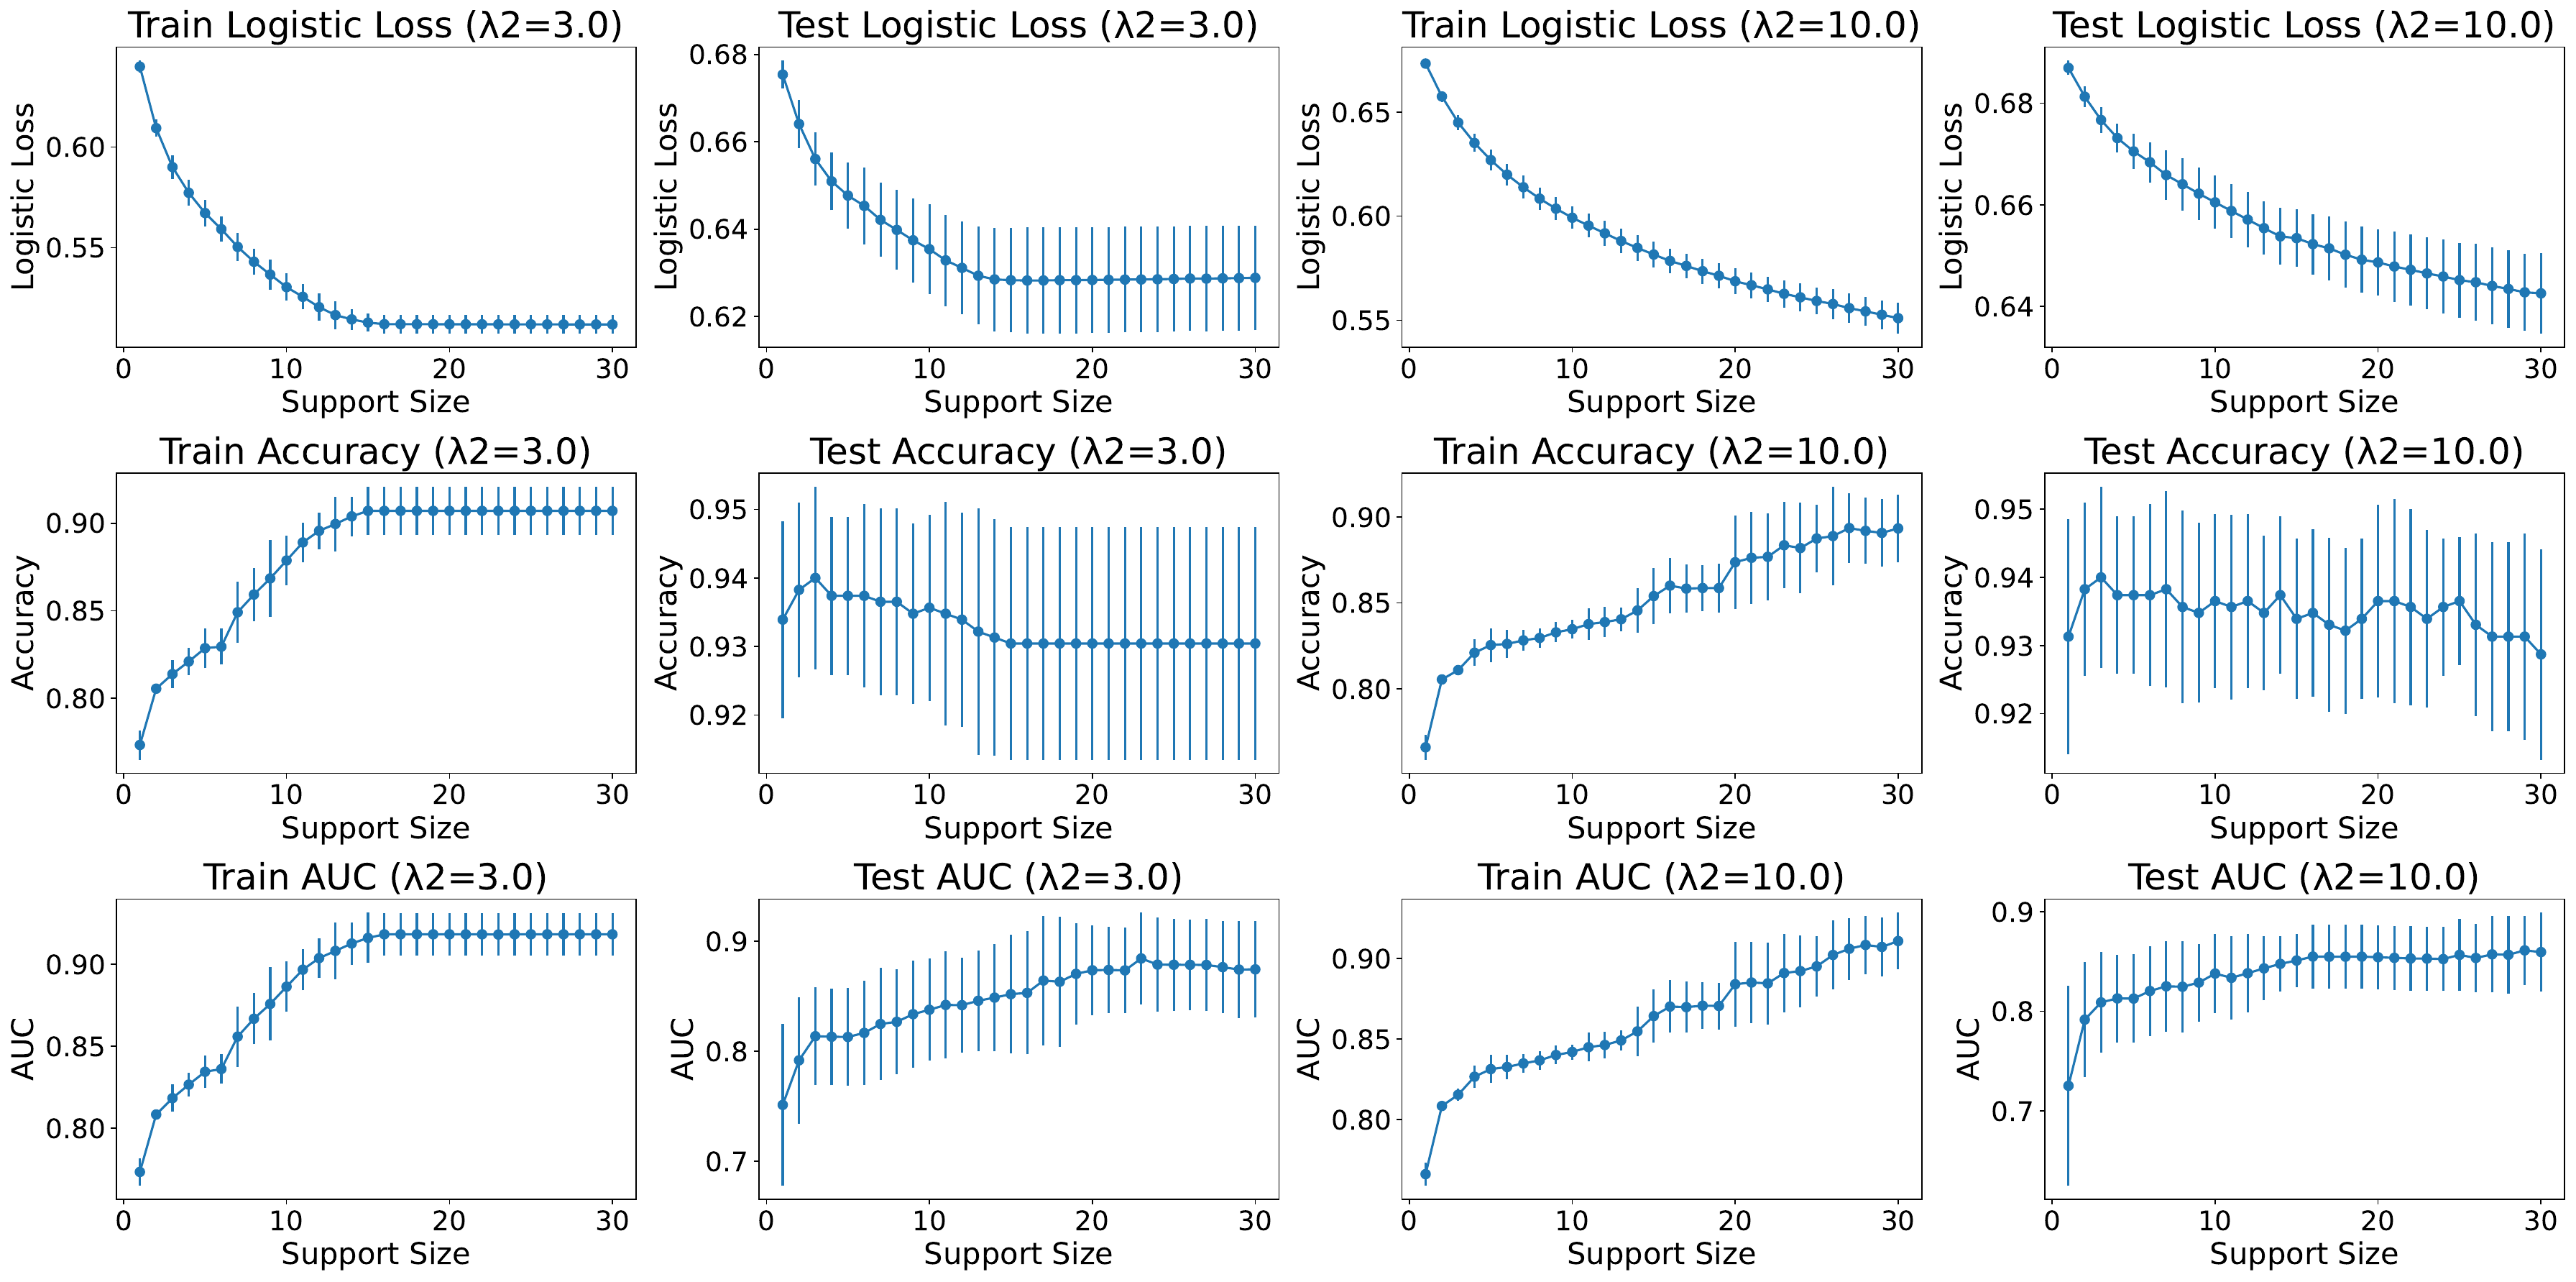}
    \caption{Beamsearch cross-validation results on the DOROTHEA dataset with $\lambda_2 \in \{3.0, 10.0\}$.}
    \label{ec_fig:beamsearch_cv_dorothea_lambda2_3_10}
\end{figure}
